# Supplementary material for: Generalized van Trees inequality: Local minimax bounds for non-smooth functionals and irregular statistical models
Source: arXiv:2405.06437 source file (2024-10-19)
Supplement: Supplementary file 1 [file chapman_robbin.tex]

\section{Proofs for Chapman-Robbins style van Trees Inequality}
\subsection{Proof of Theorem~\ref{thm:crvtBound}}
\kt{This proof is ready for review}
\begin{proof}[\bfseries{Proof of Theorem~\ref{thm:crvtBound}}]
An analogous proof is presented in \cite{pollard2014lecture}. We consider several modifications to the original proof such that i) the lower bound holds for a vector-valued functional $\psi := \Theta \mapsto \mathbb{R}^k$ and ii) the lower bound does not assume the differentiability of the functional or the regularity of statistical models. We first prove the statement for a real-valued functional $\psi : \Theta \mapsto \mathbb{R}$ and extend the result to vector-valued functionals. 

We consider a statistical model $\{P_\theta : \theta \in \Theta\}$ defined on a measurable space $(\mathcal{X}, \mathcal{A})$, indexed by a parameter space $\Theta$. We assume that $\Theta$ belongs to a complete normed space (i.e., Banach space) with a norm $\|\cdot\|_\Theta$, allowing $\Theta$ to be possibly infinite dimensional. We assume that each $P_\theta$ is absolutely continuous with respect to a dominating $\sigma$-finite measure $\mu$ and denote by $p_\theta = dP_\theta/d\mu$ the Radon-Nikodym derivative with respect to $\mu$. Similarly, we define a probability measure $Q$ supported on $\Theta$ and the density function $q$ with respect to a dominating $\sigma$-finite measure $\nu$. As a special case of $\Theta = \mathbb{R}^d$, the measure $\nu$ corresponds to the Lebesgue measure. A location family of $Q$ is defined as $\{Q_h : h \in \Theta\}$ whose density function with respect to $\nu$ is given by $q(\cdot + h)$ for $h \in \Theta$. 

Consider the product measure $\Gamma_h := P_{\theta+h} \times Q_h$ supported on the product space $\mathcal{X} \times \Theta^{(-\delta)}$ where $\Theta^{(-\delta)}$ is a set of elements in $\Theta$ given by $\{\theta: \theta+u\delta \in \Theta\}$ for all ``directions" of $u \in \Theta$ such that $\|u\|_\Theta=1$. The density of $\Gamma_h$ is given by
\begin{equation}
    \gamma_{h}(x, \theta) := (x, \theta) \in \mathcal{X} \times \Theta^{(-\delta)} \mapsto p_{\theta+h}(x)q(\theta+h)\label{eq:mixture_dist_gamma}
\end{equation}
for each $\|h\|_\Theta < \delta$ and $\delta > 0$ as defined in \ref{as:IPBorder}. We denote by $\E_{X, \theta+h}$ the expectation under the mixture distribution $\gamma_{h}$. Similarly, we denote by $\E_{X, \theta}$ the expectation under $\gamma_{0}$.
% For a fixed $\delta > 0$, we denote by $\Theta^{\delta}$ the $\delta$-enlargement of $\Theta$, that is, the collection of elements in $\mathbb{R}^p$ such that for all $\theta \in \Theta^{\delta}$, there exists $\theta_0 \in \Theta$ with $\|\theta_0 - \theta\| \le \delta$. It follows immediately that $\Theta^{(-\delta)} \subset \Theta \subset \Theta^{\delta}$. 
For any fixed $h$, we have
\begin{align}
    \E_{X, \theta+h} \left(T(X)-\psi(\theta)\right)
    &=\iint_{\mathcal{X}\times \Theta^{(-\delta)}}\left(T(x)-\psi(t)\right) \gamma_{h}(x,t)\, \mu(dx)\,\nu(dt)\nonumber\\
    &=\iint_{\mathcal{X}\times \Theta^{(-\delta)}} \left(T(x)-\psi(t)\right) p_{t+h}(x)q(t+h)\, \mu(dx)\,\nu(dt)\nonumber\\
    &= \iint_{\mathcal{X}\times \{u: u-h\in \Theta^{(-\delta)}\}} \left(T(x)-\psi(u-h)\right)p_u(x)q(u)\, \mu(dx)\,\nu(du).\nonumber
\end{align}
where we use the change of variables with $u=t+h$. In view of \ref{as:IPBorder}, the support of $q$ is contained in $\Theta^{(-2\delta)}$ and we have $\Theta^{(-2\delta)} \subseteq \{u: u-h\in \Theta^{(-\delta)}\}$ when $\|h\|_\Theta < \delta$. Additionally, we have $q(t)=0$ for all $t \in \Theta^{(-\delta)}\setminus \Theta^{(-2\delta)}$. This implies that 
\begin{align}
    &\iint_{\mathcal{X}\times \{u: u-h\in \Theta^{(-\delta)}\}} \left(T(x)-\psi(u-h)\right)p_u(x)q(u)\, \mu(dx)\,\nu(du)\nonumber\\
    &\qquad=\iint_{\mathcal{X}\times \Theta^{(-\delta)}} \left(T(x)-\psi(u-h)\right)p_u(x)q(u)\, \mu(dx)\,\nu(du).\nonumber
\end{align}
We can further write out the above display as follows:
\begin{align}
    \E_{X, \theta+h} \left(T(X)-\psi(\theta)\right)&=\iint_{\mathcal{X}\times \Theta^{(-\delta)}} \left(T(x)-\psi(u-h)\right) p_u(x)q(u)\, \mu(dx)\,\nu(du)\nonumber\\
    &=\iint_{\mathcal{X}\times \Theta^{(-\delta)}} \left(T(x)-\psi(u-h)+\psi(u)-\psi(u)\right) p_u(x)q(u)\, \mu(dx)\,\nu(du)\nonumber\\
    &=\E_{X, \theta}  \left(T(X)-\psi(\theta)\right)+\int_{\Theta} \left(\psi(u)-\psi(u-h)\right) q(u)\,\nu(du)\label{eq:remainder} 
\end{align}
where the second integral of \eqref{eq:remainder} is over $\Theta$ since $q(t)=0$ for all $t \in \Theta\setminus \Theta^{(-\delta)}$.
Next, let us consider the density ratio of the joint probability over $\mathcal{X} \times \Theta$ given by
\begin{align}
    D_h := (x, \theta) \mapsto \frac{\gamma_h(x,\theta)-\gamma_0(x,\theta)}{\gamma_0(x,\theta)}\nonumber.
\end{align}
It then follows from \eqref{eq:remainder} that 
\begin{align}
    \E_{X, \theta} D_h(X, \theta) \left(T(X)-\psi(\theta)\right) &= \E_{X, \theta+h}\left(T(X)-\psi(\theta)\right) - \E_{X, \theta}\left(T(X)-\psi(\theta)\right)\nonumber\\
    &=\int_{\Theta} \left(\psi(u)-\psi(u-h)\right)q(u)\,\nu(du). \label{eq:DhtoD0_simplified}
\end{align}
By Cauchy-Schwarz inequality, we obtain 
\begin{align}
    \left|\int_{\Theta} \left(\psi(u)-\psi(u-h)\right)q(u)\,du\right|^2 &=\left|\int_{\Theta} \left(\psi(u)-\psi(u-h)\right)q(u)I(q(u)>0)\,du\right|^2\nonumber\\
    &= \left|\E_{X, \theta} D_h(X, \theta) \left(T(X)-\psi(\theta)\right)I(q(\theta)>0)\right|^2 \nonumber \\
    &\le \left\{\E_{X, \theta} D_h^2(X, \theta)I(q(\theta)>0)\right\} \left\{\E_{X, \theta}\left|T(X)-\psi(\theta)\right|^2\right\}\label{eq:vt_cauchy_schwarz}.
\end{align}
We now analyze each term in the last display. First, by the tower property of the expectations, we have
\begin{align*}
    \E_{X, \theta}|T(X)-\psi(\theta)|^2&=\int_\Theta \E_t\left|T(X)-\psi(t)\right|^2q(t) \,\nu(dt).
\end{align*}

Next, we analyze $\E_{X, \theta} D_h^2(X, \theta)I(q(\theta)>0)$. By direct evaluation, we have  
\begin{align}
    &\E_{X, \theta}D_h^2(x, \theta)I(q(\theta)>0) \nonumber\\
    &\qquad= \iint_{\mathcal{X}\times \Theta^{(-\delta)}} \left(\frac{\gamma_h(x,t)-\gamma_0(x,t)}{\gamma_0(x,t)}\right)^2\gamma_0(x,t)I(q(t)>0)\,\mu(dx)\,\nu(dt)\nonumber\\
    &\qquad= \iint_{\mathcal{X}\times \Theta} \left(\frac{\gamma_h(x, t)^2}{\gamma_0(x,t)}-2\gamma_h(x, t)+\gamma_0(x, t)\right)I(q(t)>0)\,\mu(dx)\,\nu(dt)\nonumber\\
    &\qquad=\iint_{\mathcal{X}\times \Theta} \frac{\gamma_h(x, t)^2}{\gamma_0(x,t)}I(q(t)>0)\,\mu(dx)\,\nu(dt) -1\nonumber\\
    &\qquad=\iint_{\mathcal{X}\times \Theta} \frac{p_{t+h}(x)^2q(t+h)^2}{p_t(x)q(t)}I(q(t)>0)\,\mu(dx)\,\nu(dt) -1\nonumber\\
    &\qquad=\int_{\Theta} \frac{q(t+h)^2}{q(t)}I(q(t)>0)\int_{\mathcal{X}} \left(\frac{p_{t+h}(x)^2}{p_t(x)}+\frac{p_t(x)^2}{p_t(x)}-\frac{p_t(x)^2}{p_t(x)}\right)\,\mu(dx)\,\nu(dt) -1\label{eq:tonelli1}\\
    &\qquad= \int_{\Theta}\frac{q(t+h)^2}{q(t)}I(q(t)>0)\left(1+\int_{\mathcal{X}} \frac{\left\{p_{t+h}(x)-p_t(x)\right\}^2}{p_t(x)}\,\mu(dx)\right)\,\nu(dt) -1\label{eq:middle_step}\\
    % &= \int_{\Theta}\frac{q(\theta+h)^2}{q(\theta)}\,\nu(dt)+\iint_{\mathcal{X}\times \Theta} \frac{q(\theta+h)^2}{q(\theta)}\frac{\left\{p_{\theta+h}(x)-p_\theta(x)\right\}^2}{p_\theta(x)}\,\mu(dx)\,\nu(dt) -1\nonumber\\
    &\qquad= \int_{\Theta}\frac{\left\{q(t+h)-q(t)\right\}^2}{q(t)}I(q(t)>0)\,\nu(dt)+\iint_{\mathcal{X}\times \Theta} \frac{q(t+h)^2}{q(t)}\frac{\left\{p_{t+h}(x)-p_t(x)\right\}^2}{p_t(x)}I(q(t)>0)\,\mu(dx)\,\nu(dt) \label{eq:middle_step2}\\
    &\qquad= \overline{\chi}^2(Q_h\|Q)+\int_\Theta\frac{q(t+h)^2}{q(t)} \chi^2(P_{t+h}\|P_t)I(q(t)>0)\,\nu(dt) \label{eq:tonelli2}
\end{align}
where \eqref{eq:middle_step} follows from adding and subtracting $\frac{2p_t(x)p_{t+h}(x)}{p_t(x)}$ and integrating the additional terms. The equality \eqref{eq:middle_step2} follows by an analogous argument. The two lines \eqref{eq:tonelli1} and \eqref{eq:tonelli2} both follow from Tonelli's theorem. From the inequality \eqref{eq:vt_cauchy_schwarz}, we obtain 
\begin{align*}
    \int_\Theta \E_t\left|T(X)-\psi(t)\right|^2q(t) \,\nu(dt) 
    &\geq \frac{\left|\int_{\Theta} \left(\psi(u)-\psi(u-h)\right)q(u)\,\nu(du)\right|^2}{\E_{X, \theta} D_h^2(X, \theta)I(q(\theta)>0)}\\
    &= \frac{\left|\int_{\Theta} \left(\psi(u)-\psi(u-h)\right)q(u)\,du\right|^2}{ \overline{\chi}^2(Q_h\|Q)+\int_\Theta\frac{q(t+h)^2}{q(t)} \chi^2(P_{t+h}\|P_t)I(q(t)>0)\,\nu(dt)}.
\end{align*}

Since $T$ and $h$ do not appear in both sides of the expression, we conclude the claim by taking the infimum over $T$ and the supremum over $\|h\|_\Theta < \delta$. 

For a vector-valued functional $\psi := \Theta \mapsto \mathbb{R}^k$, we prove the matrix analogue to the above statement. We assume $h \in \Theta$ is fixed. For any $a \in \mathbb{R}^k$, we have
\begin{align*}
   &a^T\left(\int_{\Theta} \E_{t}\{T(X)-\psi(t)\}\{T(X)-\psi(t)\}^T\, q(t)\, \nu(dt) \right)a= \int_{\Theta} \E_{t}\left|a^TT(X)-a^T\psi(t)\right|^2\, q(t)\, \nu(dt).
\end{align*}
We now consider $\widetilde{T}(X) := a^TT(X)$ as a univariate estimator of the real-valued functional $\widetilde{\psi}(\theta) := a^T\psi(\theta)$, and apply the univariate result we just provided. We then obtain
\begin{align*}
   \int_{\Theta}\E_{t}\left|\widetilde{T}(X)-\widetilde{\psi}(t)\right|^2q(t)\, \nu(dt) &\ge  \frac{\left|\int_{\Theta} \left(\widetilde{\psi}(t+h)-\widetilde{\psi}(t)\right)q(t)\,\nu(dt)\right|^2}{\overline{\chi}^2(Q_h\|Q)+\int_\Theta\frac{q(t+h)^2}{q(t)} \chi^2(P_{t+h}\|P_t)I(q(t)>0)\,\nu(dt)}\\
   & =  a^T\left(\frac{\int_\Theta\left\{\psi(t+h)-\psi(t)\right\}\left\{\psi(t+h)-\psi(t)\right\}^T q(t)\, \nu(dt)}{\overline{\chi}^2(Q_h\|Q)+\int_\Theta\frac{q(t+h)^2}{q(t)} \chi^2(P_{t+h}\|P_t)I(q(t)>0)\,\nu(dt)}\right)a
\end{align*}
where the last equality follows since the denominator is a scalar quantity not depending on $\psi$. Since the vector $a \in \mathbb{R}^k$ was arbitrary, we conclude the first statement by the definition of positive semi-definite matrices.
\end{proof}
\begin{proof}
The proof is identical up to the equality \eqref{eq:DhtoD0_simplified} in the proof of Theorem~\ref{thm:crvtBound} where we establish 
\begin{align}
    \int_{\Theta} \left(\psi(u)-\psi(u-h)\right)q(u)\,\nu(du)=
    \E_{X, \theta} D_h(X, \theta) \left(T(X)-\psi(\theta)\right). \nonumber
    % \label{eq:DhtoD0_simplified}
\end{align}For a vector-valued functional $\psi := \Theta \mapsto \mathbb{R}^k$ and its norm $\|\cdot \| : \mathbb{R}^k \mapsto \mathbb{R}$, we have
\begin{align}
    \left\|\int_{\Theta} \left\{\psi(t)-\psi(t-h)\right\}q(t)I(q(t)>0)\,\nu(dt)\right\|^2 &= \left\|\E_{X, \theta} D_h(X, \theta) \left\{T(X)-\psi(\theta)\right\} I(q(\theta)>0)\right\|^2\nonumber \\
    &\le  \left\{\E_{X, \theta} |D_h(X, \theta)
| \left\|T(X)-\psi(\theta)\right\|I(q(\theta)>0)\right\}^2 \nonumber \\
    &\le \E_{X, \theta} |D^2_h(X, \theta)I(q(\theta)>0)|\E_{X, \theta}\left\|T(X)-\psi(\theta)\right\|^2\nonumber.
\end{align}   
where the first inequality follows from Jensen's inequality and the second inequality follows from Cauchy-Schwartz inequality. The rest of the proof is analogous to that of Theorem~\ref{thm:crvtBound}. 
\end{proof}
\clearpage
\subsection{Proof of Theorem~\ref{thm:crvtBound_hellinger} \kt{Almost done}}
\begin{proof}[\bfseries{Proof of Theorem~\ref{thm:crvtBound_hellinger}}]
We begin with the equality \eqref{eq:DhtoD0_simplified} in the proof of Theorem~\ref{thm:crvtBound} where we establish 
\begin{align}
    \int_{\Theta} \left(\psi(u)-\psi(u-h)\right)q(u)\,\nu(du)=
    \E_{X, \theta} D_h(X, \theta) \left(T(X)-\psi(\theta)\right). \nonumber
    % \label{eq:DhtoD0_simplified}
\end{align}
By Cauchy-Schwarz inequality, we obtain 
\begin{align}
    \left|\int_{\Theta} \left(\psi(u)-\psi(u-h)\right)q(u)\,\nu(du)\right|^2 &= \left|\E_{X, \theta} \left(\frac{\gamma_h(X,\theta)-\gamma_0(X,\theta)}{\gamma_0(X,\theta)}\right) \left(T(X)-\psi(\theta)\right)\right|^2 \nonumber \\
    &= \left|\E_{X, \theta} \left(\sqrt{\frac{\gamma_h(X,\theta)}{\gamma_0(X,\theta)}}-1\right)\left(\sqrt{\frac{\gamma_h(X,\theta)}{\gamma_0(X,\theta)}}+1\right) \left(T(X)-\psi(\theta)\right)\right|^2 \nonumber \\
    &\le \left\{\E_{X, \theta} \left(\sqrt{\frac{\gamma_h(X,\theta)}{\gamma_0(X,\theta)}}+1\right)^2 \left(T(X)-\psi(\theta)\right)^2 \right\}\E_{X, \theta} \left(\sqrt{\frac{\gamma_h(X,\theta)}{\gamma_0(X,\theta)}}-1\right)^2\nonumber \\
    &\le 2\left\{\E_{X, \theta} \left(T(X)-\psi(\theta)\right)^2 + \E_{X, \theta+h} \left(T(X)-\psi(\theta)\right)^2\right\}\E_{X, \theta} \left(\sqrt{\frac{\gamma_h(X,\theta)}{\gamma_0(X,\theta)}}-1\right)^2\nonumber 
\end{align}
where we apply the elementary inequality $(a+b)^2 \le 2(a^2+b^2)$ in the last step. 
\[\E_{X, \theta} \left(\sqrt{\frac{\gamma_h(X,\theta)}{\gamma_0(X,\theta)}}-1\right)^2 = \iint \left(\sqrt{\frac{\gamma_h(x,t)}{\gamma_0(x,t)}}-1\right)^2\gamma_0(x,t)\,\mu(dx)\,\nu(dt) = \iint \left(\sqrt{\gamma_h(x,t)}-\sqrt{\gamma_0(x,t)}\right)^2\,\mu(dx)\,\nu(dt),\]
which by definition corresponds to the squared Hellinger distance between probability measures $\Gamma_h$ and $\Gamma_0$. 

Since minimax risk upper bounds Bayes risk, we have $\E_{X, \theta} \left(T(X)-\psi(\theta)\right)^2 \le \sup_{\theta \in \Theta} \E_\theta \left(T(X)-\psi(\theta)\right)^2$. For the second term in the bracket, we have
\begin{align*}
    \E_{X, \theta+h} \left(T(X)-\psi(\theta)\right)^2 &= \int_{\Theta^{(-\delta)}}\E_{t+h}\left(T(X)-\psi(t)\right)^2q(t+h) \, \nu(dt) \\
    & =\int_{\Theta^{(-\delta)}}\E_{t+h}\left(T(X)-\psi(t)-\psi(t+h)+\psi(t+h)\right)^2q(t+h) \, \nu(dt) \\
    & = \int_{\Theta^{(-\delta)}}\E_{t+h}\left(T(X)-\psi(t+h)\right)^2q(t+h) \, \nu(dt) \\
    &\qquad + \int_{\Theta^{(-\delta)}}\{\psi(t+h)-\psi(t)\}^2 q(t+h) \, \nu(dt) \\
    &\qquad + 2\int_{\Theta^{(-\delta)}}\E_{t+h}\left(T(X)-\psi(t+h)\right)\left(\psi(t+h)-\psi(t)\right)q(t+h) \, \nu(dt)\\
    & \le \int_{\Theta^{(-\delta)}}\E_{t+h}\left(T(X)-\psi(t+h)\right)^2q(t+h) \, \nu(dt) \\
    &\qquad + \int_{\Theta^{(-\delta)}}\{\psi(t+h)-\psi(t)\}^2 q(t+h) \, \nu(dt) \\
    &\qquad + 2\sqrt{\int_{\Theta^{(-\delta)}}\E_{t+h}\left(T(X)-\psi(t+h)\right)^2\,\nu(dt)}\sqrt{\int_{\Theta^{(-\delta)}} \left(\psi(t+h)-\psi(t)\right)^2q(t+h) \, \nu(dt)}\\
    &=\left(\sqrt{\int_{\Theta^{(-\delta)}}\E_{t+h}\left(T(X)-\psi(t+h)\right)^2\,\nu(dt)}+\sqrt{\int_{\Theta^{(-\delta)}} \left(\psi(t+h)-\psi(t)\right)^2q(t+h) \, \nu(dt)}\right)^2
\end{align*}

\begin{align*}
    &\frac{\left|\int_{\Theta} \left(\psi(u)-\psi(u-h)\right)q(u)\,\nu(du)\right|^2}{2\E_{X, \theta} \left(\sqrt{\frac{\gamma_h(X,\theta)}{\gamma_0(X,\theta)}}-1\right)^2} \\
    &\qquad\le\E_{X, \theta} \left(T(X)-\psi(\theta)\right)^2+ \left( \sqrt{\int_{\Theta^{(-\delta)}}\E_{t+h}\left(T(X)-\psi(t+h)\right)^2\,\nu(dt)}+\sqrt{\int_{\Theta^{(-\delta)}} \left(\psi(t+h)-\psi(t)\right)^2q(t+h) \, \nu(dt)}\right)^2\\
    &\qquad\le\sup_{t \in\Theta}\E_{t} \left(T(X)-\psi(t)\right)^2+ \left( \sqrt{\sup_{t \in\Theta}\E_{t}\left(T(X)-\psi(t)\right)^2}+\sqrt{\int_{\Theta^{(-\delta)}} \left(\psi(t+h)-\psi(t)\right)^2q(t+h) \, \nu(dt)}\right)^2\\
        &\qquad\le2\left( \sqrt{\sup_{t \in\Theta}\E_{t}\left(T(X)-\psi(t)\right)^2}+\sqrt{\int_{\Theta^{(-\delta)}} \left(\psi(t+h)-\psi(t)\right)^2q(t+h) \, \nu(dt)}\right)^2
\end{align*}

We thus obtain 
\begin{align*}
    &\sup_{t \in\Theta}\E_{t}\left(T(X)-\psi(t)\right)^2\\
    &\qquad \ge \left[\left\{\frac{\left|\int_{\Theta} \left(\psi(u)-\psi(u-h)\right)q(u)\,\nu(du)\right|^2}{4\E_{X, \theta} \left(\sqrt{\frac{\gamma_h(X,\theta)}{\gamma_0(X,\theta)}}-1\right)^2} \right\}^{1/2}-\left\{\int_{\Theta^{(-\delta)}} \left(\psi(t+h)-\psi(t)\right)^2q(t+h) \, \nu(dt)\right\}^{1/2}\right]^2_+.
\end{align*}

Hellinger distance between $\Gamma_h$ and $\Gamma_0$ can be furthered written out as follows:
\begin{align*}
    H^2(\Gamma_h, \Gamma_0)&=\E_{X, \theta} \left(\sqrt{\frac{\gamma_h(x,\theta)}{\gamma_0(x,\theta)}}-1\right)^2 \\
    &=\E_{X, \theta} \left(\frac{\gamma_h(x,\theta)}{\gamma_0(x,\theta)}+1 - 2\sqrt{\frac{\gamma_h(x,\theta)}{\gamma_0(x,\theta)}}\right)\\
    % &=2-2\iint_{\mathcal{X}\times \Theta}  \gamma^{1/2}_h(x,\theta)\gamma^{1/2}_0(x,\theta)\, \mu(dx)\,\nu(dt)\\
    &=2-2\iint_{\mathcal{X}\times \Theta}  p^{1/2}_{\theta+h}(x)q^{1/2}(\theta+h)p^{1/2}_{\theta}(x)q^{1/2}(\theta)\, \mu(dx)\,\nu(dt) \\
    &=2-2\int_{\Theta} q^{1/2}(\theta+h)q^{1/2}(\theta)\int_{\mathcal{X}}  p^{1/2}_{\theta+h}(x)p^{1/2}_{\theta}(x)\, \mu(dx)\,\nu(dt)\\
    &=2-2\int_{\Theta} q^{1/2}(\theta+h)q^{1/2}(\theta)\left(1-\frac{1}{2}H^2(P_{\theta+h}, P_{\theta})\right)\,\nu(dt)\\
    &=H^2(Q_h, Q) +\int_{\Theta} q^{1/2}(\theta+h)q^{1/2}(\theta)H^2(P_{\theta+h}, P_{\theta})\,\nu(dt) 
\end{align*}

% \begin{align}
% \sup_{\theta\in\Theta}\E_\theta\left(T(X)-\psi(\theta)\right)^2&\ge 
%     \frac{\left|\int_{\Theta} \left(\psi(u)-\psi(u-h)\right)q(u)\,du\right|^2}{4\E_{X, \theta} \left(\sqrt{\frac{\gamma_h(x,\theta)}{\gamma_0(x,\theta)}}-1\right)^2} \nonumber \\
%     &=  \frac{\left|\int_{\Theta} \left(\psi(u)-\psi(u-h)\right)q(u)\,du\right|^2}{4\left\{H^2(Q_h, Q) +\int_{\Theta} q^{1/2}(\theta+h)q^{1/2}(\theta)H^2(P_{\theta+h}, P_{\theta})\,\nu(dt)\right\}}\nonumber
% \end{align}
\kt{After fixing the issue, we have
\begin{align}
&\sup_{\theta\in\Theta}\E_\theta\left(T(X)-\psi(\theta)\right)^2+\int_{\Theta} \left(\psi(u)-\psi(u-h)\right)^2q(u)\,du \nonumber\\
&\qquad+ 2\int_{\Theta^{(-\delta)}}\left(\E_{\theta+h}T-\psi(\theta+h)\right)\left(\psi(\theta+h)-\psi(\theta)\right)q(\theta+h) \, \nu(dt) \ge 
    \frac{\left|\int_{\Theta} \left(\psi(u)-\psi(u-h)\right)q(u)\,du\right|^2}{4\E_{X, \theta} \left(\sqrt{\frac{\gamma_h(x,\theta)}{\gamma_0(x,\theta)}}-1\right)^2} \nonumber \\
    &\qquad\implies \sup_{\theta\in\Theta}\E_\theta\left(T(X)-\psi(\theta)\right)^2 \ge  \frac{\left|\int_{\Theta} \left(\psi(u)-\psi(u-h)\right)q(u)\,du\right|^2}{4H^2(\Gamma_h, \Gamma)}-\int_{\Theta} \left(\psi(u)-\psi(u-h)\right)^2q(u)\,du\nonumber
\end{align}
We need to either lower bound $\left|\int \left(\psi(u)-\psi(u-h)\right)q(u)\,du\right|^2$ or upper bound $\int \left(\psi(u)-\psi(u-h)\right)^2q(u)\,du$. Jensen's inequality cannot be used here. As a special case of $\psi(\theta)=\theta$, we get
\begin{align*}
    \sup_{\theta\in\Theta}\E_\theta\left(T(X)-\theta\right)^2 \ge  \sup_{\|h\|_\Theta\le \delta}\frac{1-4H^2(\Gamma_h, \Gamma)}{4H^2(\Gamma_h, \Gamma)}\left|h\right|^2
\end{align*}
}
This concludes the claim. 
\kt{The current statement is 
\begin{align*}
   & \inf_{T}\sup_{\theta \in \Theta}\E_{\theta}\left\{T(X)-\psi(\theta)\right\}^2 \\
   &\qquad\ge  \sup_{ \|h\|_\Theta<\delta}\left[\frac{\left|\int_{\Theta} \left(\psi(u)-\psi(u-h)\right)q(u)\,du\right|}{2H(\Gamma_h, \Gamma_0)} -\left\{\int_{\Theta^{(-\delta)}}\left(\psi(\theta+h)-\psi(\theta)\right)^2q(\theta+h) \, \nu(dt)\right\}^{1/2}\right]_+^2
\end{align*}
This looks unnecessarily complicated and I am not sure what the multivariate version looks like.As a special case of $\psi(\theta)=\theta$, we get
\begin{align*}
    \sup_{\theta\in\Theta}\E_\theta\left(T(X)-\theta\right)^2 \ge  \sup_{\|h\|_\Theta\le \delta}\left[\frac{|h|}{2H(\Gamma_h, \Gamma_0)} -|h|\right]_+^2
\end{align*}
}
Here we use $2ab \le a^2L + b^2/L$ for any $L \ge 0$. 
By Cauchy-Schwarz inequality, we obtain 
\begin{align}
    &\frac{\left|\int_{\Theta} \left(\psi(u)-\psi(u-h)\right)q(u)\,du\right|^2}{2H^2(\Gamma_h, \Gamma_0)}\le \E_{X, \theta} \left(T(X)-\psi(\theta)\right)^2 + \E_{X, \theta+h} \left(T(X)-\psi(\theta)\right)^2\nonumber 
\end{align}
For the second term, we have 
\begin{align*}
    &\int_{\Theta^{(-\delta)}}\E_{t+h}\left(T(X)-\psi(t)\right)^2q(t+h) \, \nu(dt) \\
    &\qquad =\int_{\Theta^{(-\delta)}}\E_{t+h}\left(T(X)-\psi(t)-\psi(t+h)+\psi(t+h)\right)^2q(t+h) \, \nu(dt) \\
    &\qquad = \int_{\Theta^{(-\delta)}}\E_{t+h}\left(T(X)-\psi(t+h)\right)^2q(t+h) \, \nu(dt) + \int_{\Theta^{(-\delta)}}\{\psi(t+h)-\psi(t)\}^2 q(t+h) \, \nu(dt) \\
    &\qquad\qquad + 2\int_{\Theta^{(-\delta)}}\E_{t+h}\left(T(X)-\psi(t+h)\right)\left(\psi(t+h)-\psi(t)\right)q(t+h) \, \nu(dt) \\
    &\qquad \le \int_{\Theta^{(-\delta)}}\E_{t+h}\left(T(X)-\psi(t+h)\right)^2q(t+h) \, \nu(dt) + \int_{\Theta^{(-\delta)}}\{\psi(t+h)-\psi(t)\}^2 q(t+h) \, \nu(dt) \\
    &\qquad\qquad + \int_{\Theta^{(-\delta)}}\E_{t+h}\left\{L\left(T(X)-\psi(t+h)\right)^2 + \frac{\left(\psi(t+h)-\psi(t)\right)^2}{L}\right\}q(t+h) \, \nu(dt) \\
     &\qquad = (1+L)\int_{\Theta^{(-\delta)}}\E_{t+h}\left(T(X)-\psi(t+h)\right)^2q(t+h) \, \nu(dt) \\
     &\qquad\qquad+(1+1/L) \int_{\Theta^{(-\delta)}}\{\psi(t+h)-\psi(t)\}^2 q(t+h) \, \nu(dt) 
\end{align*}
for any $L$. Plugging into this result, we get
\begin{align}
    &(2+L)\E_{X, \theta} \left(T(X)-\psi(\theta)\right)^2 \nonumber\\
    &\qquad \ge \frac{\left|\int_{\Theta}\nonumber \left(\psi(u)-\psi(u-h)\right)q(u)\,du\right|^2}{2H^2(\Gamma_h, \Gamma_0)}- \left(1+\frac{1}{L}\right) \int_{\Theta^{(-\delta)}}\{\psi(\theta+h)-\psi(\theta)\}^2 q(\theta+h) \, \nu(dt) \nonumber\\
    &\implies \sup_{\theta \in \Theta}\E_{X, \theta} \left(T(X)-\psi(\theta)\right)^2\nonumber\\
    &\qquad \ge \sup_{L\ge0}\frac{\left|\int_{\Theta}\nonumber \left(\psi(u)-\psi(u-h)\right)q(u)\,du\right|^2}{2(2+L)H^2(\Gamma_h, \Gamma_0)}- \frac{L+1}{L(2+L)} \int_{\Theta^{(-\delta)}}\{\psi(\theta+h)-\psi(\theta)\}^2 q(\theta+h) \, \nu(dt) \nonumber
\end{align}
\kt{This will recover LAM by picking $L = h$ and let $h \to 0$.}
Let $A := \frac{\left|\int_{\Theta}\nonumber \left(\psi(u)-\psi(u-h)\right)q(u)\,du\right|^2}{2H^2(\Gamma_h, \Gamma_0)}$ and $B:= \int_{\Theta^{(-\delta)}}\{\psi(\theta+h)-\psi(\theta)\}^2 q(\theta+h) \, \nu(dt)$. Consider the following function 
\[Q(x) := \frac{A}{2+x} - \frac{x+1}{x(2+x)}B\]
Derivative is
\begin{align*}
Q'(x) &= -\frac{A}{(2 + x)^2} + \frac{x^2 + 2x + 2}{x^2(x + 2)^2}B\\ 
&= -\frac{B}{(x + 2)^2}\left[\frac{A}{B} - 1 - \frac{2}{x} - \frac{2}{x^2}\right]\\
&= -\frac{B}{(x + 2)^2}\left[\frac{A}{B} - \frac{1}{2} - \frac{1}{2} - \frac{2}{x} - \frac{2}{x^2}\right]\\
&= -\frac{B}{(x + 2)^2}\left[\left(\frac{A}{B} - \frac{1}{2}\right) - 2\left(\frac{1}{2} + \frac{1}{x}\right)^2\right].
\end{align*}
If $A/B - 1 < 0$, then the derivative is positive for all $x > 0$ and hence, the minimum is attained at $x = 0$.
If $A/B - 1 \ge 0$, then the derivative is zero at $x = ((A/(2B) - 1/4)^{1/2} - 1/2)^{-1}$.

The second derivative is
\begin{align*}
Q''(x) &= \frac{2A}{(2 + x)^3} + \frac{2x^2(x+2)^2(x + 1)-4x(x+1)(x+2)(x^2+2x+2)}{x^4(x + 2)^4}B\\ 
 &= \frac{2A}{(2 + x)^3} + \frac{2x(x+2)(x + 1)-4(x+1)(x^2+2x+2)}{x^3(x + 2)^3}B
\end{align*}
\kt{A few ideas:
\begin{itemize}
    \item Using the fact that $1/L \ge \frac{L+1}{L(2+L)} \ge 1/2L$, we can somehow simplify the last expression
    \item If we assume $|\psi(\theta+h)-\psi(\theta)| \le C_\psi |h|^\alpha$, we can then pick $L = |h|^\alpha$. The last term will then 
    \begin{align*}
        \frac{h^\alpha+1}{h^\alpha(2+h^\alpha)} \int_{\Theta^{(-\delta)}}\{\psi(\theta+h)-\psi(\theta)\}^2 q(\theta+h) \, \nu(dt) \le  \frac{1}{h^\alpha} C_\psi^2 |h|^{2\alpha} = C_\psi^2 |h|^{\alpha}
    \end{align*}
    The final expression is 
    \[\frac{\left|\int_{\Theta}\nonumber \left(\psi(u)-\psi(u-h)\right)q(u)\,du\right|^2}{2(2+h^\alpha)H^2(\Gamma_h, \Gamma_0)}-C_\psi^2 |h|^{\alpha}\]
\end{itemize}
When $\psi(\theta) = \theta$, we have
\begin{align*}
    \frac{h^2}{2+L}\left(\frac{1}{2H^2(\Gamma_h, \Gamma_0)}-\frac{L+1}{L}\right)
\end{align*}
}

\end{proof}

\clearpage
\section{Minimax lower bound based on Hellinger distance}
\subsection{Derivation of a sharper constant for the two-point lower bound}
Here we present the improvement of Theorem 6.1 for general functionals with a sharper constant.
\begin{proof}[\bfseries{Proof of Theorem~\ref{thm:sharper_ihbound}}]
For any estimator $T$ and an arbitrary constant $c$, we have 
\begin{align}
    \left|\E_{\theta+h} T - \E_{\theta} T\right|^2 &= \left|\int_\mathcal{X} \{T(x)-c\} \{p_{\theta+h}(x)-p_\theta(x)\}\, \mu(dx)\right|^2\nonumber\\
    &=\left|\int_\mathcal{X}  \{T(x)-c\} \left\{p^{1/2}_{\theta+h}(x)-p^{1/2}_\theta(x)\right\}\left\{p^{1/2}_{\theta+h}(x)+p^{1/2}_\theta(x)\right\}\, \mu(dx)\right|^2\nonumber\\
    &\le2H^2(P_{\theta+h}, P_\theta)\int_\mathcal{X}  \{T(x)-c\}^2 \left\{p_{\theta+h}(x)+p_\theta(x)\right\}\, \mu(dx).\label{eq:proofB2_CS_ineq}
\end{align}
where the last inequality follows by Cauchy–Schwarz inequality and $(a+b)^2 \le 2a^2 + 2b^2$. The first term of the right-hand side follows that 
\begin{align*}
    \int_\mathcal{X}  \left(T(x)-c\right)^2 p_{\theta+h}(x)\, \mu(dx)&=\int_\mathcal{X}  \{T(x)-\E_{\theta+h}T+\E_{\theta+h}T-c\}^2 p_{\theta+h}(x)\, \mu(dx) \\
    &=\text{Var}_{\theta+h}T + \{\E_{\theta+h}T-c\}^2\\
    &=\E_{\theta+h}|T-\psi(\theta+h)|^2 -|\E_{\theta+h}T - \psi(\theta+h)|^2+ \{\E_{\theta+h}T-c\}^2.
\end{align*}
By repeating the analogous argument for $\int_\mathcal{X}  \{T(x)-c\}^2 p_{\theta}(x)\, \mu(dx)$ and plugging them into \eqref{eq:proofB2_CS_ineq}, we obtain 
\begin{align*}
     \left|\E_{\theta+h} T - \E_{\theta} T\right|^2 &\le2H^2(P_{\theta+h}, P_\theta)\left(\E_{\theta+h}|T-\psi(\theta+h)|^2 -|\E_{\theta+h}T - \psi(\theta+h)|^2\right.\\
     &\qquad+ \{\E_{\theta+h}T-c\}^2 + \E_{\theta}|T-\psi(\theta)|^2 -|\E_{\theta}T - \psi(\theta)|^2+ \{\E_{\theta}T-c\}^2\left.\right).
\end{align*}
Since the above inequality holds for an arbitrary constant $c$, we choose $c$ to minimize the upper bound. As the optimal $c^*$ is given by $c^* = \frac{1}{2}\left(\E_{\theta}T+\E_{\theta+h}T\right)$, we can further simplify the expression as 
\begin{align*}
     \left|\E_{\theta+h} T - \E_{\theta} T\right|^2 &\le2H^2(P_{\theta+h}, P_\theta)\left(\E_{\theta+h}|T-\psi(\theta+h)|^2 +\E_{\theta}|T-\psi(\theta)|^2\right. \\
     &\qquad  \left.-d^2(\theta+h)-d^2(\theta)+ \frac{\left|\E_{\theta}T-\E_{\theta+h}T\right|^2}{2}  \right)\, .
\end{align*}
where we define $d(\theta):=\E_\theta T-\psi(\theta)$.
The above display immediately implies the following:
\begin{align*}
     &\implies \E_{\theta+h}|T-\psi(\theta+h)|^2 +\E_{\theta}|T-\psi(\theta)|^2 \ge \frac{1-H^2(P_{\theta+h}, P_\theta)}{2H^2(P_{\theta+h}, P_\theta)}\left|\E_{\theta+h} T - \E_{\theta} T\right|^2+ d^2(\theta+h)+d^2(\theta)\\
     &\implies \E_{\theta+h}|T-\psi(\theta+h)|^2 +\E_{\theta}|T-\psi(\theta)|^2 \\
     &\qquad \ge \frac{1-H^2(P_{\theta+h}, P_\theta)}{2H^2(P_{\theta+h}, P_\theta)}\left| \psi(\theta+h)-\psi(\theta)+
     d(\theta+h)-d(\theta)\right|^2+ d^2(\theta+h)+d^2(\theta).
\end{align*}
The existing proofs by \cite{ibragimov1981statistical} and \cite{lin2019optimal} proceed by studying two cases: i) $\max\{|d(\theta+h)|, |d(\theta)|\} < \frac{1}{4}|\psi(\theta+h)-\psi(\theta)|$ and ii) $|d(\theta)| > \frac{1}{4}|\psi(\theta+h)-\psi(\theta)|$. We instead optimize this boundary to obtain the sharper constant.
We now define the following function
\[
\eta(x, y) = A(B + x - y)^2 + x^2 + y^2.
\]
Then the lower bound above can be written as
\[
E_{\theta + h}|T - \psi(\theta + h)|^2 + E_{\theta}|T - \psi(\theta)|^2 \ge \eta(d(\theta + h), d(\theta)),
\]
with $A = \frac{1 - H^2(P_{\theta + h}, P_{\theta})}{2H^2(P_{\theta + h}, P_{\theta})}$ and $B = \psi(\theta + h) - \psi(\theta)$. This further implies that
\[
E_{\theta + h}|T - \psi(\theta + h)|^2 + E_{\theta}|T - \psi(\theta)|^2 \ge \min_{x, y\in\mathbb{R}}\,\eta(x, y).
\]
The minimizer of $\eta$ is $x^* = -y^* = -\frac{2AB}{4A + 2}$ and hence,
\[
\min_{x, y}\eta(x, y) = \frac{4AB^2}{(4A + 2)^2} + \frac{8A^2B^2}{(4A + 2)^2} = \frac{4AB^2(1 + 2a)}{(4A + 2)^2} = \frac{AB^2}{2A + 1}.
\]
Now we have 
\begin{align*}
    \partial_{xx}\eta = 2A+2\,, \partial_{xy}\eta = -2A\,, \text{ and }\, \partial_{yy}\eta = 2A+2
\end{align*}
and the discriminant is given by $(2A+2)^2-4A^2 = 4(2A+1)$. Hence the optima is at a saddle point when $A < -1/2$. The constant $A$ is defined as $(1 - H^2(P_{\theta + h}, P_{\theta}))/(2H^2(P_{\theta + h}, P_{\theta}))$, which is monotone decreasing with respect to $H^2(P_{\theta + h}, P_{\theta})$ and attains the minimum $-1/4$ at $H^2(P_{\theta + h}, P_{\theta})=2$. Thus the minimizer of $\eta$ is well-defined for all values of $A$ and thereby all values of $H^2(P_{\theta + h}, P_{\theta})$. The minimum of the function $\eta$ with respect to $d(\theta + h)$ and $d(\theta)$ is thus given by 
\begin{align*}
    \frac{AB^2}{2A+1} &= \frac{1-H^2(P_{\theta+h}, P_\theta)}{2H^2(P_{\theta+h}, P_\theta)}\left| \psi(\theta+h)-\psi(\theta)\right|^2 / \left(\frac{1-H^2(P_{\theta+h}, P_\theta)}{H^2(P_{\theta+h}, P_\theta)}+1\right) \\
    &= \frac{1-H^2(P_{\theta+h}, P_\theta)}{2}\left| \psi(\theta+h)-\psi(\theta)\right|^2
\end{align*}

When $H^2(P_{\theta+h}, P_\theta) > 1$, the leading constant becomes negative and we replace with a trivial lower bound of zero. 
Therefore, we conclude
\[
\frac{1-H^2(P_{\theta+h}, P_\theta)}{2}\left| \psi(\theta+h)-\psi(\theta)\right|^2 E_{\theta + h}|T - \psi(\theta + h)|^2 + E_{\theta}|T - \psi(\theta)|^2 \ge  \left(\frac{1 -H^2(P_{\theta + h}, P_{\theta})}{2}\right)_+|\psi(\theta + h) - \psi(\theta)|^2.
\]

\end{proof}

% \begin{align*}
%     \E_{X, \theta} \left(\frac{\gamma^{1/2}_h(x,\theta)}{\gamma^{1/2}_0(x,\theta)}-1\right)^2 &=\E_{X, \theta} \left(\frac{\gamma_h(x,\theta)}{\gamma_0(x,\theta)}+1 - 2\frac{\gamma^{1/2}_h(x,\theta)}{\gamma^{1/2}_0(x,\theta)}\right)\\
%     &=2-2\iint  \gamma^{1/2}_h(x,\theta)\gamma^{1/2}_0(x,\theta)\, \mu(dx)\,\nu(dt)\\
%     &=2-2\iint  p^{1/2}_{\theta+h}(x)q^{1/2}(\theta+h)p^{1/2}_{\theta}(x)q^{1/2}(\theta)\, \mu(dx)\,\nu(dt) \\
%     &=2-2\int q^{1/2}(\theta+h)q^{1/2}(\theta)\int  p^{1/2}_{\theta+h}(x)p^{1/2}_{\theta}(x)\, \mu(dx)\,\nu(dt)\\
%     &=2-2\int q^{1/2}(\theta+h)q^{1/2}(\theta)\left(1-\frac{1}{2}H^2(f_{\theta}, p_{\theta+h})\right)\,\nu(dt)\\
%     &=2-2\int q^{1/2}(\theta+h)q^{1/2}(\theta)\,\nu(dt) +\int q^{1/2}(\theta+h)q^{1/2}(\theta)H^2(f_{\theta}, p_{\theta+h})\,\nu(dt) 
% \end{align*}

% \begin{align*}
% &\E_{X, \theta}  \left(T(X)-\psi(\theta)\right)^2\\
%     &\quad \ge \frac{\left\{\int_{\Theta} \left(\psi(u)-\psi(u-h)\right)q(u)\,d\lambda\right\}^2}{12-12\int q^{1/2}(\theta+h)q^{1/2}(\theta)\,\nu(dt) +6\int q^{1/2}(\theta+h)q^{1/2}(\theta)H^2(f_{\theta}, p_{\theta+h})\,\nu(dt) }-\frac{2}{3}\int_{\Theta} \left(\psi(u)-\psi(u-h)\right)^2 q(u)\,du  
% \end{align*}
% and subject to $\E_{X, \theta}D^2_h(x, \theta) > 0$, we have
% \begin{equation}
%     \frac{\left|\E_{X, \theta} D_h(x, \theta) \left(T(X)-\psi(\theta)\right) \right|^2}{\E_{X, \theta}D^2_h(x, \theta)} \le \E_{X, \theta}  \left\{T(X)-\psi(\theta)\right\} ^2.\label{eq:Cauchy_Schwarz}
% \end{equation}
% When $\E_{X, \theta}D^2_h(x, \theta) = 0$, we allow the lower bound to diverge. 
