# Supplementary material for: Generalized van Trees inequality: Local minimax bounds for non-smooth functionals and irregular statistical models
Source: arXiv:2405.06437 source file (2024-10-19)
Supplement: Supplementary file 2 [file diffeq.tex]

\newpage
\section{Setting up a differential equation}
Let $u(t) = \sqrt{g(t)}$ where the support of $g$ is contained in $(-1,1)$. Further, we require that $u(1)=u(-1)=0$ and $\int u^2(t)\, dt=1$. We denote by  $\dot{u}(t)$ the derivative of $u(t)$ with respect to $t$. The aim is to find the solution to the following Lagrange multiplier 
\[\frac{\{\int_0^1 u^2(t)\,dt\}^2}{\frac{4}{\tilde{c}^2}\int^1_{-1} \dot{u}^2(t) \, dt +1}-\lambda\left(\int_{-1}^1 u^2(t)\,dt-1\right)\]
Let $u_\varepsilon(t) = u(t) + \varepsilon \eta(t)$ be a functional perturbation of $u(t)$ with small $\varepsilon$ and $\eta$ is a differentiable function satisfying $\eta(1)=\eta(-1)=0$. By Euler–Lagrange equation, we have the following,
\begin{align*}
    &\frac{\partial}{\partial \varepsilon} \frac{\{\int_0^1 u_\varepsilon^2(t)\,dt\}^2}{\frac{4}{\tilde{c}^2}\int^1_{-1} \dot{u_\varepsilon}^2(t) \, dt +1}-\lambda\left(\int_{-1}^1 u_\varepsilon^2(t)\,dt-1\right)\bigg|_{\varepsilon=0}\\
    &\qquad= \frac{\partial}{\partial \varepsilon} \frac{[\int_0^1 \{u(t)+\varepsilon \eta(t)\}^2\,dt]^2}{\frac{4}{\tilde{c}^2}\int^1_{-1} \{\dot{u}(t)+\varepsilon \dot{\eta}(t)\}^2 \, dt +1} -\lambda\left(\int_{-1}^1 \{u(t)+\varepsilon \eta(t)\}^2\,dt-1\right)\bigg|_{\varepsilon=0}\\
    &\qquad=  \frac{\left(\frac{4}{\tilde{c}^2}\int^1_{-1} \{\dot{u}(t)+\varepsilon \dot{\eta}(t)\}^2 \, dt +1\right)\frac{\partial}{\partial \varepsilon}[\int_0^1 \{u(t)+\varepsilon \eta(t)\}^2\,dt]^2}{\left(\frac{4}{\tilde{c}^2}\int^1_{-1} \{\dot{u}(t)+\varepsilon \dot{\eta}(t)\}^2 \, dt +1\right)^2} \bigg|_{\varepsilon=0}\\
    &\qquad\qquad - \frac{[\int_0^1 \{u(t)+\varepsilon \eta(t)\}^2\,dt]^2\frac{\partial}{\partial \varepsilon}\left(\frac{4}{\tilde{c}^2}\int^1_{-1} \{\dot{u}(t)+\varepsilon \dot{\eta}(t)\}^2 \, dt +1\right)}{\left(\frac{4}{\tilde{c}^2}\int^1_{-1} \{\dot{u}(t)+\varepsilon \dot{\eta}(t)\}^2 \, dt +1\right)^2}\bigg|_{\varepsilon=0}\\
    &\qquad\qquad -\frac{\partial}{\partial \varepsilon}\lambda\left(\int_{-1}^1 \{u(t)+\varepsilon \eta(t)\}^2\,dt-1\right)\bigg|_{\varepsilon=0}\\
    &\qquad=\frac{4\int_0^1 u^2(t)\,dt \, \int_0^1u(t)\eta(t)\, dt}{\frac{4}{\tilde{c}^2}\int^1_{-1} \dot{u}^2(t) \, dt +1}- \frac{\{\int_0^1 u^2(t)\,dt\}^2\frac{8}{\tilde{c}^2}\int^1_{-1}\dot{u}(t)\dot{\eta}(t)\, dt}{\left(\frac{4}{\tilde{c}^2}\int^1_{-1} \dot{u}^2(t) \, dt +1\right)^2}-2\lambda\int_{-1}^1u(t)\eta(t)\, dt
    \end{align*}
    
    Now, we denote by $A=\int_0^1 u^2(t)\,dt$ and $B=\frac{4}{\tilde{c}^2}\int^1_{-1} \dot{u}^2(t) \, dt +1$ and the above display becomes 
    \begin{align*}
        &\frac{4\int_0^1 u^2(t)\,dt \, \int_0^1u(t)\eta(t)\, dt}{\frac{4}{\tilde{c}^2}\int^1_{-1} \dot{u}^2(t) \, dt +1}- \frac{\{\int_0^1 u^2(t)\,dt\}^2\frac{8}{\tilde{c}^2}\int^1_{-1}\dot{u}(t)\dot{\eta}(t)\, dt}{\left(\frac{4}{\tilde{c}^2}\int^1_{-1} \dot{u}^2(t) \, dt +1\right)^2}-2\lambda\int_{-1}^1u(t)\eta(t)\, dt \\
        &\qquad = \frac{4A}{B}\int_0^1u(t)\eta(t)\, dt- \frac{8A^2}{\tilde{c}^2B^2}\int^1_{-1}\dot{u}(t)\dot{\eta}(t)\, dt-2\lambda\int_{-1}^1u(t)\eta(t)\, dt\\
        &\qquad = \frac{2A}{B}\int_{-1}^1u(t)\eta(t)I(t \geq 0)\, dt- \frac{4A^2}{\tilde{c}^2B^2}\left(\dot{u}(t)\eta(t)\bigg|^1_{-1}-\int^1_{-1}\ddot{u}(t)\eta(t)\, dt\right)-\lambda\int_{-1}^1u(t)\eta(t)\, dt \\
        &\qquad = \int_{-1}^1\left(\frac{2A}{B} u(t)I(t\geq 0)+ \frac{4A^2}{\tilde{c}^2B^2}\ddot{u}(t)-\lambda u(t) \right) \eta(t)\, dt
    \end{align*}
Thus the resulting differentiable equation is 
\begin{align*}
    \begin{cases}
        \left(\frac{2A}{B}-\lambda\right) u(t)+ \frac{4A^2}{\tilde{c}^2B^2}\ddot{u}(t) = 0 \quad &\text{ when }\quad t \geq 0\\
         -\lambda u(t)+ \frac{4A^2}{\tilde{c}^2B^2}\ddot{u}(t) = 0\quad &\text{ when }\quad t < 0
    \end{cases}
\end{align*}

For a general case with $C_1, C_2 > 0$
\begin{align*}
    C_1 u(t) + C_2 \ddot{u}(t) = 0 \implies u(t) &= \cos\left(t\sqrt{C_1/C_2} \right) + \sin\left(t\sqrt{C_1/C_2} \right) \\
    \implies g(t) &= \left\{\cos\left(t\sqrt{C_1/C_2} \right) + \sin\left(t\sqrt{C_1/C_2} \right) \right\}^2
\end{align*}
\begin{align*}
    -C_1 u(t) + C_2 \ddot{u}(t) = 0 \implies u(t) &= \exp\left(t\sqrt{C_1/C_2}\right) + \exp\left(-t\sqrt{C_1/C_2} \right) \\
    \implies g(t) &= \left\{\exp\left(t\sqrt{C_1/C_2}\right) + \exp\left(-t\sqrt{C_1/C_2} \right) \right\}^2
\end{align*}

\newpage
\section{Setting up a differential equation}
For simplicity, we focus on a univariate case. Let $g:= \mathbb{R} \mapsto \mathbb{R}^+$ be an absolutely continuous density function whose support is contained in $(-1,1)$. The absolute continuity of $g$ over $\mathbb{R}$ implies that $g(1)=g(-1)=0$. 
We define Fisher information of $g$ as 
\begin{align*}
    \mathcal{J}(g) = \int_{-1}^1 \frac{\{g'(t)\}^2}{g(t)}I\{g(t)>0\}\,dt.
\end{align*}

For a given constant $c \geq 0$, our goal is to find $g$ that solves the following optimization
\[\sup_{g}\frac{\{\int_0^1 g(t)\,dt\}^2}{\frac{1}{c^2}\mathcal{J}(g)  +1} \quad \text{subject to}\quad \int_{-1}^1 g(t)\, dt = 1 \text{ and } \text{$g$ is abs. cont.}\]

We define $u^2(t) = g(t)$ and denote by $\dot{u}(t)$ the derivative of $u(t)$ with respect to $t$. The original problem can be formulated in terms of $u$ as folllws:

\[\sup_{u}\frac{\{\int_0^1 u^2(t)\,dt\}^2}{\frac{4}{c^2}\int_{-1}^1 \dot{u}(t)^2 \, dt +1} \quad \text{subject to}\quad \int_{-1}^1 u^2(t)\, dt = 1 \text{ and } \text{$u^2$ is abs. cont.}\]

Now we consider the following constrained optimization problem:
\[\sup_{a\in[0,1]}\sup_{u}\frac{a^2}{\frac{4}{c^2}\int_{-1}^1 \dot{u}(t)^2 \, dt +1} \quad \text{subject to}\quad \int_{-1}^1 u^2(t)\, dt = 1 \text{, } \text{$u^2$ is abs. cont.} \text{ and } \int_{0}^1u^2(t)\,dt = a\]

Once the numerator is fixed at $a$, the optima is attained by minimizing the denominator. We thus need to solve the simpler problem:
\begin{equation}
    \sup_{a\in[0,1]}\inf_{u}4\int_{-1}^1 \dot{u}(t)^2 \, dt \quad \text{subject to}\quad \int_{-1}^1 u^2(t)\, dt = 1 \text{, } \text{$u^2$ is abs. cont.} \text{ and } \int_{0}^1u^2(t)\,dt = a. \label{eq:opt}
\end{equation}

Since $u^2(t)$ must be integrate to one, we have $\int_{-1}^0u^2(t)\,dt = 1-a$. Furthermore, our constraints are equivalent to the following:

\begin{align*}
    \int_{-1}^0u^2(t)\,dt = 1-a &\Longleftrightarrow \int_{-1}^0\left(\frac{u(t)}{\sqrt{1-a}}\right)^2\,dt = 1\\
     \int_{0}^1u^2(t)\,dt = a &\Longleftrightarrow \int_{-1}^0\left(\frac{u(t)}{\sqrt{a}}\right)^2\,dt = 1
\end{align*}

By defining $\nu_1(t) := \frac{u(t)}{\sqrt{1-a}}$ and $\nu_2(t) := \frac{u(t)}{\sqrt{a}}$, the optimization problem becomes 

\begin{align*}
    4\inf_{u}\int_{-1}^1 \dot{u}(t)^2 \, dt &= 4\inf_{u}\left\{\int_{-1}^0 \dot{u}(t)^2 \, dt + \int_{0}^1\dot{u}(t)^2 \, dt\right\}\\
    &= 4\inf_{u}\left\{(1-a)\int_{-1}^0 \dot{\nu_1}(t)^2 \, dt + a\int_{0}^1\dot{\nu_2}(t)^2 \, dt\right\}
\end{align*}

If we \textit{pretend} we can solve the optimization separately, then finding $\nu_1$ and $\nu_2$ is \textit{almost} equivalent to finding two density functions that minimize Fisher information over compact supports. There are two major caveats:
\begin{enumerate}
    \item Previously known result (i.e., $\cos^2(\pi x/2)$ minimizes Fisher information) is for absolutely continuous density functions. This introduces a new constraint $\nu_1(0)=\nu_2(0)=0$ to the original problem. This means we are only optimizing over density functions $u$ such that $u(-1)=u(1)=u(0)=0$. 
    \item Both $\nu_1$ and $\nu_2$ depend on $u$ so we need to consider the optimization simultaneously. 
\end{enumerate}

If we take a leap of faith and consider two problems separately, we find the following $\nu_1$ and $\nu_2$ by the simple change of variable:
\begin{align*}
    \nu_1^2(t) &= 2\cos^2\left(\frac{\pi (t+1)}{2}\right)I(-1\leq t \leq 0)\\
    \nu_2^2(t) &= 2\cos^2\left(\frac{\pi (t-1)}{2}\right)I(0\leq t \leq 1)
\end{align*}
The resulting function $u$ is given by 
\begin{align*}
    u(t) &= \sqrt{1-a}\nu_1(t) + \sqrt{a}\nu_2(t) \\
    &= \sqrt{2}\left\{\sqrt{1-a}\cos\left(\frac{\pi (t+1)}{2}\right)I(-1\leq t \leq 0)+\sqrt{a}\cos\left(\frac{\pi (t-1)}{2}\right)I(0\leq t \leq 1)\right\}
\end{align*}

Because we have indicators $I(-1\leq t \leq 0)$ and $I(0\leq t \leq 1)$, the resulting density function $g$ is given by 
\[g(t) = u^2(t) = 2\left\{(1-a)\cos^2\left(\frac{\pi (t+1)}{2}\right)I(-1\leq t \leq 0)+a\cos^2\left(\frac{\pi (t-1)}{2}\right)I(0\leq t \leq 1)\right\}\]
\begin{figure}[h]
     \centering
     \begin{subfigure}{0.7\textwidth}
         \centering
         \includegraphics[width=\textwidth]{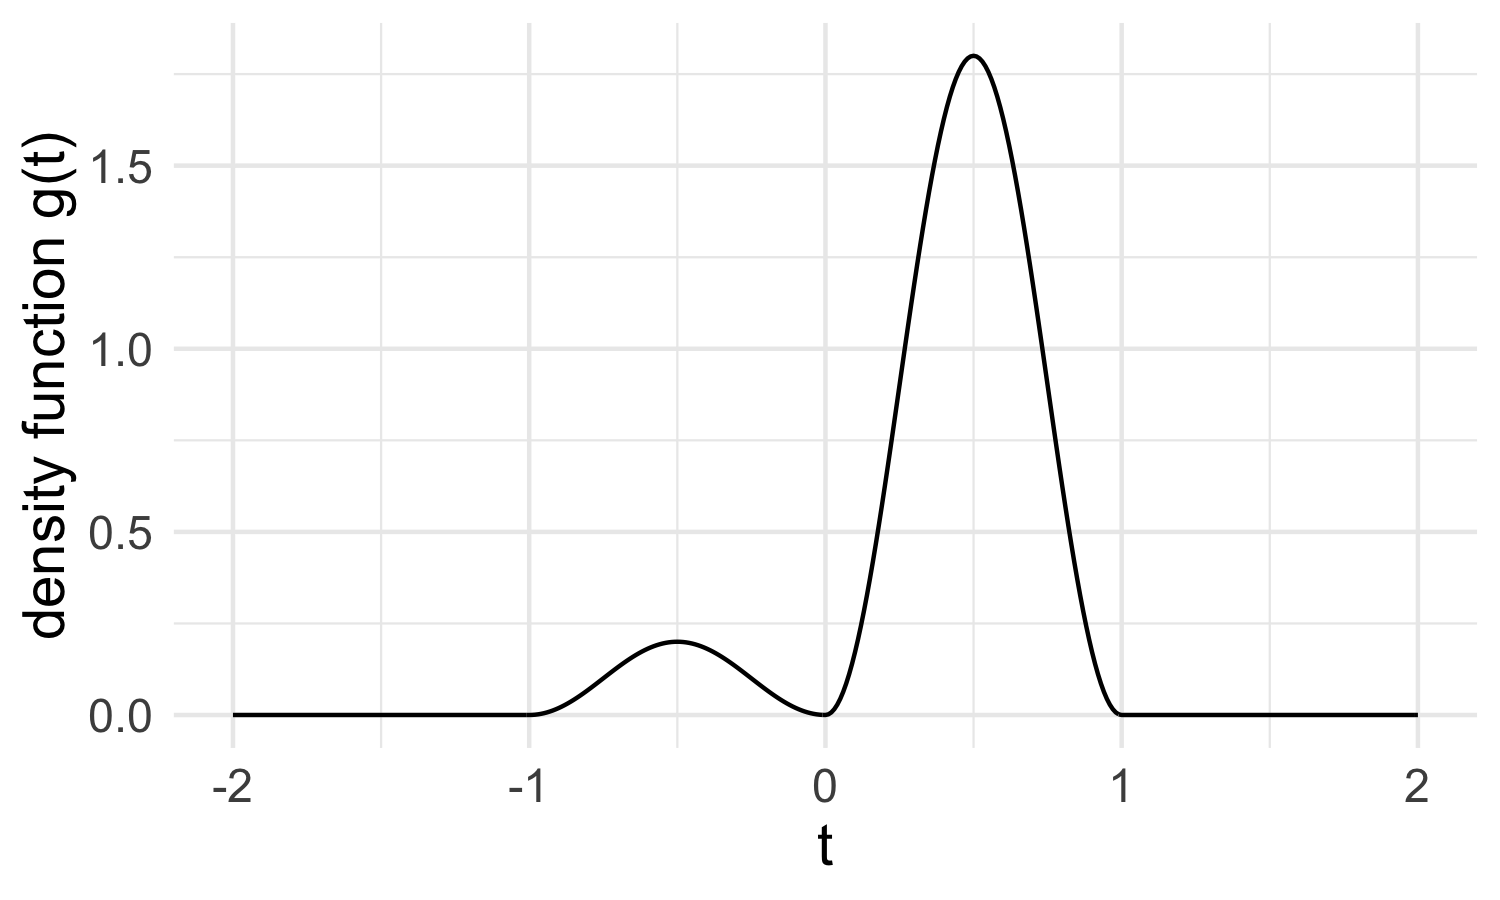}
         \label{fig:y equals x}
     \end{subfigure}
     \caption{An example of $g(t)$ when $a=0.9$}
\end{figure}

Finally, we can compute Fisher information of $g$ as follows:
\begin{align*}
    \mathcal{J}(g) &= \int_{-1}^1 \frac{\{g'(t)\}^2}{g(t)}I\{g(t)>0\}\,dt \\
    &=\int_{-1}^0 \frac{\{g'(t)\}^2}{g(t)}I\{g(t)>0\}\,dt + \int_{0}^1 \frac{\{g'(t)\}^2}{g(t)}I\{g(t)>0\}\,dt \\
    &= (1-a)\int_{-1}^0 \frac{\left\{\tfrac{d}{dt} 2\cos^2\left(\frac{\pi (t+1)}{2}\right) \right\}^2}{2\cos^2\left(\frac{\pi (t+1)}{2}\right)}\,dt + a\int_{0}^1 \frac{\left\{\tfrac{d}{dt} 2\cos^2\left(\frac{\pi (t-1)}{2}\right) \right\}^2}{2\cos^2\left(\frac{\pi (t-1)}{2}\right)}\,dt \\
    &= \pi^2.
\end{align*}
Since Fisher information does not depend on $a$, we can trivially maximize the objective by setting $a=1$. This is not an optimal solution since I know (based on simulation) that the location-scale family of $\cos^2(\cdot)$ can attain better optima depending on the value of $c$. Back to the drawing board...

\newpage
\section{One more try}
For each $a\in[0, 1]$, we need to solve the problem:
\[
\inf_u \int_{-1}^1 \dot{u}^2(t)dt,\mbox{ subject to }\int_{-1}^1 u^2(t)dt = 1, u^2\mbox{ abs. cont. and }\int_0^1 u^2(t)dt = a.
\]
In the original density form, this problem is
\[
\inf_g\int_{-1}^1 \frac{(g'(t))^2}{g(t)}dt,\mbox{ subject to }\int_{-1}^1 g(t)dt = 1, g\mbox{ abs. cont. and }\int_0^1 g(dt) = a.
\]

Theorem 2.1 of~\cite{ernst2017minimizing} implies that the minimizing $g$ satisfies
\[
-2\dot{\nu}(x) - \nu^2(x) = B_1\mathbf{1}\{-1 \le x \le 0\} + B_2\mathbf{1}\{0 \le x\le 1\}.
\]
where $\nu(t) = g'(t)/g(t)$. The general solution of the first-order non-homogeneous ODE is given by 
\begin{align*}
    \nu(x) = \begin{cases}
        \sqrt{B_1}\tan\left(\frac{\sqrt{B_1}}{2}(c_1-x)\right) & \text{where } -1 \le x \le 0\\
        \sqrt{B_2}\tan\left(\frac{\sqrt{B_2}}{2}(c_2-x)\right) & \text{where } 0 \le x \le 1
    \end{cases}
\end{align*}
\kt{Sanity check}
\begin{align*}
    \nu'(x) &= -\sqrt{B_1}\sec^2\left(\frac{\sqrt{B_1}}{2}(c_1-x)\right)\frac{\sqrt{B_1}}{2}\\
    -2\nu'(x) &= B_1\sec^2\left(\frac{\sqrt{B_1}}{2}(c_1-x)\right) \\
    \nu^2(x) &= B_1\tan^2\left(\frac{\sqrt{B_1}}{2}(c_1-x)\right)=B_1 \left(\sec^2\left(\frac{\sqrt{B_1}}{2}(c_1-x)\right) - 1\right)
\end{align*}
\kt{End sanity check}

By definition, the function $\nu(t) = g'(t)/g(t)$.
\begin{align*}
    g'(x)/g(x) = \begin{cases}
        \sqrt{B_1}\tan\left(\frac{\sqrt{B_1}}{2}(c_1-x)\right) & \text{where } -1 \le x \le 0\\
        \sqrt{B_2}\tan\left(\frac{\sqrt{B_2}}{2}(c_2-x)\right) & \text{where } 0 \le x \le 1
    \end{cases}
\end{align*}
The general solution $g$ is given by 
\begin{align*}
    g(x) = \begin{cases}
        \widetilde{C_1}\cos^2\left(\frac{\sqrt{B_1}}{2}(x-c_1)\right) & \text{where } -1 \le x \le 0\\
        \widetilde{C_2}\cos^2\left(\frac{\sqrt{B_2}}{2}(x-c_2)\right) & \text{where } 0 \le x \le 1
    \end{cases}
\end{align*}
\kt{At least this suggests we should focus on the mixture of location-scale family of $\cos^2$ priors. I think we need to explore different boundaries.}

\kt{Sanity check}
\begin{align*}
    g'(x) &= -\widetilde{C_1}\sqrt{B_1}\cos\left(\frac{\sqrt{B_1}}{2}(x-c_1)\right)\sin\left(\frac{\sqrt{B_1}}{2}(x-c_1)\right)\\
    \frac{g'(x)}{g(x)} &= \frac{-\widetilde{C_1}\sqrt{B_1}\cos\left(\frac{\sqrt{B_1}}{2}(x-c_1)\right)\sin\left(\frac{\sqrt{B_1}}{2}(x-c_1)\right)}{\widetilde{C_1}\cos^2\left(\frac{\sqrt{B_1}}{2}(x-c_1)\right)}\\
    &= -\sqrt{B_1}\frac{\sin\left(\frac{\sqrt{B_1}}{2}(x-c_1)\right)}{\cos\left(\frac{\sqrt{B_1}}{2}(x-c_1)\right)}\\
    &=-\sqrt{B_1}\tan\left(\frac{\sqrt{B_1}}{2}(x-c_1)\right)\\
    &=\sqrt{B_1}\tan\left(\frac{\sqrt{B_1}}{2}(c_1-x)\right)
\end{align*}
\kt{End sanity check}

It now remains to solve the initial value problem. First, the resulting density $g$ needs to be continuous at zero. This gives us the following
\begin{align*}
    \lim_{x\to0^-}g(x) = \widetilde{C_1}\cos^2\left(\frac{-c_1\sqrt{B_1}}{2}\right),\,
    \lim_{x\to0^+}g(x) = \widetilde{C_2}\cos^2\left(\frac{-c_2\sqrt{B_2}}{2}\right)
\end{align*}
\begin{equation}
    \widetilde{C_1}\cos^2\left(\frac{-c_1\sqrt{B_1}}{2}\right) = \widetilde{C_2}\cos^2\left(\frac{-c_2\sqrt{B_2}}{2}\right)\label{eq:g(0)=g(0)}
\end{equation}
Since $g(1)=g(-1)=0$ and its derivatives must be zero on boundary, (\kt{we may need to generalize this to $1\le a_- \le 0 \le a_+ \le 1$}), we have 
\begin{align*}
    \lim_{x\to-1}g(x) = \widetilde{C_1}\cos^2\left(\frac{-\sqrt{B_1}(c_1+1)}{2}\right),\,
    \lim_{x\to1}g(x) = \widetilde{C_2}\cos^2\left(\frac{-\sqrt{B_2}(c_2+1)}{2}\right)
\end{align*}
Since $\cos(\cdot)$ is zero at $\pm \frac{k\pi}{2}$ for all odd $k$, 
\begin{align}
    \sqrt{B_1}(c_1+1) = k_1\pi, \, \sqrt{B_2}(c_2+1) = k_2\pi\nonumber
\end{align}
or equivalently,
\begin{align}
    c_1 = \frac{k_1\pi}{\sqrt{B_1}}-1, \,  
    c_2 = \frac{k_2\pi}{\sqrt{B_2}}-1\label{eq:c1c2}
\end{align}
For such values of $\sqrt{B_1}(c_1+1)$ and $\sqrt{B_2}(c_2+1)$ the derivatives of $g(x)$ on boundaries are zero. Combining \eqref{eq:g(0)=g(0)} and \eqref{eq:c1c2}, we have
\begin{align}
    \widetilde{C_1}\cos^2\left(\frac{\sqrt{B_1}}{2}-\frac{k_1\pi}{2}\right) &= \widetilde{C_2}\cos^2\left(\frac{\sqrt{B_2}}{2}-\frac{k_2\pi}{2}\right)\nonumber\\
    \implies\widetilde{C_1}\sin^2\left(\frac{\sqrt{B_1}}{2}\right) &= \widetilde{C_2}\sin^2\left(\frac{\sqrt{B_2}}{2}\right)
\end{align}

We have constraints $\int_{-1}^0g(t)\, dt = 1-a$ and $\int_{0}^1g(t)\, dt = a$ as follows:
\begin{align*}
    \widetilde{C_1}\int_{-1}^0 \cos^2\left(\frac{\sqrt{B_1}(t-c_1)}{2}\right)\, dt &= \widetilde{C_1}\int_{-1}^0 \cos^2\left(\frac{\sqrt{B_1}t}{2}-\frac{k_1\pi}{2}+\frac{\sqrt{B_1}}{2}\right)\, dt\\
    &=\widetilde{C_1}\int_{-1}^0 \sin^2\left(\frac{\sqrt{B_1}}{2}(t+1)\right)\, dt\\
    &= \frac{\widetilde{C_1}}{2}\int_{-1}^0 1-\cos(\sqrt{B_1}(t+1))\, dt\\
    &= \frac{\widetilde{C_1}}{2}-\frac{\widetilde{C_1}}{2}\int_{-1}^0\cos(\sqrt{B_1}(t+1))\, dt\\
    &= \frac{\widetilde{C_1}}{2}-\frac{\widetilde{C_1}}{2\sqrt{B_1}}\int_0^{\sqrt{B_1}} \cos(u)\, du\\
    &= \frac{\widetilde{C_1}}{2}-\frac{\widetilde{C_1}}{2\sqrt{B_1}}\sin(\sqrt{B_1}) 
\end{align*}

\begin{align*}
    \widetilde{C_2}\int_{0}^1 \cos^2\left(\frac{\sqrt{B_2}(t-c_2)}{2}\right)\, dt &= \widetilde{C_2}\int_{0}^1 \cos^2\left(\frac{\sqrt{B_2}t}{2}-\frac{k_2\pi}{2}+\frac{\sqrt{B_2}}{2}\right)\, dt\\
    &=\widetilde{C_2}\int_{0}^1 \sin^2\left(\frac{\sqrt{B_2}}{2}(t+1)\right)\, dt\\
    &= \frac{\widetilde{C_2}}{2}\int_{0}^1 1-\cos(\sqrt{B_2}(t+1))\, dt\\
    &= \frac{\widetilde{C_2}}{2}-\frac{\widetilde{C_2}}{2}\int_{0}^1\cos(\sqrt{B_2}(t+1))\, dt\\
    &= \frac{\widetilde{C_2}}{2}-\frac{\widetilde{C_2}}{2\sqrt{B_2}}\int_{\sqrt{B_2}}^{2\sqrt{B_2}} \cos(u)\, du\\
    &= \frac{\widetilde{C_2}}{2}-\frac{\widetilde{C_2}}{2\sqrt{B_2}}\sin(2\sqrt{B_2})+\frac{\widetilde{C_2}}{2\sqrt{B_2}}\sin(\sqrt{B_2}) 
\end{align*}

\begin{align}
    \frac{\widetilde{C_1}}{2}-\frac{\widetilde{C_1}}{2\sqrt{B_1}}\sin(\sqrt{B_1}) =1-a\\
    \frac{\widetilde{C_2}}{2}-\frac{\widetilde{C_2}}{2\sqrt{B_2}}\sin(2\sqrt{B_2})+\frac{\widetilde{C_2}}{2\sqrt{B_2}}\sin(\sqrt{B_2}) =a
\end{align}

\kt{I think the initial value problem is under-specified. If we add another constraint to assume the density is continuously differentiable at zero, we also have the following}
\begin{align*}
    \lim_{x\to0^-}g'(x) &=  -\widetilde{C_1}\sqrt{B_1}\cos\left(-\frac{\sqrt{B_1}}{2}c_1\right)\sin\left(-\frac{\sqrt{B_1}}{2}c_1\right)\\
    &=-\widetilde{C_1}\sqrt{B_1}\cos\left(\frac{\sqrt{B_1}}{2}-\frac{k_1\pi}{2}\right)\sin\left(\frac{\sqrt{B_1}}{2}-\frac{k_1\pi}{2}\right)\\
    &= \widetilde{C_1}\sqrt{B_1}\sin\left(\frac{\sqrt{B_1}}{2}\right)\cos\left(\frac{\sqrt{B_1}}{2}\right)\\
     &= \widetilde{C_1}\sqrt{B_1}\sin\left(\frac{\sqrt{B_1}}{2}\right)\cos\left(\frac{\sqrt{B_1}}{2}\right)\\
     &= \frac{\widetilde{C_1}\sqrt{B_1}}{2}\sin\left(\sqrt{B_1}\right)
\end{align*}
By symmetry, we get the following constraints
\begin{align}
   \widetilde{C_1}\sqrt{B_1}\sin\left(\sqrt{B_1}\right) = \widetilde{C_2}\sqrt{B_2}\sin\left(\sqrt{B_2}\right)
\end{align}

We now have four equations;
\begin{align}
\widetilde{C_1}\sin^2\left(\frac{\sqrt{B_1}}{2}\right) &= \widetilde{C_2}\sin^2\left(\frac{\sqrt{B_2}}{2}\right)\\
\widetilde{C_1}\sqrt{B_1}\sin\left(\sqrt{B_1}\right) &= \widetilde{C_2}\sqrt{B_2}\sin\left(\sqrt{B_2}\right)\\
\frac{1}{\sqrt{B_1}}\sin(\sqrt{B_1}) &=1-\frac{2-2a}{\widetilde{C_1}}\\
    \frac{1}{\sqrt{B_2}}\sin(2\sqrt{B_2})-\frac{1}{\sqrt{B_2}}\sin(\sqrt{B_2}) &=1-\frac{2a}{\widetilde{C_2}}
\end{align} 
Combining the first two conditions to eliminated $\widetilde{C_1}$, we get
\[\sqrt{B_2}\sin\left(\sqrt{B_2}\right)\sin^2\left(\frac{\sqrt{B_1}}{2}\right) = \sqrt{B_1}\sin\left(\sqrt{B_1}\right)\sin^2\left(\frac{\sqrt{B_2}}{2}\right)\]
\newpage

The general solution $g$ is given by 
\begin{align*}
    g(x) = \begin{cases}
        \widetilde{C_1}\cos^2\left(\frac{\sqrt{B_1}}{2}(x-c_1)\right) & \text{where } -1 \le x \le 0\\
        \widetilde{C_2}\cos^2\left(\frac{\sqrt{B_2}}{2}(x-c_2)\right) & \text{where } 0 \le x \le 1.
    \end{cases}
\end{align*}
Consider the case when the support of $g$ is given by $[\delta_{-}, \delta_{+}] \subseteq [-1,1]$ and $\delta_{-} \le 0 \le \delta_{+}$.
\begin{enumerate}
    \item Since $g(\delta_{-})=0$, we have
    \begin{equation}
        \widetilde{C_1}\cos^2\left(\frac{\sqrt{B_1}}{2}(\delta_{-}-c_1)\right)=0 \implies \sqrt{B_1}(\delta_{-}-c_1)=\pm\pi
    \end{equation}
    Similarly  $g(\delta_{+})=0$ gives
        \begin{equation}
        \widetilde{C_2}\cos^2\left(\frac{\sqrt{B_2}}{2}(\delta_{+}-c_2)\right)=0 \implies \sqrt{B_2}(\delta_{+}-c_2)=\pm\pi
    \end{equation}
    \item Since $g$ is absolutely continuous, we have
    \begin{align}
        \widetilde{C_1}\cos^2\left(-\frac{c_1\sqrt{B_1}}{2}\right)= \widetilde{C_2}\cos^2\left(-c_2\frac{\sqrt{B_2}}{2}\right)
    \end{align}
    \item By the constraint $\int_0^1 g(t)\, dt =a$, we have
    \begin{align}
     \widetilde{C_1}\int_{\delta_{-}}^0\cos^2\left(\frac{\sqrt{B_1}}{2}(x-c_1)\right) \, dt = -\frac{\widetilde{C_1}\delta_{-}}{2} + \frac{\widetilde{C_1}}{2\sqrt{B_1}}\sin(-c_1\sqrt{B_1})=a
    \end{align}
    Similarly we have
    \begin{align}
     \widetilde{C_2}\int_{0}^{\delta_+}\cos^2\left(\frac{\sqrt{B_2}}{2}(x-c_2)\right) \, dt = \frac{\widetilde{C_2}\delta_{+}}{2} - \frac{\widetilde{C_2}}{2\sqrt{B_2}}\sin(-c_2\sqrt{B_2})=1-a
    \end{align}
\end{enumerate}

Next, we compute Fisher information of $g$. It follows that 
\begin{align}
    \frac{\{g'(x)\}^2}{g(x)} &= \frac{B_1\widetilde{C_1}^2\cos^2\left(\frac{\sqrt{B_1}}{2}(x-c_1)\right)\sin^2\left(\frac{\sqrt{B_1}}{2}(x-c_1)\right)}{\widetilde{C_1}\cos^2\left(\frac{\sqrt{B_1}}{2}(x-c_1)\right)}\nonumber\\
    &= B_1\widetilde{C_1}\sin^2\left(\frac{\sqrt{B_1}}{2}(x-c_1)\right)\nonumber
\end{align}
for $\delta_{-}\le x \le 0$. We thus have
\begin{align}
    \mathcal{J}(g) &= B_1\widetilde{C_1}\int_{\delta_{-}}^0  \sin^2\left(\frac{\sqrt{B_1}}{2}(x-c_1)\right)\, dx + B_2\widetilde{C_2}\int_0^{\delta_{+}} \sin^2\left(\frac{\sqrt{B_2}}{2}(x-c_2)\right)\, dx \nonumber \\
    &=-\frac{B_1\widetilde{C_1}}{2}\delta_{-} - \frac{\sqrt{B_1}\widetilde{C_1}}{2}\sin(-\sqrt{B_1}c_1)+\frac{B_2\widetilde{C_2}}{2}\delta_{+} + \frac{\sqrt{B_2}\widetilde{C_2}}{2}\sin(-\sqrt{B_2}c_2)
\end{align}

\kt{Sanity check}

The standard cosine prior corresponds to the case when $\widetilde{C_1}=\widetilde{C_2}=1$, $c_1=c_2=0$, $B_1=B_2=\pi^2$, $\delta_{-}=-1$ and $\delta_{+}=1$. Fisher information for this prior is $\pi^2$.

\kt{End sanity check}

\begin{align}
    -\frac{B_1\widetilde{C_1}\delta_{-}}{2} + \frac{\widetilde{C_1}\sqrt{B_1}}{2}\sin(-c_1\sqrt{B_1})=B_1a\\
    \frac{B_2\widetilde{C_2}\delta_{+}}{2} - \frac{\sqrt{B_2}\widetilde{C_2}}{2}\sin(-c_2\sqrt{B_2})=B_2(1-a)
\end{align}
Fisher information of $g$ in a general form is given by
\begin{align}
     \mathcal{J}(g) &=-B_1\widetilde{C_1}\delta_{-} - B_1a+B_2\widetilde{C_2}\delta_{+} -B_2(1-a).
\end{align}
Two conditions (12) and (13) gives us 
\[c_1=\delta_{-}\pm\pi/\sqrt{B_1}\quad\text{and}\quad c_2=\delta_{+}\pm\pi/\sqrt{B_2}.\]
Plugging them into (14), we obtain
    \begin{align}
        \widetilde{C_1}\sin^2\left(-\frac{\delta_{-}\sqrt{B_1}}{2}\right)= \widetilde{C_2}\sin^2\left(-\frac{\delta_{+}\sqrt{B_2}}{2}\right).
    \end{align}
By the constraint $\int_0^1 g(t)\, dt =a$, we have
\begin{align}
    -\frac{\widetilde{C_1}\delta_{-}}{2} - \frac{\widetilde{C_1}}{2\sqrt{B_1}}\sin(\delta_{-}\sqrt{B_1})=1-a
\end{align}
Similarly we have
\begin{align}
    \frac{\widetilde{C_2}\delta_{+}}{2} + \frac{\widetilde{C_2}}{2\sqrt{B_2}}\sin(\delta_{+}\sqrt{B_2})=a
\end{align}
Continuous derivative at zero gives
\[\sqrt{B_1}\widetilde{C_1}\sin(\delta_{-}\sqrt{B_1})=\sqrt{B_2}\widetilde{C_2}\sin(\delta_{+}\sqrt{B_2})\]
Combining this result, we get
\begin{align}
    -\widetilde{C_1}\delta_{-} - \frac{\widetilde{C_1}}{\sqrt{B_1}}\sin(\delta_{-}\sqrt{B_1})=2-2a\\
    \widetilde{C_2}\delta_{+} + \frac{\sqrt{B_1}}{B_2}\widetilde{C_1}\sin(\delta_{-}\sqrt{B_1})=2a\\
    \implies -\widetilde{C_1}\delta_{-} + \frac{B_2\widetilde{C_2}\delta_{+}}{B_1}+2a\left(1-\frac{B_2}{B_1}\right)=2\\
    \implies (\widetilde{C_2}\delta_{+}-\widetilde{C_1}\delta_{-}) -\widetilde{C_2}\delta_{+}\left(1-\frac{B_2}{B_1}\right)+2a\left(1-\frac{B_2}{B_1}\right)=2\\
    \implies (\widetilde{C_2}\delta_{+}-\widetilde{C_1}\delta_{-}) +(2a-\widetilde{C_2}\delta_{+})\left(1-\frac{B_2}{B_1}\right)=2
\end{align}
