# Supplementary material for: Generalized van Trees inequality: Local minimax bounds for non-smooth functionals and irregular statistical models
Source: arXiv:2405.06437 source file (2024-10-19)
Supplement: Supplementary file 3 [file hellinger.tex]

\clearpage
\section{QMD and Fisher information}

\begin{definition}[Differentiable in quadratic mean] The statistical model $\{P_t : t \in \Theta\}$ is differentiable in quadratic mean at $\theta \in \Theta$
if there exists a real-valued function $\dot{\ell}_{\theta} \in L_2(\mu)$ such that 

We then define the Fisher information $\mathcal{I}(\theta)$ of the model at $\theta$ as 
\begin{align}
    \mathcal{I}(\theta) \coloneqq \int_{\mathcal{X}} \dot{\ell}_{\theta}\dot{\ell}_{\theta}^Tp_{\theta}\, d\mu
\end{align}
\end{definition}
\subsection{The connection to absolute continuity of the density function}
Here we restate the result by \citet{pollardAsymptotia, gassiat2013revisiting}. 
\begin{lemma}
\begin{align*}
    \dot{\ell}_{\theta} = \left(\nabla p_{\theta}/p^{1/2}_{\theta}\right)I(p_{\theta} > 0)
\end{align*}
and this implies that 
\begin{align*}
    \mathcal{I}(\theta) = \int_{\mathcal{X}}\frac{\nabla p_{\theta}\nabla p^T_{\theta}}{p_{\theta}}I(p_{\theta} > 0)\, d\mu 
\end{align*}
\end{lemma}
\subsection{The local limit of squared Hellinger divergence}
The following result is presented for an expositional purpose (it is trivial) and \cite{lin2019optimal} uses as the definition of regularity.
\begin{lemma}\label{lm:local_limit_H2}
Let $h$ be a fixed vector in $\Theta$ and $\varepsilon_n$ be an arbitrary convergent sequence such that $\varepsilon_n \to 0$. If a statistical model $P_\theta$ is Hellinger differentiable or differentiable in quadratic mean at $\theta_0$, then it implies
\begin{align*}
    \lim_{\varepsilon_n\to 0}\varepsilon_n^{-2} H^2(P_{\theta_0+h\varepsilon_n}, P_{\theta_0}) =\frac{1}{4} h^T\mathcal{I}(\theta_0)h.
\end{align*}
\end{lemma}
\begin{proof}
The proof is analogous under two types of differentiablity. Quadratic mean differentiability directly implies that
\begin{align}
     \lim_{\varepsilon_n\to0}\varepsilon_n^{-2}H^2(P_{\theta_0+h\varepsilon_n}, P_{\theta_0}) &=\lim_{\varepsilon_n\to0}\varepsilon_n^{-2}\int \left(p_{\theta_0+h\varepsilon_n}^{1/2} - p_{\theta_0}^{1/2} \right)^2\, d\mu \nonumber \\
     &=\lim_{\varepsilon_n\to0}\varepsilon_n^{-2}\left\{\int \left( \frac{1}{2}h^T\varepsilon_n\dot{s}_{\theta_0}p_{\theta_0}^{1/2}\right)^2\, d\mu + o(|\varepsilon_n|^2)\right\}\nonumber\\
     &=\frac{1}{4} h^T\mathcal{I}(\theta_0)h \nonumber.
\end{align}
Therefore, a statistical model has well-defined Fisher information (i.e. it is regular) if the squared Hellinger distance is locally quadratic in $\varepsilon_n$.
\end{proof}
