# Supplementary material for: Generalized van Trees inequality: Local minimax bounds for non-smooth functionals and irregular statistical models
Source: arXiv:2405.06437 source file (2024-10-19)
Supplement: Supplementary file 4 [file hellinger_lowerbound.tex]

\newpage
\section{Attempts for deriving a tighter lower bound with Hellinger distance}
\subsection{Attempt 1}
We begin with the following inequality from Cauchy-Schwarz:
\begin{align}
    |\E_{\theta_1}T-\E_{\theta_2}T|^2 &\leq \int(T(x)-c)^2\left(p^{1/2}_{\theta_1}+p^{1/2}_{\theta_2}\right)^2\, d\mu (x)\,  H^2(P_{\theta_1}, P_{\theta_2})
\end{align}
for any $c$ and 
\[H^2(P_{\theta_1}, P_{\theta_2}) = \int \left(p^{1/2}_{\theta_1}-p^{1/2}_{\theta_2}\right)^2\, d\mu (x).\]
The optimal $c$ to minimize the RHS is given by 
\[c_* := \frac{\int T(x)\left(p^{1/2}_{\theta_1}+p^{1/2}_{\theta_2}\right)^2\, d\mu(x)}{\int\left(p^{1/2}_{\theta_1}+p^{1/2}_{\theta_2}\right)^2\, d\mu(x)}.\]
We then obtain that
\begin{align*}
    &|\E_{\theta_1}T-\E_{\theta_2}T|^2 \\
    &\qquad\leq\int T^2(x)\left(p^{1/2}_{\theta_1}+p^{1/2}_{\theta_2}\right)^2\, d\mu(x) - \frac{\left\{\int T(x)\left(p^{1/2}_{\theta_1}+p^{1/2}_{\theta_2}\right)^2\, d\mu(x)\right\}^2}{\int \left(p^{1/2}_{\theta_1}+p^{1/2}_{\theta_2}\right)^2\, d\mu(x)}\\
    &\qquad = \E_{\theta_1}T^2+\E_{\theta_2}T^2+2\int T^2(x)\left(p_{\theta_1}p_{\theta_2}\right)^{1/2} \, d\mu(x)-\frac{\left\{\E_{\theta_1}T+\E_{\theta_2}T+2\int T(x)\left(p_{\theta_1}p_{\theta_2}\right)^{1/2} \, d\mu(x)\right\}^2}{4-H^2(P_{\theta_1}, P_{\theta_2})}
\end{align*}
\kt{Here, we want to find the upper bound for $\int T^2(x)\left(p_{\theta_1}p_{\theta_2}\right)^{1/2} \, d\mu(x)$.}
Let $A := \{x : p_{\theta_1}(x) \geq p_{\theta_2}(x)\}$. Then we have 
\begin{align*}
    \int T^2(x)\left(p_{\theta_1}p_{\theta_2}\right)^{1/2} \, d\mu(x) \leq \int_AT^2(x)p_{\theta_1}\, d\mu(x) + \int_{A^c}T^2(x)p_{\theta_2}\, d\mu(x)
\end{align*}
\kt{It is also challenging to deal with $\int T(x)\left(p_{\theta_1}p_{\theta_2}\right)^{1/2} \, d\mu(x)$ since we don't know if $T(x) \geq 0$}

\subsection{Attempt 2}
We can proceed without plugging in the optimal $c$. We then have
\begin{align*}
    |\E_{\theta_1}T-\E_{\theta_2}T|^2 &\leq \int(T(x)-c)^2\left(p^{1/2}_{\theta_1}+p^{1/2}_{\theta_2}\right)^2\, d\mu (x)\,  H^2(P_{\theta_1}, P_{\theta_2}) \\
    &= \left\{\E_{\theta_1}(T(x)-c)^2 + \E_{\theta_2}(T(x)-c)^2+2\int (T(x)-c)^2\left(p_{\theta_1}p_{\theta_2}\right)^{1/2}\, d\mu (x)\right\}  H^2(P_{\theta_1}, P_{\theta_2})
\end{align*}
Since $(T(x)-c)^2 \geq 0$, we can bound the third term as follows:
\begin{align*}
    \int (T(x)-c)^2\left(p_{\theta_1}p_{\theta_2}\right)^{1/2} \, d\mu(x) \leq \int_A(T(x)-c)^2p_{\theta_1}\, d\mu(x) + \int_{A^c}(T(x)-c)^2p_{\theta_2}\, d\mu(x)
\end{align*}

\subsection{Attempt 3}
We can instead begin with the following:
\begin{align}
    |\E_{\theta_1}T-\E_{\theta_2}T|^2 &\leq \int(T(x)-c)^2\left(p^{1/2}_{\theta_1}-p^{1/2}_{\theta_2}\right)^2\, d\mu (x)\,  \left(4-H^2(P_{\theta_1}, P_{\theta_2})\right)
\end{align}
for any $c$. The optimal $c$ to minimize the RHS is given by 
\[c_* := \frac{\int T(x)\left(p^{1/2}_{\theta_1}-p^{1/2}_{\theta_2}\right)^2\, d\mu(x)}{\int\left(p^{1/2}_{\theta_1}-p^{1/2}_{\theta_2}\right)^2\, d\mu(x)}.\]
We then obtain
\begin{align*}
    &\int T^2(x)\left(p^{1/2}_{\theta_1}-p^{1/2}_{\theta_2}\right)^2\, d\mu(x) - \frac{\left\{\int T(x)\left(p^{1/2}_{\theta_1}-p^{1/2}_{\theta_2}\right)^2\, d\mu(x)\right\}^2}{\int \left(p^{1/2}_{\theta_1}-p^{1/2}_{\theta_2}\right)^2\, d\mu(x)}\\
    &\qquad = \E_{\theta_1}T^2+\E_{\theta_2}T^2-2\int T^2(x)\left(p_{\theta_1}p_{\theta_2}\right)^{1/2} \, d\mu(x)-\frac{\left\{\E_{\theta_1}T+\E_{\theta_2}T-2\int T(x)\left(p_{\theta_1}p_{\theta_2}\right)^{1/2} \, d\mu(x)\right\}^2}{H^2(P_{\theta_1}, P_{\theta_2})}
\end{align*}
Using trivial lower bound of $\int T^2(x)\left(p_{\theta_1}p_{\theta_2}\right)^{1/2} \, d\mu(x) \geq0$,  we get
\begin{align*}
    &\E_{\theta_1}T^2+\E_{\theta_2}T^2-2\int T^2(x)\left(p_{\theta_1}p_{\theta_2}\right)^{1/2} \, d\mu(x)-\frac{\left\{\E_{\theta_1}T+\E_{\theta_2}T-2\int T(x)\left(p_{\theta_1}p_{\theta_2}\right)^{1/2} \, d\mu(x)\right\}^2}{H^2(P_{\theta_1}, P_{\theta_2})}\\
    &\qquad\leq \E_{\theta_1}T^2+\E_{\theta_2}T^2-\frac{\left\{\E_{\theta_1}T+\E_{\theta_2}T-2\int T(x)\left(p_{\theta_1}p_{\theta_2}\right)^{1/2} \, d\mu(x)\right\}^2}{H^2(P_{\theta_1}, P_{\theta_2})}
\end{align*}
\kt{As above, it is challenging to deal with $\int T(x)\left(p_{\theta_1}p_{\theta_2}\right)^{1/2} \, d\mu(x)$ since we don't know if $T(x) \geq 0$}

\subsection{Attempt 4}
If we don't optimize for $c$, we get
\begin{align*}
    &|\E_{\theta_1}T-\E_{\theta_2}T|^2 \\
    &\qquad\leq \int(T(x)-c)^2\left(p^{1/2}_{\theta_1}-p^{1/2}_{\theta_2}\right)^2\, d\mu (x)\,  \left(4-H^2(P_{\theta_1}, P_{\theta_2})\right)\\
    &\qquad\leq \int(T(x)-c)^2\left(p_{\theta_1}+p_{\theta_2}\right)\, d\mu (x)\,  \left(4-H^2(P_{\theta_1}, P_{\theta_2})\right)\\
    &\qquad= \left\{\E_{\theta_1}(T(x)-c)^2+\E_{\theta_2}(T(x)-c)^2\right\}  \left(4-H^2(P_{\theta_1}, P_{\theta_2})\right)\\
    &\qquad= \left\{\text{Var}_{\theta_1}T+(\E_{\theta_1}T-c)^2+\text{Var}_{\theta_2}T+(\E_{\theta_2}T-c)^2\right\}  \left(4-H^2(P_{\theta_1}, P_{\theta_2})\right)\\
    &\qquad= \left\{\E_{\theta_1}|T-\psi(\theta_1)|^2-|\E_{\theta_1}T-\psi(\theta_1)|^2+(\E_{\theta_1}T-c)^2+\E_{\theta_2}|T-\psi(\theta_2)|^2-|\E_{\theta_2}T-\psi(\theta_2)|^2+(\E_{\theta_2}T-c)^2\right\} \\
    &\qquad\qquad\left(4-H^2(P_{\theta_1}, P_{\theta_2})\right)\\
    &\qquad=\left\{R(\theta_1)+R(\theta_2)-\{d^2(\theta_1)+d^2(\theta_2)\}+\frac{1}{2}(\E_{\theta_1}T-\E_{\theta_2}T)^2\right\} \left(4-H^2(P_{\theta_1}, P_{\theta_2})\right)
\end{align*}
where we use $c = \frac{\E_{\theta_1}T+\E_{\theta_2}T}{2}$. This implies 
\begin{align*}
    |\E_{\theta_1}T-\E_{\theta_2}T|^2\frac{\left(1-\frac{4-H^2}{2}\right)}{4-H^2}+\{d^2(\theta_1)+d^2(\theta_2)\} \leq R(\theta_1)+R(\theta_2)
\end{align*}
Unfortunately, $\frac{\left(1-\frac{4-H^2}{2}\right)}{4-H^2} \leq 0$ when $H^2 \leq 2$. 

\kt{
\begin{itemize}
    \item All these attempts had similar challenge to control $\int T(x)\left(p_{\theta_1}p_{\theta_2}\right)^{1/2} \, d\mu(x)$ or $\int T^2(x)\left(p_{\theta_1}p_{\theta_2}\right)^{1/2} \, d\mu(x)$. 
    \item The only bound I could think of was:\begin{align*}
    \int T^2(x)\left(p_{\theta_1}p_{\theta_2}\right)^{1/2} \, d\mu(x) \leq \int_AT^2(x)p_{\theta_1}\, d\mu(x) + \int_{A^c}T^2(x)p_{\theta_2}\, d\mu(x)
\end{align*}
But the issue of this approach is that we don't know how $T$ behaves over the set $A$. 
\item The attempt 4 was promising at first, but I think the trivial lower bound $\int T^2(x)\left(p_{\theta_1}p_{\theta_2}\right)^{1/2} \, d\mu(x) \geq0$ was not good enough.
\end{itemize}
}
\subsection{Lemma 1 of \cite{chen1997general}}
An alternative proof technique directly derives the lower bound for $R(\theta_1)+R(\theta_2)$ using Markov's inequality.
\begin{proof}
Let $\alpha = \frac{1}{2}|\psi(\theta_1)+\psi(\theta_2)|$ and an event $A = \{|T(x)-\psi(\theta_2)| \leq \alpha\}$. By triangle inequality, we have
\begin{align*}
   &|T(x)-\psi(\theta_2)| \leq \alpha\\
    &\qquad \implies |T(x)-\psi(\theta_2)+\psi(\theta_1)-\psi(\theta_1)| \leq \alpha\\
    &\qquad \implies |\psi(\theta_2)+\psi(\theta_1)|-|T(x)-\psi(\theta_1)| \leq \alpha\\
    &\qquad \implies |\psi(\theta_2)+\psi(\theta_1)|-\alpha \leq |T(x)-\psi(\theta_1)|\\
    &\qquad \implies \frac{1}{2}|\psi(\theta_2)+\psi(\theta_1)| \leq |T(x)-\psi(\theta_1)|\\
    &\qquad \implies \alpha \leq |T(x)-\psi(\theta_1)|.
\end{align*}
Naturally, we have 
\[|T(x)-\psi(\theta_2)|^2 \leq \alpha^2 \implies \alpha^2 \leq |T(x)-\psi(\theta_1)|^2.\]
We thus conclude 
\[\mathbb{P}(\{|T(x)-\psi(\theta_2)|^2 \leq \alpha^2\}) \leq \mathbb{P}(\{|T(x)-\psi(\theta_1)|^2 \leq \alpha^2\}).\]
By Markov's inequality 
\begin{align*}
    \E_{\theta_1}|T-\psi(\theta_1)|^2 + \E_{\theta_2}|T-\psi(\theta_1)|^2 &\geq \alpha^2\mathbb{P}_{\theta_1}(|T-\psi(\theta_1)|^2\geq \alpha^2)+\alpha^2\mathbb{P}_{\theta_2}(|T-\psi(\theta_2)|^2\geq \alpha^2)\\
    &\geq \alpha^2\mathbb{P}_{\theta_1}(|T-\psi(\theta_2)|^2\leq \alpha^2)+\alpha^2\mathbb{P}_{\theta_2}(|T-\psi(\theta_2)|^2\geq \alpha^2) \\
    &=\alpha^2 \left\{\mathbb{P}_{\theta_1}(|T-\psi(\theta_2)|^2\leq \alpha^2)+1-\mathbb{P}_{\theta_2}(|T-\psi(\theta_2)|^2\leq \alpha^2)\right\}\\
    &\geq\alpha^2 \left\{1-\int_Ap_{\theta_2}-p_{\theta_1}\, d\mu(x)\right\}\\
    &\geq \alpha^2 \left\{1-\frac{1}{2}TV(P_{\theta_1}, P_{\theta_2})\right\}
    \end{align*}
    
The original proof is credited \cite{donoho1987geometrizing}. There might be useful technical tools in \cite{donoho1987geometrizing,donoho1991geometrizing2,donoho1991geometrizing3}.
\end{proof}

\begin{figure}[h]
     \centering
     \begin{subfigure}{0.9\textwidth}
         \centering
         \includegraphics[width=\textwidth]{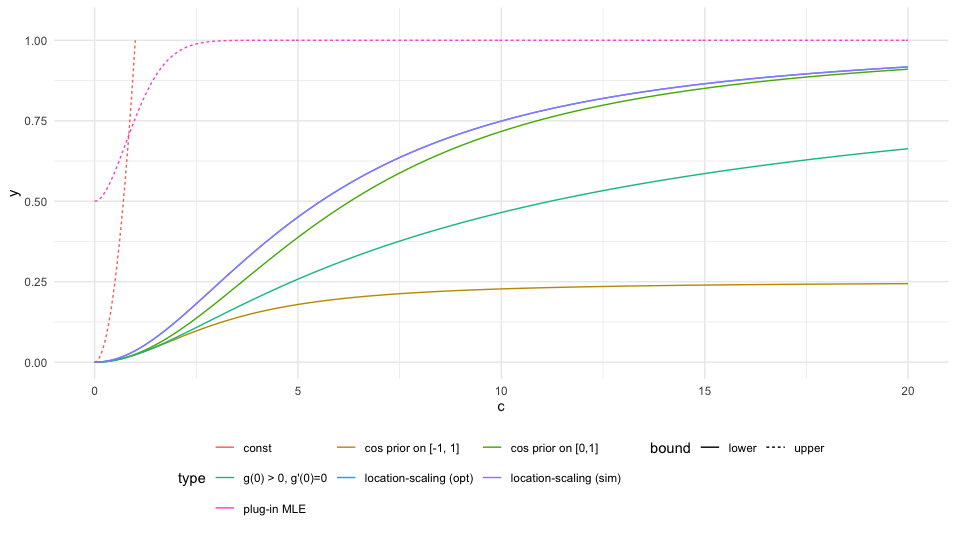}
     \end{subfigure}
\end{figure}
