# Supplementary material for: Generalized van Trees inequality: Local minimax bounds for non-smooth functionals and irregular statistical models
Source: arXiv:2405.06437 source file (2024-10-19)
Supplement: Supplementary file 5 [file lam.tex]

\clearpage
\section{Asymptotic Properties}

Or nonparametric version:
\begin{align}
    \sup_{g \in \mathcal{G}} \liminf_{n\to \infty} \E_{P_{n^{-1/2}, g}}\left[n^{1/2}\big\{T - \psi(P_{n^{-1/2}, g})\big\}\right]^2 \ge P_0\dot{\psi}_{\theta_0}\dot{\psi}_{\theta_0}^T
\end{align}
\kt{Myabe check the treatment of constant $cn^{-1/2}$ so it's consistent with parametric version}
\subsection{van Trees inequality}
\begin{definition}[Absolute continuity on $\mathbb{R}^d$]
A function $q := \mathbb{R}^d \mapsto \mathbb{R}$ is absolutely continuous on $B([\theta], \delta)$ for $\delta > 0$ if there exits an integrable function $\nabla q := \mathbb{R}^d \mapsto \mathbb{R}$ such that 
\begin{align*}
    q(\theta+\delta u) - q(\theta) = \int_{\theta}^{\theta+\delta u} \nabla q(t)\, dt
\end{align*}
for all unit vector $u \in \mathbb{R}^d$. Similarly for a density function defined on $\mathcal{X}$ with respect to $\sigma$-finite measure $\mu$, $p_\theta$ is absolutely continuous on $B([\theta], \delta)$ for $\delta > 0$ if there exists a $\mu$-almost everywhere integrable function $\nabla p_\theta$ such that 
\begin{align*}
    p_{\theta+\delta u}(x) - p_\theta(x) = \int_{\theta}^{\theta+\delta u} \nabla p_t(x)\, dt
\end{align*}
$\mu$-almost everywhere for all unit vector $u \in \mathbb{R}^d$.
\end{definition}
\begin{definition}[Regularity condition for a statistical model]
Consider a family of distributions $\{P_t : t \in \Theta \subseteq \mathbb{R}^d\}$ on X. We call $\{P_t : t \in \Theta\}$ satisfies the regularity conditions if it satisfies all of the following:
\begin{enumerate}[label=\textbf{(A\arabic*)},leftmargin=2cm]
\setcounter{enumi}{1}
\item There exists $\delta > 0$ such that 
\begin{enumerate}
    \item The function $\theta \in \Theta \mapsto p_\theta(x)$ is absolutely continuous on $B(\theta_0, \delta)$ with gradients at $t \in B(\theta_0, \delta)$ denoted by $\nabla p_t(x)$, which is continuous at $\theta_0$.
        \item The following mapping
        \begin{align}
         x \in \mathcal{X} \mapsto \sup_{t \in B(\theta_0, \delta)}\frac{\nabla p_{\theta_0+t}(x)}{\sqrt{p_{\theta_0}(x)}}I\{p_{\theta_0} > 0\}
    \end{align}
    is square-integrable with respect to $\mu$.
    \end{enumerate}

    \end{enumerate}
\end{definition}

\begin{definition}[Regularity condition for a location model]
Consider a location family $\{Q_h : 0 < \|h\| \le \delta\}$, which is given by $q_h(t) = q(t-h)$. We call $Q_h$ satisfies the regularity conditions if all of the following conditions hold:
\begin{enumerate}[label=\textbf{(A\arabic*)},leftmargin=2cm]
\setcounter{enumi}{2}
\item There exists $\delta > 0$ such that 
\begin{enumerate}
    \item The density $q$ is bounded and absolute continuous function on $B([\theta_0], \delta)$ whose gradient $\nabla q$ is continuous at $\theta_0$. 
        \item The following mapping
        \begin{align}
         t \in \mathbb{R}^d \mapsto \sup_{t \in B(\theta, \delta)}\frac{\nabla q(\theta+t)}{\sqrt{q(\theta)}}I\{q(\theta) > 0\}\label{eq:reg_int_q}
        \end{align}
    is square-integrable with respect to Lebesgue measure.
    \end{enumerate}
    \end{enumerate}
\end{definition}
\begin{proposition}\label{prop:lam_vt_chisq}
Theorem~\ref{thm:crvtBound} implies 
\begin{align}
    \liminf_{c\to \infty} \liminf_{n\to \infty}\sup_{\|h\| \le c} \E_{\theta_0 + hn^{-1/2}}\left[n^{1/2}\big\{T - \psi(\theta_0 + hn^{-1/2})\big\}\right]^2 \ge \nabla\psi_{\theta_0}\mathcal{I}(\theta_0)^{-1}\nabla\psi_{\theta_0}^T
\end{align}
\end{proposition}
\begin{proof}[\bfseries{Proof of Proposition~\ref{prop:lam_vt_chisq}}]
\kt{We need to rewrite the assumption to allow something like a Gaussian prior}
For this proof, we assume that $\Theta \subseteq \mathbb{R}^d$ and the real-valued function $\psi : \Theta \mapsto \mathbb{R}$. We consider the density function $q$ whose support is given by an open unit ball in $\mathbb{R}^d$. We introduce the location-scaling family of this density function such that
\begin{align}
    q_{n, c, \delta}(t) := \begin{cases}
    \frac{1}{\gamma^d_{n,c,\delta}}q\left(\frac{t-\theta_0}{\gamma_{n,c,\delta}}\right) & \text{ when } t \in B(\theta_0, \gamma_{n,c,\delta})\\
    0  & \text{ when } t \in B(\theta_0, cn^{-1/2}) \setminus B(\theta_0, \gamma_{n,c,\delta})\\
    \end{cases}\nonumber
\end{align}
where $\gamma_{n,c,\delta} := cn^{-1/2}-2\delta $ for $0 < \delta < \frac{cn^{-1/2}}{2}$. By construction, we have 
\[\supp(q_{n, c, \delta}) = B(\theta_0,\gamma_{n,c,\delta}) = B^{(-2\delta)}(\theta_0, cn^{-1/2})\]
and thus the density function $q_{n, c, \delta}$ satisfies the assumption \ref{as:IPBorder} for any fixed $0 < \delta < \frac{cn^{-1/2}}{2}$. Throughout the proof, we assume $c$ and $\delta$ are fixed constants. 
\kt{Condition of $n$ large enough}
\begin{align*}
    |\psi(\theta_0) - \psi(\theta_0 - u\gamma)|\,  \vee 
\end{align*}
When $c, \delta$ and $n$ are fixed, $\gamma_{n,c,\delta}$ is also fixed. We thus drop the subscript from $\gamma_{n,c,\delta}$ and also adapt the notation $q_{n, c, \delta} = q_{\gamma}$ for simpler exposition. For any $h \in \mathbb{R}^d$ such that $\|h\| \le c$, we have

\begin{align*}
   \sup_{\|h\| \le c} \E_{\theta_0 + hn^{-1/2}}\big|T(X) - \psi(\theta_0 + hn^{-1/2})\big|^2 &= \sup_{t \in B(\theta_0, cn^{-1/2})}\E_{t}\left|T(X)-\psi(t)\right|^2.
\end{align*}
We now apply Theorem~\ref{thm:crvtBound} to the last display, which gives the following lower bound:
\begin{align}
    &\sup_{t \in B(\theta_0, cn^{-1/2})}\E_{t}\left|T(X)-\psi(t)\right|^2 \ge \sup_{0 < \delta < \frac{cn^{-1/2}}{2}}\sup_{ \|h\|<\delta}\frac{\left|\int_{B(\theta_0, cn^{-1/2})} \left\{\psi(t)-\psi(t-h)\right\} q_{\gamma}(t)\,dt\right|^2}{\overline{\chi}^2(Q_{h,\gamma}\|Q_{\gamma})+\int_{B(\theta_0, cn^{-1/2})} \frac{ q_{\gamma}(t+h)^2}{ q_{\gamma}(t)}\chi^2(P^n_{t+h}\|P^n_t)I( q_{\gamma}(t)>0)\,dt}\nonumber.
\end{align}
For any $u \in \mathbb{R}^d$ such that $\|u\|=1$, consider an arbitrary sequence $h = u\varepsilon_i$ such that $\varepsilon_i \in (-\delta, \delta)$ and $\varepsilon_i \to 0$ as $i \to \infty$. We then have
\begin{align}
    &\sup_{ \|h\|<\delta}\frac{\left|\int_{B(\theta_0, \gamma)} \left\{\psi(t)-\psi(t-h)\right\}q_{\gamma}(t)\,dt\right|^2}{\overline{\chi}^2(Q_{h,\gamma}\|Q_{\gamma})+\int_{B(\theta_0, \gamma)} \frac{q_\gamma(t+h)^2}{q_\gamma(t)}\chi^2(P_{t+h}\|P_t)\,dt} \nonumber \\
    &\qquad\ge \sup_{\|u\|=1} \liminf_{i \to \infty}\frac{\varepsilon_i^{-2}\left|\int_{B(\theta_0, \gamma)} \left\{\psi(t)-\psi(t-u\varepsilon_i)\right\}q_\gamma(t)\,dt\right|^2}{\varepsilon_i^{-2}\overline{\chi}^2(Q_{u\varepsilon_i,\gamma}\|Q_{\gamma})+\varepsilon_i^{-2}\int_{B(\theta_0, \gamma)} \frac{q_\gamma(t+u\varepsilon_i)^2}{q_\gamma(t)}\chi^2(P^n_{t+u\varepsilon_i}\|P^n_t)\,dt}.\nonumber
\end{align}
We now analyze the limiting behaviors of all terms at hand. 
For the numerator, we have
\begin{align}
    \liminf_{i \to \infty}\varepsilon_i^{-2}\left|\int_{B(\theta_0, \gamma)} \left\{\psi(t)-\psi(t-h)\right\} q_{\gamma}(t)\,dt\right|^2
    &=\liminf_{i \to \infty}\left|\int_{B(\theta_0, \gamma)} \left\{\frac{\psi(t)-\psi(t-u\varepsilon_i)}{\varepsilon_i}\right\}\frac{1}{\gamma^d}q\left(\frac{t-\theta_0}{\gamma}\right)
\,dt\right|^2\nonumber\\
    &=\liminf_{i \to \infty}\left|\int_{B([0], 1)} \left\{\frac{\psi(\theta_0 +\gamma s)-\psi(\theta_0 +\gamma s-u\varepsilon_i)}{\varepsilon_i}\right\}q(s)\,ds\right|^2\nonumber\\
    &\ge\left|\int_{B([0], 1)} \liminf_{i \to \infty}\left\{\frac{\psi(\theta_0 +\gamma s)-\psi(\theta_0 +\gamma s-u\varepsilon_i)}{\varepsilon_i}\right\}q(s)\,ds\right|^2\nonumber\\
&=\left|\int_{B([0], 1)} \nabla \psi_{\theta_0 +\gamma s}\, u q(s)\,ds\right|^2\nonumber
\end{align}
where we used change of variables with $s = \frac{t-\theta_0}{\gamma}$, Fatou's lemma and the continuity of $\nabla \psi$ at $\theta_0$. By Lemma~\ref{lm:chisq_Q} and Lemma~\ref{lm:chisq_P}, we have
\begin{align}
    \liminf_{i\to\infty}\varepsilon_i^{-2}\overline{\chi}^2(Q_{u\varepsilon_i,\gamma}\|Q_{\gamma}) = u^T\frac{\mathcal{J}(Q)}{\gamma^2} u\nonumber
\end{align}
and 
\begin{align}
    \liminf_{i\to\infty}\varepsilon_i^{-2}\int_{B(\theta_0, \gamma)} \frac{q_\gamma(t+u\varepsilon_i)^2}{q_\gamma(t)}\chi^2(P^n_{t+u\varepsilon_i}\|P^n_t)\,dt = u^T\left(n\int_{B([0], 1)} \mathcal{I}(\theta_0+\gamma s) q(s)\, ds\right)  u.\nonumber
\end{align}
Putting together the results up to this point, we have
\begin{align*}
    &\sup_{\|h\| \le c} \E_{\theta_0 + hn^{-1/2}}\big|T(X) - \psi(\theta_0 + hn^{-1/2})\big|^2\ge \sup_{0 < \delta < \frac{cn^{-1/2}}{2}}\sup_{\|u\|=1}\frac{\left|\int_{B([0], 1)} \nabla \psi_{\theta_0 +\gamma s}\, u q(s)\,ds\right|^2}{u^T\left(\gamma^{-2} \mathcal{J}(Q) + \int_{B([0], 1)}\mathcal{I}(\theta_0 + \gamma s)q(s)\, ds\right)\, u}.
\end{align*}
Finally, we set $u := \|M^{-1/2}\|^{-1}M^{-1/2}$ where 
\[M := \left(\gamma^{-2} \mathcal{J}(Q) + \int_{B([0], 1)}\mathcal{I}(\theta_0 + \gamma s)q(s)\, ds\right).\]
For this choice of $u$, we obtain 
\begin{align*}
    & \sup_{0 < \delta < \frac{cn^{-1/2}}{2}}\sup_{\|u\|=1}\frac{\left|\int_{B([0], 1)} \nabla \psi_{\theta_0 +\gamma s}\, uq(s)\,ds\right|^2}{u^T\left(\gamma^{-2} \mathcal{J}(Q) + \int_{B([0], 1)}\mathcal{I}(\theta_0 + \gamma s)q(s)\, ds\right)\, u}\\
    &\qquad \ge  \sup_{0 < \delta < \frac{cn^{-1/2}}{2}}\int_{B([0], 1)}\nabla \psi_{\theta_0 +\gamma s}\left(\gamma^{-2} \mathcal{J}(Q) + \int_{B([0], 1)}\mathcal{I}(\theta_0 + \gamma s)q(s)\, ds\right)^{-1}\nabla \psi_{\theta_0 +\gamma s}^Tq(s)\,ds.
\end{align*}
The lower bound depends on $\delta$ only through $\gamma$ as by definition $\gamma := cn^{-1/2}-2\delta$. We can thus further give the lower bound with respect to $\delta$ by taking $\delta \to 0$, which implies $\gamma \to cn^{-1/2}$. We thus have 
\begin{align*}
    &\sup_{\|h\| \le c} \E_{\theta_0 + hn^{-1/2}}\left[n^{1/2}\big\{T - \psi(\theta_0 + hn^{-1/2})\big\}\right]^2 \\
    &\qquad \ge \sup_{0 < \delta < \frac{cn^{-1/2}}{2}}\int_{B([0], 1)}\nabla \psi_{\theta_0 +\gamma s}\left(\frac{1}{n\gamma^2}\mathcal{J}(Q) + \int_{B([0], 1)}\mathcal{I}(\theta_0 + \gamma s)q(s)\, ds\right)^{-1}\nabla \psi_{\theta_0 +\gamma s}^T\,q(s)\,ds\\
    &\qquad \ge \int_{B([0], 1)}\nabla \psi_{\theta_0 +cn^{-1/2} s}\left(c^{-2} \mathcal{J}(Q) + \int_{B([0], 1)}\mathcal{I}(\theta_0 + cn^{-1/2} s)q(s)\, ds\right)^{-1}\nabla \psi_{\theta_0 +cn^{-1/2} s}^T\,q(s)\,ds \\
    & \implies \liminf_{n\to \infty}\sup_{\|h\| \le c} \E_{\theta_0 + hn^{-1/2}}\left[n^{1/2}\big\{T - \psi(\theta_0 + hn^{-1/2})\big\}\right]^2 \ge \nabla \psi_{\theta_0}\left(c^{-2} \mathcal{J}(Q) + \mathcal{I}(\theta_0)\right)^{-1}\nabla \psi_{\theta_0}^T \\
    & \implies\liminf_{c\to \infty} \liminf_{n\to \infty}\sup_{\|h\| \le c} \E_{\theta_0 + hn^{-1/2}}\left[n^{1/2}\big\{T - \psi(\theta_0 + hn^{-1/2})\big\}\right]^2 \ge \nabla\psi_{\theta_0}\mathcal{I}(\theta_0)^{-1}\nabla \psi_{\theta_0}^T
\end{align*}
This concludes the claim. 
\end{proof}

\begin{lemma}\label{lm:chisq_Q}
Assuming $q$ is a bounded and absolutely continuous density function with finite Fisher information, we have
\begin{align}
   \liminf_{i\to\infty}\varepsilon_i^{-2}\overline{\chi}^2(Q_{u\varepsilon_i,\gamma}\|Q_{\gamma}) = \frac{u^T\, \mathcal{J}(Q)\, u}{\gamma^2}
\end{align}
\end{lemma}
\begin{proof}[\bfseries{Proof of Lemma~\ref{lm:chisq_Q}}]
We assume that $\varepsilon_i$ is small enough such that $\varepsilon_i < \gamma\delta$. By the absolute continuity of $q$ on $B(\theta_0, \delta)$, we have
\begin{align*}
    \liminf_{i\to\infty}\varepsilon_i^{-2}\overline{\chi}^2(Q_{u\varepsilon_i,\gamma}\|Q_{\gamma}) &=  \liminf_{i\to\infty}\int_{B(\theta_0, \gamma)} \left(\frac{q_{\gamma}(t+u\varepsilon_i)-q_{\gamma}(t)}{\varepsilon_i q_{\gamma}(t)}\right)^2 q_{\gamma}(t)\, dt \\
     &=  \liminf_{i\to\infty}\int_{B(\theta_0, \gamma)} \left(\frac{q\left(\frac{t-\theta_0+u\varepsilon_i}{\gamma}\right)-q\left(\frac{t-\theta_0}{\gamma}\right)}{\varepsilon_i q\left(\frac{t-\theta_0}{\gamma}\right)}\right)^2 \frac{1}{\gamma^d}q\left(\frac{t-\theta_0}{\gamma}\right)\, dt\\
     &= \liminf_{i\to\infty}\int_{B([0], 1)} \left(\frac{q\left(s+\frac{u\varepsilon_i}{\gamma}\right)-q(s)}{\varepsilon_i q(s)}\right)^2 q(s)\, ds \\
    &= \liminf_{i\to\infty}\int_{B([0], 1)} \left(\frac{\int_{s}^{s+u\varepsilon_i/\gamma}\nabla q(\tilde{s})\,d\tilde{s}}{\varepsilon_i q(s)}\right)^2 q(s)\, ds.
\end{align*}

The integral in the above display can be written out as follows:
\begin{align*}
    \int_{B([0], 1)} \left(\frac{\int_{s}^{s+u\varepsilon_i/\gamma}\nabla q(\tilde{s})\,d\tilde{s}}{\varepsilon_i q(s)}\right)^2 q(s)\, ds
    &= \gamma^{-2}\int_{B([0], 1)}\frac{1}{q(s)} \left(\int_{B([0], 1)}\nabla q(s+t\varepsilon_i /\gamma)\,dt\right)^2 \, ds \\
    &= \gamma^{-2}\iiint_{B([0], 1)\times B([0], 1)\times B([0], 1)}\frac{\nabla q(s+t_1\varepsilon_i /\gamma)\nabla q(s+t_2\varepsilon_i /\gamma)}{q(s)}\,dt_1\, dt_2\, ds 
\end{align*}
The last integral is bounded as $\varepsilon_i \to 0$ by the regularity condition \eqref{eq:reg_int_q}. Furthermore, the continuity of the gradient at $s$ implies that $\nabla q(s+t_1\varepsilon_i /\gamma)\nabla q(s+t_2\varepsilon_i /\gamma) \to \nabla q(s)^2$ as $\varepsilon_i \to 0$. By the application of dominate convergence theorem, we obtain that  
\begin{align*}
\liminf_{i\to\infty}\int_{B([0], 1)} \left(\frac{\int_{s}^{s+u\varepsilon_i/\gamma}\nabla q(\tilde{s})\,d\tilde{s}}{\varepsilon_i q(s)}\right)^2 q(s)\, ds &=
\int_{B([0], 1)}\liminf_{i\to\infty} \left(\frac{\int_{s}^{s+u\varepsilon_i/\gamma}\nabla q(\tilde{s})\,d\tilde{s}}{\varepsilon_i q(s)}\right)^2 q(s)\, ds\\
&= \,\frac{1}{\gamma^2}\int_{B([0], 1)} \frac{\{\nabla q(s) u\}^2}{q(s)}\, ds  \\
&= \frac{u^T\, \mathcal{J}(Q)\, u}{\gamma^2}
\end{align*}
This concludes the claim.

\end{proof}

\begin{lemma}\label{lm:chisq_P}
Assuming that the prior $q : \mathbb{R}^d \mapsto \mathbb{R}$ is absolutely continuous and $\nabla q$ is continuous. Additionally, $P_t$ is regular on $B(\theta_0, \delta)$ for some $\delta \ge \gamma > 0$, we have
\begin{align*}
    \liminf_{i\to\infty}\int_{B(\theta_0, \gamma)} \frac{q_{\gamma}(t+u\varepsilon_i)^2}{q_{\gamma}(t)}\varepsilon_i^{-2} \chi^2(P^n_{t+u\varepsilon_i}\|P^n_t)I(q_{\gamma}(t)>0)\,dt = u^T\left(n\int_{B([0], 1)} \mathcal{I}(\theta_0+scn^{-1/2})\, q(s)\, ds \right)\, u.
\end{align*}
\end{lemma}
\begin{proof}
First, by the change of variables, we have
\begin{align*}
    &\liminf_{i\to\infty}\int_{B(\theta_0, \gamma)} \frac{q_{\gamma}(t+u\varepsilon_i)^2}{q_{\gamma}(t)}\varepsilon_i^{-2}\chi^2(P^n_{t+u\varepsilon_i}\|P^n_t)I(q_{\gamma}(t)>0)\,dt \\
    &\qquad= \liminf_{i\to\infty}\int_{B(\theta_0, \gamma)}\left(\frac{1}{\gamma^d}\right) \frac{q\left(\frac{t+u\varepsilon_i-\theta_0}{\gamma}\right)^2}{q\left(\frac{t-\theta_0}{\gamma}\right)}\varepsilon_i^{-2}\chi^2(P^n_{t+u\varepsilon_i}\|P^n_t)\,dt\\
    &\qquad= \liminf_{i\to\infty}\int_{B([0], 1)} \frac{q\left(s+\frac{u\varepsilon_i}{\gamma}  \right)^2}{q(s)}\varepsilon_i^{-2}\chi^2(P^n_{\theta_0 + \gamma s + u\varepsilon_i}\|P^n_{\theta_0 + \gamma s})\,ds.
\end{align*}
In order to apply the dominated convergence theorem, we study the terms inside of the integral.
By the absolute continuity of $q$, we have
\begin{align*}
     \frac{q\left(s+\frac{u\varepsilon_i}{\gamma}  \right)^2}{q(s)} &=  \frac{\left(q(s) + \int_{s}^{s+u \varepsilon_i/\gamma} \nabla q(t)\, dt \right)^2}{q(s)}= q(s) + 2 \int_{s}^{s+u \varepsilon_i/\gamma} \nabla q(t)\, dt + \left(\int_{s}^{s+u \varepsilon_i/\gamma} \nabla q(t)\, dt\right)^2.
\end{align*}
Furthermore, we assume that the gradient $\nabla q$ to be continuous so it is locally bounded such that $|\nabla q| \le M < \infty$. This implies that
\begin{align*}
     \frac{q\left(s+\frac{u\varepsilon_i}{\gamma}  \right)^2}{q(s)} &\le  q(s) + 2 \int_{s}^{s+u \varepsilon_i/\gamma} \nabla q(t)u\, dt + \left(\int_{s}^{s+u \varepsilon_i/\gamma} \nabla q(t)u\, dt\right)^2\\
    &\le  q(s) + 2 M \varepsilon_i/\gamma + \left(2 M \varepsilon_i/\gamma \right)^2\\
    & = q(s) + O(\varepsilon_i).
\end{align*}
For the chi-square divergence between $P^n_{\theta_0 + \gamma s + u\varepsilon_i}$ and $P^n_{\theta_0 + \gamma s}$, Lemma~\ref{lm:chisq_local_behavior} states that 
\begin{align}
    \varepsilon_i^{-2}\chi^2(P^n_{\theta_0 + \gamma s + u\varepsilon_i}\|P^n_{\theta_0 + \gamma s}) = u^T\, \mathcal{I}^n(\theta_0 + \gamma s) \,u + o(1)\nonumber.
\end{align}
Therefore, assuming $\mathcal{I}(\theta)$ is continuous at $\theta_0$, it is locally bounded as for $n$ large enough, which in turn implies $\gamma \to 0$. 
\begin{align*}
    &\liminf_{i\to\infty}\int_{B([0], 1)} \frac{q\left(s+\frac{u\varepsilon_i}{\gamma}  \right)^2}{q(s)}\varepsilon_i^{-2}\chi^2(P^n_{\theta_0 + \gamma s + u\varepsilon_i}\|P^n_{\theta_0 + \gamma s})\,ds \\
    &\qquad = \liminf_{i\to\infty}\int_{B([0], 1)} (q(s) + O(\varepsilon_i))(u^T\, \mathcal{I}^n(\theta_0 + \gamma s) \,u + o(1))\,ds.
\end{align*}
\end{proof}

Here I state two technical lemmas I borrow from the existing results.

\begin{lemma}\label{lm:chisq_local_behavior}
When $P_t$ is regular on $B(\theta, \delta)$, we then have 
\begin{align}
    \chi^2(P_\theta, P_{\theta + u\varepsilon}) = \varepsilon^2 u^T \mathcal{I}(\theta) u + o(| \varepsilon|^2)
\end{align}
as $\varepsilon \to 0$.

\end{lemma}
\begin{proof}
The local behavior of $\chi^2$-divergence requires regularity conditions. We need to extend Theorem 7.12 of
\url{https://people.lids.mit.edu/yp/homepage/data/LN_fdiv.pdf} to a multivariate version. \kt{Looking for an earlier citation}.
\kt{What kind of distributions satisfy this condition?}

\begin{align*}
    \chi^2(P_{t+u\varepsilon_i}\|P_t) &= \int_{\mathcal{X}} \frac{\{p_{t+u\varepsilon_i}(x)-p_t(x)\}^2}{p_t(x)}I\{p_t(x)>0\}\, \mu(dx)\\
    &= \int_{\mathcal{X}} \frac{\{\int_t^{t+u\varepsilon_i}\nabla p_s(x)\, ds\}^2}{p_t(x)}I\{p_t(x)>0\}\, \mu(dx)
\end{align*}
\end{proof}

\begin{proposition}
Assuming the location family $Q_h$ is differentiable in quadratic mean, $q$ is continuous and bounded 
and $\{P_\theta: \theta \in \Theta\}$ is differentiable in quadratic mean at $\theta = \theta_0$, then  Theorem~\ref{thm:crvtBound_hellinger} implies 
\end{proposition}
\begin{proof}
For any $h \in \mathbb{R}^d$ such that $\|h\| \le c$, we have

\begin{align*}
   \sup_{\|h\| \le c} \E_{\theta_0 + hn^{-1/2}}\big|T(X) - \psi(\theta_0 + hn^{-1/2})\big|^2 &\ge \sup_{t \in B(\theta_0, \gamma)}\E_{t}\left|T(X)-\psi(t)\right|^2 \\
   &\ge \int_{B(\theta_0, \gamma)} \E_{t}\left|T(X)-\psi(t)\right|^2 q_{\gamma}(t)\, dt
\end{align*}
We now apply Theorem~\ref{thm:crvtBound_hellinger} to the last display, which gives the lower bound:
\begin{align}
    &\int_{B(\theta_0, cn^{-1/2})} \E_{t}\left|T(X)-\psi(t)\right|^2 q_{\gamma}(t)\, dt \nonumber\\
    &\qquad\ge \sup_{0 < \delta < \frac{cn^{-1/2}}{2}}\sup_{ \|h\|<\delta}   \left[\left\{\frac{\left|\int_{B(\theta_0, cn^{-1/2})} \left(\psi(u)-\psi(u-h)\right)q_\gamma(u)\,du\right|^2}{4\E_{X, \theta} \left(\sqrt{\frac{\gamma_h(X,\theta)}{\gamma_0(X,\theta)}}-1\right)^2} \right\}^{1/2}\right.\nonumber\\
    &\qquad\qquad\left.-\left\{\int_{B(\theta_0, cn^{-1/2})} \left(\psi(t+h)-\psi(t)\right)^2q_\gamma(t+h) \, dt\right\}^{1/2}\right]^2_+\nonumber
\end{align}
For any $u \in \mathbb{R}^d$ such that $\|u\|=1$, consider an arbitrary sequence $h = u\varepsilon_i$ such that $\varepsilon_i \in (-\delta, \delta)$ and $\varepsilon_i \to 0$ as $i \to \infty$. We then have
\begin{align}
    &\sup_{ \|h\|<\delta}\left[\left\{\frac{\left|\int_{B(\theta_0, \gamma)} \left(\psi(t)-\psi(t-h)\right)q_\gamma(t)\,dt\right|^2}{4\E_{X, \theta} \left(\sqrt{\frac{\gamma_h(X,\theta)}{\gamma_0(X,\theta)}}-1\right)^2} \right\}^{1/2}-\left\{\int_{B(\theta_0, \gamma)} \left(\psi(t)-\psi(t-h)\right)^2q_\gamma(t) \, dt\right\}^{1/2}\right]^2_+ \nonumber \\
    &\qquad\ge \sup_{\|u\|=1} \liminf_{i \to \infty}\left[\left\{\frac{\left|\int_{B(\theta_0, \gamma)} \left(\psi(t)-\psi(t-u\varepsilon_i)\right)q_\gamma(t)\,dt\right|^2}{4\E_{X, \theta} \left(\sqrt{\frac{\gamma_{u\varepsilon_i}(X,\theta)}{\gamma_0(X,\theta)}}-1\right)^2} \right\}^{1/2}-\left\{\int_{B(\theta_0, \gamma)} \left(\psi(t)-\psi(t-u\varepsilon_i)\right)^2q_\gamma(t) \, dt\right\}^{1/2}\right]^2_+\nonumber.
\end{align}

We evaluate all terms at hand. 
\begin{align}
    \liminf_{i \to \infty}\varepsilon_i^{-2}\left|\int_{B(\theta_0, \gamma)} \left\{\psi(t)-\psi(t-h)\right\} q_{\gamma}(t)\,dt\right|^2
    &\ge\left|\int_{B([0], 1)} \nabla \psi_{\theta_0 +\gamma s}\, u q(s)\,ds\right|^2\nonumber
\end{align}

\begin{align*}
    \int_{B(\theta_0, \gamma)} \left(\psi(t)-\psi(t-u\varepsilon_i)\right)^2q_\gamma(t)\, dt &= \int_{B(\theta_0, \gamma)} \left(\frac{\psi(t)-\psi(t-u\varepsilon_i)}{\varepsilon_i}\right)^2\frac{1}{\gamma^d}q\left(\frac{t-\theta_0}{\gamma}\right)\, dt\\
    &= \int_{B([0], 1)} \left(\frac{\psi(\theta_0+\gamma s)-\psi(\theta_0+\gamma s-u\varepsilon_i)}{\varepsilon_i}\right)^2q\left(s\right)\, ds
\end{align*}

\begin{align*}
    \E_{X, \theta} \left(\sqrt{\frac{\gamma_{u\varepsilon_i}(x,\theta)}{\gamma_0(x,\theta)}}-1\right)^2 &=\E_{X, \theta} \left(\frac{\gamma_{u\varepsilon_i}(x,\theta)}{\gamma_0(x,\theta)}+1 - 2\sqrt{\frac{\gamma_{u\varepsilon_i}(x,\theta)}{\gamma_0(x,\theta)}}\right)\\
    &=2-2\iint_{\mathcal{X}\times B(\theta_0, \gamma)}  p^{1/2}_{t+u\varepsilon_i}(x)q^{1/2}(t+u\varepsilon_i)p^{1/2}_{t}(x)q^{1/2}(t)\, \mu(dx)\,dt \\
    &=2-2\int_{B(\theta_0, \gamma)} q^{1/2}(t+u\varepsilon_i)q^{1/2}(t)\int_{\mathcal{X}}  p^{1/2}_{t+u\varepsilon_i}(x)p^{1/2}_{t}(x)\, \mu(dx)\,dt\\
    &=2-2\int_{B(\theta_0, \gamma)} q^{1/2}(t+u\varepsilon_i)q^{1/2}(t)\left(1-\frac{1}{2}H^2(P_{t+u\varepsilon_i}, P_{t})\right)\,dt\\
    &=H^2(Q_h, Q) +\int_{B(\theta_0, \gamma)} q^{1/2}(t+u\varepsilon_i)q^{1/2}(t)H^2(P_{t+u\varepsilon_i}, P_{t})\,dt 
\end{align*}
Location family $Q_h$ is DQM if $q$ is continuously differentiable. 
\end{proof}
