# Supplementary material for: Generalized van Trees inequality: Local minimax bounds for non-smooth functionals and irregular statistical models
Source: arXiv:2405.06437 source file (2024-10-19)
Supplement: Supplementary file 6 [file mix_ibragimov.tex]

\clearpage
\section{The extension of \cite{ibragimov1981statistical} to mixture models}
Let $\mu_1$ and $\mu_2$ be probability measures over a parameter space $\Theta$, which index a statistical model $P_\theta$. 
\begin{itemize}
    \item $p_i := \int_{\Theta}p_\theta \,\mu_i(d\theta)$
    \item $m_i := \int \psi(\theta)\, \mu_i(d\theta)$
    \item $V_i^2 := \int [\psi(\theta)-m_i]^2\, \mu_i(d\theta)$
    \item $B(\theta) := E_\theta T- \psi(\theta)$
\end{itemize}

\begin{align*}
    \left|\E_{P_1}T(X)- \E_{P_2}T(X)\right|^2 &= \left|\int_{\mathcal{X}} (T(x)-c)\{p_1(x)-p_2(x)\}\, dx\right|^2 \\
    &= \left|\int_{\mathcal{X}} (T(x)-c)\{p^{1/2}_1(x)-p^{1/2}_2(x)\}\{p^{1/2}_1(x)+p^{1/2}_2(x)\}\, dx\right|^2 \\
    &\le \left|\int_{\mathcal{X}} (T(x)-c)^2\{p^{1/2}_1(x)+p^{1/2}_2(x)\}^2\, dx\right|H^2(P_1, P_2)
    \\
    &\le 2\left\{\E_{P_1}(T(X)-c)^2+\E_{P_2}(T(X)-c)^2\right\} H^2(P_1, P_2)
\end{align*}
where we use Cauchy Schwarz inequality and the fact that $(a+b)^2 \le 2a^2 + 2b^2$.

We may consider alternative upper bound as follows:
\begin{align*}
    &\left|\E_{P_1}T(X)- \E_{P_2}T(X)\right|^2 \\
    &\qquad= \left|\iint_{\Theta \times \mathcal{X}} (T(x)-c)p_t(x)\{\mu_1(t)-\mu_2(t)\}\, dt\,dx\right|^2 \\
    &\qquad= \left|\iint_{\Theta \times \mathcal{X}} (T(x)-c)p_t(x)\{\mu_1^{1/2}(t)-\mu^{1/2}_2(t)\}\{\mu^{1/2}_1(t)+\mu^{1/2}_2(t)\}\, dt\, dx\right|^2 \\
    &\qquad\le \left\{\iint_{\Theta \times \mathcal{X}} (T(x)-c)^2p_t(x)\{\mu^{1/2}_1(t)+\mu^{1/2}_2(t)\}^2\, dt\, dx\right\}\left\{\iint_{\Theta \times \mathcal{X}} \, p_t(x)\{\mu_1^{1/2}(t)-\mu^{1/2}_2(t)\}^2\,dt\,dx\right\} \\
    &\qquad= \left\{\iint_{\Theta \times \mathcal{X}} (T(x)-c)^2p_t(x)\{\mu^{1/2}_1(t)+\mu^{1/2}_2(t)\}^2\, dt\, dx\right\}\left\{\int_\Theta\{\mu_1^{1/2}(t)-\mu^{1/2}_2(t)\}^2\int_\mathcal{X} \, p_t(x)\,dx\,dt\right\} \\
    &\qquad\le 2\left\{\E_{P_1}(T(X)-c)^2+\E_{P_2}(T(X)-c)^2\right\} H^2(\mu_1, \mu_2)
\end{align*}
where the last three steps follow from Cauchy Schwarz inequality,  Tonelli's theorem, and $(a+b)^2 \le 2a^2 + 2b^2$. Two upper bounds only differ by the Hellinger distance. We check which bound is tighter. 
\kt{The looseness of $(a+b)^2 \le 2a^2 + 2b^2$ is different between two examples.}
\begin{align*}
    H^2(P_1, P_2) &= 2 - 2\int_{\mathcal{X}} \sqrt{p_1(x) p_2(x)} \, dx \\
    &= 2-2\int_{\mathcal{X}} \sqrt{\int_{\Theta} p_t(x) \mu_1(t) \, dt \, \int_{\Theta} p_t(x) \mu_2(t)\, dt}\, dx\\
    & \le 2-2\int_{\mathcal{X} }\left(\int_{\Theta} \sqrt{p_t(x) \mu_1(t)} \, dt \,\int_{\Theta}\sqrt{p_t(x) \mu_2(t)}\, dt\right)\, dx
    % &\le 2-2\iint \sqrt{p_t \mu_1 p_t \mu_2}\, d\theta\, dx \\
    % & = H^2(\mu_1, \mu_2)
\end{align*}
{\color{red}Arun: I am not clear on all details of above display. Can you write out all the steps?}\kt{I think you are right. I made a mistake by not writing out formally.
\begin{align*}
\int_{\Theta} \mu_1^{1/2}(t)\mu_2^{1/2}(t)dt \le \int_{\mathcal{X}}\int_{\Theta} p_t(x)\mu_1^{1/2}(t)\mu_2^{1/2}(t)dtdx &\le \int_{\mathcal{X}} \left(\int_{\Theta} p_t(x)\mu_1(t)dt\right)^{1/2}\left(\int_{\Theta} p_t(x)\mu_2(t)dt\right)^{1/2}dx
\end{align*}
Hence, $H^2(P_1, P_2) \le H^2(\mu_1, \mu_2).$
}
\begin{align*}
    \E_{P_1}(T(X)-c)^2+\E_{P_2}(T(X)-c)^2 &= Var_{P_1}T + Var_{P_2}T + (\E_{P_1}T -c)^2 + (\E_{P_2}T -c)^2
\end{align*}
Since the bound holds for any $c$, we can optimize the bound with respect of $c$. The optimal choice $c^*$ to minimize the bound is $c^*=\frac{\E_{P_1}T+\E_{P_2}T}{2}$; hence we obtain
\begin{align*}
    \left(\frac{1-H^2(P_1, P_2)}{2H^2(P_1, P_2)}\right)_+\left|\E_{P_1}T(X)- \E_{P_2}T(X)\right|^2 & \le Var_{P_1}T + Var_{P_2}T. 
\end{align*}
We now analyze the variance term.
\begin{align*}
    Var_{P_1}T &= \E_{P_1}|T(x)-m_1|^2 - |\E_{P_1}T(x) - m_1|^2 \\
    &= \E_{P_1}|T(x)-\psi(\theta)+\psi(\theta)-m_1|^2  - |\E_{P_1}T(x) - m_1|^2 \\ 
    &= \E_{P_1}|T(x)-\psi(\theta)|^2 + \E_{P_1}|\psi(\theta)-m_1|^2  +2\E_{P_1}(\psi(\theta)-m_1)(T(x)-\psi(\theta))- |\E_{P_1}T(x) - m_1|^2 \\
    &= \E_{P_1}|T(x)-\psi(\theta)|^2 + V_1^2 + 2 \iint (\psi(t)T(x)-\psi(t)^2-m_1T(x)+m_1\psi(t))p_t(x)\mu_1(t)\, dx\,dt \\
    &\qquad - |\E_{P_1}T(x) - m_1|^2 \\
    % &= \E_{P_1}|T(x)-\psi(\theta)|^2 + V_1 + 2 \iint (\psi(t)T(x)-\psi(t)^2-m_1T(x)+m_1\psi(t))p_t(x)\mu_1(t)\, dx\,dt \\
    % &\qquad - |\E_{P_1}T(x) - m_1|^2\\
    &= \E_{P_1}|T(x)-\psi(\theta)|^2 + V_1^2 + 2\left(\int (\psi(t)-m_1)\E_t[T(x)]\, \mu_1(t)\, dt\right) -2V_1^2- |\E_{P_1}T(x) - m_1|^2\\
    &= \E_{P_1}|T(x)-\psi(\theta)|^2 - V_1^2 + 2\left(\int \psi(t)\E_t[T(x)]\, \mu_1(t)\, dt\right) - \big\{\E_{P_1}T(x)\big\}^2 - m_1^2 \\
    & =\E_{P_1}|T(x)-\psi(\theta)|^2 - V_1^2 + 2\left(\int \psi(t)\E_t[T(x)]\, \mu_1(t)\, dt\right) - \big\{\E_{P_1}T(x)\big\}^2 - m_1^2 \\
    &\qquad \pm \int \psi(t)^2 \mu_1(t)\, dt \pm \int (\E_t T)^2 \mu_1(t)\, dt\\
    &= \E_{P_1}|T(x)-\psi(\theta)|^2 - \int \left|\psi(t)-\E_{t}[T(x)]\right|^2\mu_1(t)\,dt + \int Var(\E_tT) \, \mu_1(t)\, dt.
\end{align*}
Putting together, we have
\begin{align*}
    & \E_{P_1}|T(x)-\psi(\theta)|^2  + \E_{P_2}|T(x)-\psi(\theta)|^2 \\
    & \qquad \ge \left(\frac{1-H^2(p_1, p_2)}{2H^2(p_1, p_2)}\right)_+\left|\E_{P_1}T(X)- \E_{P_2}T(X)\right|^2 - \int Var(\E_tT) \, \mu_1(t)\, dt - \int Var(\E_tT) \, \mu_2(t)\, dt\\
    &\qquad\qquad+ \int \left|\psi(t)-\E_{t}[T(x)]\right|^2\mu_1(t)\,dt  + \int \left|\psi(t)-\E_{t}[T(x)]\right|^2\mu_2(t)\,dt \\
    & \qquad = \left(\frac{1-H^2(p_1, p_2)}{2H^2(p_1, p_2)}\right)_+\left|\int\E_tT(X) -\psi(t)+\psi(t)\mu_1(t)\,dt- \int \E_tT(X)  -\psi(t)+\psi(t)\mu_2(t)\, dt\right|^2 \\
    &\qquad\qquad+ \int \left|\psi(t)-\E_{t}[T(x)]\right|^2\mu_1(t)\,dt  + \int \left|\psi(t)-\E_{t}[T(x)]\right|^2\mu_2(t)\,dt\\
    &\qquad\qquad- \int Var(\E_tT) \, \mu_1(t)\, dt - \int Var(\E_tT) \, \mu_2(t)\, dt\\
    & \qquad = \left(\frac{1-H^2(p_1, p_2)}{2H^2(p_1, p_2)}\right)_+\left|\int B(t)\mu_1(t)\,dt + m_1- \int B(t)\mu_2(t) \, dt-m_2\right|^2 \\
    &\qquad\qquad+ \int B(t)^2\mu_1(t)\,dt  + \int B(t)^2\mu_2(t)\,dt  - \int Var(\E_tT) \, \mu_1(t)\, dt - \int Var(\E_tT) \, \mu_2(t)\, dt
\end{align*}
{\color{red}\bf Can we follow Cai and Low technique from here, by first deriving a bound that restricts the risk with respect to one prior to be less than $\varepsilon?$}

\clearpage
With slightly more similar approach to \cite{cai2011testing}, we assume that 
\[\E_{P_1}|T(x) - \psi(\theta)|^2 \le \varepsilon^2\]
This does not affect our derivation up to the following part:
\begin{align*}
    &\left(\frac{1-H^2(P_1, P_2)}{2H^2(P_1, P_2)}\right)_+\left|\E_{P_1}T(X)- \E_{P_2}T(X)\right|^2 \le Var_{P_1}T + Var_{P_2}T\\
    &\qquad \implies \left(\frac{1-H^2(P_1, P_2)}{2H^2(P_1, P_2)}\right)_+\left|\int B(t)\mu_1(t)\,dt + m_1- \int B(t)\mu_2(t) \, dt-m_2\right|^2 \le Var_{P_1}T + Var_{P_2}T
\end{align*}
First we observe that by Jensen's inequality, 
\[\int B^2(t)\, \mu_1(dt) = \int |\E_t T(X)-\psi(t)|^2 \, \mu_1(dt) \le \int \E_t |T(X)-\psi(t)|^2 \, \mu_1(dt).\]
Now, we have
\begin{align*}
    Var_{P_1}T &= \int \E_t|T(X)-m_1|^2\, \mu_1(dt) - |\E_{P_1}T - m_1|^2 \\
    &= \int \E_t|T(X)-\psi(t)+\psi(t)-m_1|^2\, \mu_1(dt) - |\E_{P_1}T - m_1|^2 \\
    &= \int \E_t|T(X)-\psi(t)|^2\, \mu_1(dt) + V_1^2 +2\int B(t)|\psi(t)-m_1|\, \mu_1(dt)- |\E_{P_1}T - m_1|^2 \\
    &\le \int \E_t|T(X)-\psi(t)|^2\, \mu_1(dt) + V_1^2\\
    &\qquad +2\left\{\int B^2(t)\, \mu_1(dt)\right\}^{1/2}\left\{\int |\psi(t)-m_1|^2\, \mu_1(dt)\right\}^{1/2}- |\E_{P_1}T - m_1|^2 \\
    &\le \int \E_t|T(x)-\psi(t)|^2\, \mu_1(dt) + V_1^2 +2\left\{\int \E_t |T(X)-\psi(t)|^2 \, \mu_1(dt)\right\}^{1/2} V_1 - |\E_{P_1}T - m_1|^2 \\
    &= \left[\left\{\int \E_t |T(X)-\psi(t)|^2 \, \mu_1(dt)\right\}^{1/2}+V_1\right]^2 - |\E_{P_1}T - m_1|^2 \\
    & \le (\varepsilon + V_1)^2- |\E_{P_1}T - m_1|^2
\end{align*}
Repeating the analogous derivation for $ Var_{P_2}T$, we have
\begin{align*}
    &\left(\frac{1-H^2(P_1, P_2)}{2H^2(P_1, P_2)}\right)_+\left|\int B(t)\,\mu_1(dt) + m_1- \int B(t)\,\mu_2(dt) -m_2\right|^2 \\
    &\qquad \le (\varepsilon + V_1)^2- |\E_{P_1}T - m_1|^2 + \big\{\sqrt{\E_{P_2}|T(X)-\psi(t)|^2} + V_2\big\}^2- |\E_{P_2}T - m_2|^2\\
    &\qquad = (\varepsilon + V_1)^2- \left|\int B(t)\, \mu_1(dt)\right|^2 + \big\{\sqrt{\E_{P_2}|T(X)-\psi(t)|^2} + V_2\big\}^2- \left|\int B(t)\, \mu_2 (dt)\right|^2
\end{align*}
The goal of the successive derivation is to find the lower bound of $\E_{P_2}|T(X)-\psi(t)|^2$ in terms of $\varepsilon$. This hopefully gives us a quadratic function to optimize.

\begin{align*}
    \big\{\sqrt{\E_{P_2}|T(X)-\psi(t)|^2} + V_2\big\}^2&\ge \left(\frac{1-H^2(P_1, P_2)}{2H^2(P_1, P_2)}\right)_+\left|\beta_1 + m_1- \beta_2 -m_2\right|^2 - (\varepsilon + V_1)^2 + \beta_1^2 + \beta_2^2
\end{align*}
where $\beta_i := \int B(t) \, \mu_i(dt)$. Now consider the function
\[\eta(\beta_1, \beta_2) := \left(\frac{1-H^2(P_1, P_2)}{2H^2(P_1, P_2)}\right)_+\left|\beta_1 + m_1- \beta_2 -m_2\right|^2 + \beta_1^2 + \beta_2^2\]
Then the above bound implies 
\[\big\{\sqrt{\E_{P_2}|T(X)-\psi(t)|^2} + V_2\big\}^2 \ge \inf_{\beta_1, \beta_2} \eta(\beta_1, \beta_2)\]
\begin{align*}
    \frac{\partial}{\partial \beta_1}\eta(\beta_1, \beta_2) &= 2\left(\frac{1-H^2(P_1, P_2)}{2H^2(P_1, P_2)}\right)_+\left(\beta_1 + m_1- \beta_2 -m_2\right)+ 2\beta_1 \qquad \text{and}\\
    \frac{\partial}{\partial \beta_2}\eta(\beta_1, \beta_2) &= -2\left(\frac{1-H^2(P_1, P_2)}{2H^2(P_1, P_2)}\right)_+\left(\beta_1 + m_1- \beta_2 -m_2\right)+ 2\beta_2
\end{align*}
The optimal values $\beta_1^*$ and $\beta_2^*$ to set above derivatives zero is given by 
\begin{align*}
    4\left(\frac{1-H^2(P_1, P_2)}{2H^2(P_1, P_2)}\right)_+\left(\beta^*_1 + m_1- \beta^*_2 -m_2\right)+2(\beta^*_1-\beta^*_2) = 0\quad \text{and}\quad \beta_1^* + \beta_2^* = 0.
\end{align*}
Since $\beta_2^* = -\beta_1^*$, we have
\begin{align*}
    &4\left(\frac{1-H^2(P_1, P_2)}{2H^2(P_1, P_2)}\right)_+\left(2\beta^*_1 + m_1 -m_2\right)+4\beta^*_1 = 0\\
    &\qquad \implies 4\left(\frac{2-2H^2(P_1, P_2)+2H^2(P_1, P_2)}{2H^2(P_1, P_2)}\right)_+\beta_1^* + 4\left(\frac{1-H^2(P_1, P_2)}{2H^2(P_1, P_2)}\right)_+\left(m_1 -m_2\right)= 0\\
    &\qquad \implies \beta_1^* = \left(\frac{1-H^2(P_1, P_2)}{2}\right)_+\left(m_2 -m_1\right)
\end{align*}

Furthermore, we have
\begin{align*}
    \frac{\partial^2}{\partial \beta_1^2}\eta(\beta_1, \beta_2) &= 2\left(\frac{1-H^2(P_1, P_2)}{2H^2(P_1, P_2)}\right)_+ + 2 \quad \text{and}\\
    \frac{\partial^2}{\partial \beta_2^2}\eta(\beta_1, \beta_2) &= 2\left(\frac{1-H^2(P_1, P_2)}{2H^2(P_1, P_2)}\right)_++ 2 \quad \text{and}\\
    \frac{\partial^2}{\partial \beta_1\partial\beta_2}\eta(\beta_1, \beta_2) &= -2\left(\frac{1-H^2(P_1, P_2)}{2H^2(P_1, P_2)}\right)_+
\end{align*}
The determinant is hence 
\begin{align*}
    \left\{2\left(\frac{1-H^2(P_1, P_2)}{2H^2(P_1, P_2)}\right)_+ + 2\right\}^2 - \left\{2\left(\frac{1-H^2(P_1, P_2)}{2H^2(P_1, P_2)}\right)_+ \right\}^2 > 0
\end{align*}
and $\frac{\partial^2}{\partial \beta_1^2}\eta(\beta_1, \beta_2) > 0$ for any value of $H^2(P_1, P_2)$. Thus $\eta(\beta_1^*, \beta_2^*)$ is a local minimum. 
\begin{align*}
    &\big\{\sqrt{\E_{P_2}|T(X)-\psi(t)|^2} + V_2\big\}^2 \\
    &\qquad \ge \left(\frac{1-H^2(P_1, P_2)}{2H^2(P_1, P_2)}\right)_+\left(2\beta^*_1 + m_1-m_2\right)^2 - (\varepsilon + V_1)^2 + 2\beta_1^{*2} \\
    &\qquad \ge \left(\frac{1-H^2(P_1, P_2)}{2H^2(P_1, P_2)}\right)_+\left(H^2(P_1, P_2)\left(m_1 -m_2\right)\right)^2 - (\varepsilon + V_1)^2 + \left(\frac{\left\{1-H^2(P_1, P_2)\right\}^2}{2}\right)_+\left(m_2 -m_1\right)^2\\
     &\qquad = \left(\frac{\{1-H^2(P_1, P_2)\}H^2(P_1, P_2)+\left\{1-H^2(P_1, P_2)\right\}^2}{2}\right)_+\left(m_1 -m_2\right)^2 - (\varepsilon + V_1)^2 \\
         &\qquad = \left(\frac{1-H^2(P_1, P_2)}{2}\right)_+\left(m_1 -m_2\right)^2 - (\varepsilon + V_1)^2 
\end{align*}
We thus have 
\begin{align}
    &\big\{\sqrt{\E_{P_2}|T(X)-\psi(t)|^2} + V_2\big\}^2 \ge \left(\frac{1-H^2(P_1, P_2)}{2}\right)_+\left(m_1 -m_2\right)^2 - (\varepsilon + V_1)^2\nonumber\\
    &\implies\E_{P_2}|T(X)-\psi(t)|^2 \ge \left[\left\{\left(\frac{1-H^2(P_1, P_2)}{2}\right)_+\left(m_1 -m_2\right)^2 - (\varepsilon + V_1)^2\right\}_+^{1/2}-V_2\right]^2
\end{align}
Then we have
\begin{align}
    \lambda\varepsilon^2  + (1-\lambda)\E_{P_2}|T(X)-\psi(t)|^2 \ge \lambda\varepsilon^2 + (1-\lambda)\left[\left\{\left(\frac{1-H^2(P_1, P_2)}{2}\right)_+\left(m_1 -m_2\right)^2 - (\varepsilon + V_1)^2\right\}_+^{1/2}-V_2\right]^2\nonumber
\end{align}

We now need to optimize for 
\[\lambda x^2 + (1-\lambda)\left[\left\{A-(x+B)^2\right\}_+^{1/2}-C\right]^2\]

\kt{\cite{cai2011testing} solves the minimum of the RHS in terms of $\varepsilon^*$}

\kt{Another idea is to use $Var_{P_2}T$ without the upper bound:
\[Var_{P_2}T =\E_{P_2}|T(x)-\psi(\theta)|^2 - \int B^2(t)\mu_2(t)\,dt + \int Var(\E_tT) \, \mu_2(t)\, dt.\]
and this may lead to
\begin{align*}
    &\left(\frac{1-H^2(P_1, P_2)}{2H^2(P_1, P_2)}\right)_+\left|\int B(t)\,\mu_1(dt) + m_1- \int B(t)\,\mu_2(dt) -m_2\right|^2 \\
    &\qquad \le  (\varepsilon + V_1)^2- \left|\int B(t)\, \mu_1(dt)\right|^2 + \E_{P_2}|T(x)-\psi(\theta)|^2- \left|\int B(t)\, \mu_2 (dt)\right|^2+ \int Var(\E_tT) \, \mu_2(t)\, dt
\end{align*}
which could be better since $\E_{P_2}|T(x)-\psi(\theta)|^2$ appears itself.
}
\clearpage
Alt. Attempt 1:
Recall we have
\begin{align*}
    Var_{P_2}T &= \E_{P_2}|T(x)-m_1|^2 - |\E_{P_2}T(x) - m_1|^2 \\
    &= \E_{P_2}|T(x)-\psi(\theta)+\psi(\theta)-m_2|^2  - |\E_{P_2}T(x) - m_2|^2 \\ 
    &= \E_{P_2}|T(x)-\psi(\theta)|^2 + \E_{P_2}|\psi(\theta)-m_2|^2  +2\E_{P_2}(\psi(\theta)-m_2)(T(x)-\psi(\theta))- |\E_{P_2}T(x) - m_2|^2 
\end{align*}
Now consider the last two terms:
\begin{align*}
    2\E_{P_2}(\psi(\theta)-m_2)(T(x)-\psi(\theta)) &= 2 \iint (\psi(t)T(x)-\psi(t)^2-m_2T(x)+m_2\psi(t))p_t(x)\mu_2(t)\, dx\,dt \\
    &= 2\left(\int (\psi(t)-m_2)\E_t[T(x)]\, \mu_2(t)\, dt\right) -2V_1^2\\
    &= 2\int \psi(t)\E_t[T(x)]\, \mu_2(t)\, dt -2m_2 \E_{P_2}T(x) -2V_1^2
\end{align*}
and 
\begin{align*}
    |\E_{P_2}T(x) - m_2|^2 &= \big\{\E_{P_2}T(x)\big\}^2 - 2m_2 \E_{P_2}T(x)+ m_2^2.
\end{align*}
This gives us that 
\begin{align*}
    &2\E_{P_2}(\psi(\theta)-m_2)(T(x)-\psi(\theta))- |\E_{P_2}T(x) - m_2|^2 \\
    &\qquad = 2\int \psi(t)\E_t[T(x)]\, \mu_2(t)\, dt -2m_2 \E_{P_2}T(x) -2V_2^2 -\big\{\E_{P_2}T(x)\big\}^2 +2m_2 \E_{P_2}T(x)- m_2^2\\
    &\qquad = 2\int \psi(t)\E_t[T(x)]\, \mu_2(t)\, dt -2V_2^2 -\big\{\E_{P_2}T(x)\big\}^2 - m_2^2 \pm \int \psi(t)^2 \mu_2(t)\, dt \pm \int (\E_t T)^2 \mu_2(t)\, dt \\
    &\qquad = -\int \{\E_t T(x) - \psi(t)\}^2\, \mu_2(dt) -2V_2^2 -\big\{\E_{P_2}T(x)\big\}^2 - m_2^2 + \int \psi(t)^2 \, \mu_2(dt) + \int (\E_t T)^2 \, \mu_2(dt)\\
    &\qquad = -\int B^2(t) \, \mu_2(dt) - V_2^2  + Var_{\mu_2}\E_t T
\end{align*}
Putting together, we have 
\begin{align}
    Var_{P_2}T &= \E_{P_2}|T(x)-\psi(\theta)|^2 -\int B^2(t) \, \mu_2(dt)  + Var_{\mu_1}\E_t T \nonumber\\
    &\le \E_{P_2}|T(x)-\psi(\theta)|^2 - \left(\int B(t) \, \mu_2(dt)\right)^2  + Var_{\mu_2}\E_t T\label{eq:var_bound1}
\end{align}
In contrast, the result by \cite{cai2011testing} says
\begin{align}
    Var_{P_2}T \le \left(\sqrt{\E_{P_2}|T(x)-\psi(\theta)|^2} + V_2 \right)^2 - \left(\int B(t) \, \mu_2(dt)\right)^2   \label{eq:var_bound2}
\end{align}

Letting $\beta_i := \int B(t) \, \mu_i(dt)$ and using \eqref{eq:var_bound1} for both terms, we get
\begin{align*}
    &\left(\frac{1-H^2(P_1, P_2)}{2H^2(P_1, P_2)}\right)_+\left|\beta_1 + m_1- \beta_2 -m_2\right|^2 \\
    & \qquad \le Var_{P_1}T + Var_{P_2}T \\ 
    & \qquad \le \E_{P_2}|T(x)-\psi(\theta)|^2 - \beta_2^2  + Var_{\mu_2}\E_t T + \varepsilon^2 - \beta_1^2  + Var_{\mu_1}\E_t T \\
    &\implies \E_{P_2}|T(x)-\psi(\theta)|^2 \\
    &\qquad\qquad\ge \left(\frac{1-H^2(P_1, P_2)}{2H^2(P_1, P_2)}\right)_+\left|\beta_1 + m_1- \beta_2 -m_2\right|^2 - \varepsilon^2 + \beta_1^2 + \beta_2^2 - Var_{\mu_1}\E_t T - Var_{\mu_2}\E_t T 
\end{align*}
As shown, the function 
\[\eta(\beta_1, \beta_2) := \left(\frac{1-H^2(P_1, P_2)}{2H^2(P_1, P_2)}\right)_+\left|\beta_1 + m_1- \beta_2 -m_2\right|^2 + \beta_1^2 + \beta_2^2\]
attains local minimum at 
\[\beta_1^* = -\beta_2^* = \left(\frac{1-H^2(P_1, P_2)}{2}\right)_+\left(m_2 -m_1\right)\]
and 
\[\eta(\beta_1^*, \beta_2^*) = \left(\frac{1-H^2(P_1, P_2)}{2}\right)_+\left(m_1 -m_2\right)^2.\]
We thus have
\begin{align*}
    \E_{P_2}|T(x)-\psi(\theta)|^2 \ge \left(\frac{1-H^2(P_1, P_2)}{2}\right)_+\left(m_1 -m_2\right)^2 - \varepsilon^2 - Var_{\mu_1}\E_t T - Var_{\mu_2}\E_t T.
\end{align*}
For $\lambda \in [0,1]$, we have the following relationship:
\begin{align*}
    \lambda \varepsilon^2 + (1-\lambda)\E_{P_2}|T(x)-\psi(\theta)|^2 \ge \lambda\varepsilon^2 + (1-\lambda)(A-\varepsilon^2)
\end{align*}
where 
\[A:=\left(\frac{1-H^2(P_1, P_2)}{2}\right)_+\left(m_1 -m_2\right)^2- Var_{\mu_1}\E_t T - Var_{\mu_2}\E_t T\]
Consider the quadratic, 
\[J(x) := \lambda x^2 + (1-\lambda) (A-x^2), J'(x) = 2(2\lambda-1)x,  J''(x) = 2(2\lambda-1)\]
The global minimum is attained when $x=0$ for $\lambda \ge 1/2$. This concludes that 
\begin{align}
    \lambda \varepsilon^2 + (1-\lambda)\E_{P_2}|T(x)-\psi(\theta)|^2 \ge \left(\frac{1-H^2(P_1, P_2)}{4}\right)_+\left(m_1 -m_2\right)^2- \frac{Var_{\mu_1}\E_t T + Var_{\mu_2}\E_t T}{2}
\end{align}
for any $\varepsilon$. 
\clearpage
Alt. Attempt 2:
Letting $\beta_i := \int B(t) \, \mu_i(dt)$ and using \eqref{eq:var_bound1} for $Var_{P_2} T$ and \eqref{eq:var_bound2} for $Var_{P_1} T$, we get
\begin{align*}
    &\left(\frac{1-H^2(P_1, P_2)}{2H^2(P_1, P_2)}\right)_+\left|\beta_1 + m_1- \beta_2 -m_2\right|^2 \\
    & \qquad \le Var_{P_1}T + Var_{P_2}T \\ 
    & \qquad \le \E_{P_2}|T(x)-\psi(\theta)|^2 - \beta_2^2  + Var_{\mu_2}\E_t T + (\varepsilon + V_1)^2 - \beta_1^2\\
    &\implies \E_{P_2}|T(x)-\psi(\theta)|^2 \\
    &\qquad\qquad\ge \left(\frac{1-H^2(P_1, P_2)}{2H^2(P_1, P_2)}\right)_+\left|\beta_1 + m_1- \beta_2 -m_2\right|^2 + \beta_1^2 + \beta_2^2 - (\varepsilon+V_1)^2 - Var_{\mu_2}\E_t T 
\end{align*}
Using the identical minimization over $\beta_1$ and $\beta_2$ as before, we have
\begin{align*}
    \E_{P_2}|T(x)-\psi(\theta)|^2 \ge \left(\frac{1-H^2(P_1, P_2)}{2}\right)_+\left(m_1 -m_2\right)^2 - (\varepsilon+V_1)^2 - Var_{\mu_2}\E_t T.
\end{align*}
For $\lambda \in [0,1]$, we have the following relationship:
\begin{align*}
    \lambda \varepsilon^2 + (1-\lambda)\E_{P_2}|T(x)-\psi(\theta)|^2 \ge \lambda\varepsilon^2 + (1-\lambda)\{A-(\varepsilon+B)^2\}
\end{align*}
where 
\[A:=\left(\frac{1-H^2(P_1, P_2)}{2}\right)_+\left(m_1 -m_2\right)^2- Var_{\mu_2}\E_t T\quad \text{and}\quad B:=V_1\]
Consider the quadratic, 
\[J(x) := \lambda x^2 + (1-\lambda)\{A-(x+B)^2\}\]
whose local minimum is attained at $x^* = \frac{B(\lambda-1)}{1-2\lambda}$ for $\lambda \ge 1/2$. This follows since 
\begin{align*}
    J'(x) = 2\lambda x - 2(1-\lambda)(x+B) = 2\lambda x - 2(x+B-\lambda x - \lambda B) =  4\lambda x -2x -2B + 2\lambda B
\end{align*}
and we have 
\begin{align*}
    2\lambda x^* -x^* -B + \lambda B = 0 \implies (\lambda -1) B = (1-2\lambda) x^*.
\end{align*}
Also we have $J''(x) = -2+4\lambda$ and thus $J''(x) \ge 0$ when $\lambda \ge 1/2$. This concludes that 
\begin{align}
    \lambda \varepsilon^2 + (1-\lambda)\E_{P_2}|T(x)-\psi(\theta)|^2 &\ge \lambda \left(\frac{B(\lambda-1)}{1-2\lambda}\right)^2 + (1-\lambda)\left\{A-\left(\frac{B(\lambda-1)}{1-2\lambda}+B\right)^2\right\}\nonumber\\
    &= \lambda \left(\frac{B(\lambda-1)}{1-2\lambda}\right)^2 + (1-\lambda)\left\{A-\left(\frac{B(\lambda-1)+B(1-2\lambda)}{1-2\lambda}\right)^2\right\}\nonumber\\
    &= \lambda \left(\frac{B(\lambda-1)}{1-2\lambda}\right)^2 + (1-\lambda)\left\{A-\left(\frac{-\lambda B}{1-2\lambda}\right)^2\right\}\nonumber\\
    &= (1-\lambda)A + \frac{\lambda B^2(\lambda-1)^2-(1-\lambda)\lambda^2B^2}{(1-2\lambda)^2}\nonumber\\
    &= (1-\lambda)A + \frac{\lambda B^2(1-\lambda)\{(1-\lambda)-\lambda\}}{(1-2\lambda)^2}\nonumber\\
    &= (1-\lambda)A + \frac{\lambda B^2(1-\lambda)}{1-2\lambda}
\end{align}
for any $\varepsilon$. \kt{From here, I tried to pick $\lambda$ so it balances $(1-\lambda)A$ and $\frac{\lambda B^2(1-\lambda)}{1-2\lambda}$, but such $\lambda$ is $\frac{A}{B^2 + 2A}$, which is smaller than $1/2$}
\clearpage
Alt. Attempt 3:
Recall we have
\begin{align*}
    Var_{P_2}T &= \E_{P_2}|T(x)-m_1|^2 - |\E_{P_2}T(x) - m_1|^2 \\
    &= \E_{P_2}|T(x)-\psi(\theta)+\psi(\theta)-m_2|^2  - |\E_{P_2}T(x) - m_2|^2 \\ 
    &= \E_{P_2}|T(x)-\psi(\theta)|^2 + \E_{P_2}|\psi(\theta)-m_2|^2  +2\E_{P_2}(\psi(\theta)-m_2)(T(x)-\psi(\theta))- |\E_{P_2}T(x) - m_2|^2 \\
    & \le \E_{P_2}|T(x)-\psi(\theta)|^2 + \E_{P_2}|\psi(\theta)-m_2|^2  +\E_{P_2}L(\psi(\theta)-m_2)^2+\E_{P_2}L^{-1}(T(x)-\psi(\theta))^2\\
    &\qquad- |\E_{P_2}T(x) - m_2|^2 \\
    & = (1+L)\E_{P_2}|T(x)-\psi(\theta)|^2 + (1+1/L)V_2^2- \left|\int B(t) \, \mu_2(dt)\right|^2
\end{align*}
Letting $\beta_i := \int B(t) \, \mu_i(dt)$ and using \eqref{eq:var_bound2} for $Var_{P_1} T$, we get
\begin{align*}
    &\left(\frac{1-H^2(P_1, P_2)}{2H^2(P_1, P_2)}\right)_+\left|\beta_1 + m_1- \beta_2 -m_2\right|^2 \\
    & \qquad \le Var_{P_1}T + Var_{P_2}T \\ 
    & \qquad \le (1+L)\E_{P_2}|T(x)-\psi(\theta)|^2 + (1+1/L)V_2^2- \left|\int B(t) \, \mu_2(dt)\right|^2 + (\varepsilon + V_1)^2 - \beta_1^2\\
    &\implies \E_{P_2}|T(x)-\psi(\theta)|^2 \\
    &\qquad\qquad\ge \frac{1}{(1+L)}\left[\left(\frac{1-H^2(P_1, P_2)}{2H^2(P_1, P_2)}\right)_+\left|\beta_1 + m_1- \beta_2 -m_2\right|^2 + \beta_1^2 + \beta_2^2 -(1+1/L)V_2^2- (\varepsilon+V_1)^2 \right] \\
    &\qquad\qquad\ge \frac{1}{(1+L)}\left[\left(\frac{1-H^2(P_1, P_2)}{2}\right)_+\left(m_1 -m_2\right)^2 -(1+1/L)V_2^2- (\varepsilon+V_1)^2 \right] 
\end{align*}

For $\lambda \in [0,1]$, we have the following relationship:
\begin{align*}
    \lambda \varepsilon^2 + (1-\lambda)\E_{P_2}|T(x)-\psi(\theta)|^2 \ge \lambda\varepsilon^2 + \frac{1-\lambda}{1+L}\{A-(\varepsilon+B)^2\}
\end{align*}
where 
\[A_L:=\left(\frac{1-H^2(P_1, P_2)}{2}\right)_+\left(m_1 -m_2\right)^2-(1+1/L)V_2^2\quad \text{and}\quad B:=V_1\]
Consider the quadratic, 
\[J(x) := \lambda x^2 + \frac{1-\lambda}{1+L}\{A_L-(x+B)^2\}\]
