# Supplementary material for: Generalized van Trees inequality: Local minimax bounds for non-smooth functionals and irregular statistical models
Source: arXiv:2405.06437 source file (2024-10-19)
Supplement: Supplementary file 7 [file mle_proj.tex]

\clearpage
\section{Projection of Gaussian mean}
\subsection{Proof of Corollary~\ref{cor:gaussian_proj} \kt{Almost done}}
\begin{proof}
We consider a statistical model $\{P_\theta : \theta \in \mathbb{R}\}$ where $P_\theta$ is a collection of Gaussian distributions given by $N(\theta, \sigma^2)$ with known variance $\sigma^2 > 0$.
Similar to the proof of Corollary~\ref{cor:crvt_lam}, we define a random variable $\vartheta := \theta_0 + cn^{-1/2}T$ where $T \in (-1,1)$. The density function of $T$ is give by bounded and absolutely continuous function $q$. For each $t \in T$, the density of $\vartheta$ is then given by $q_{\theta_0, n,c}(\vartheta) :=  \frac{n^{1/2}}{c}q\left(\frac{n^{1/2}(t-\theta_0)}{c}\right)$. The assumption~\ref{as:IPBorder} is satisfied for given $c$ when $n$ is large enough.
First we consider the case when $\theta_0 < a$. The analogous argument holds for $b < \theta_0$. In this case, the functional $\Pi_{[a,b]}(\theta)$ is continuously differentiable at $\theta_0$ for $n$ large enough with its derivative zero. Hence we can apply Remark~\ref{remark:univariate_van_trees} and obtain
\begin{align*}
    \sup_{|t|<1} \E^n_{\theta_0 + tcn^{-1/2}}\left[n^{1/2}\left\{T(x)-\psi(\theta_0+tcn^{-1/2})\right\}\right]^2 &\ge \frac{\left(\int_{\mathcal{B}_p([0], 1)}\psi'(\theta_0+ tcn^{-1/2})\, q(t)\, dt\right)^2}{\frac{1}{c^2} \mathcal{J}(q) + \int_{\mathcal{B}_p([0], 1)}\mathcal{I}(\theta_0 + tcn^{-1/2})q(t)\, dt} = 0.
\end{align*}

Next we consider the case $a < \theta_0 < b$. Since the functional $\Pi_{[a,b]}(\theta)$ is continuously differentiable at $\theta_0$ for $n$ large enough, Remark~\ref{remark:univariate_van_trees} implies
\begin{align*}
    \sup_{|t|<1} \E^n_{\theta_0 + tcn^{-1/2}}\left[n^{1/2}\left\{T(x)-\psi(\theta_0+tcn^{-1/2})\right\}\right]^2 &\ge \frac{1}{\frac{1}{c^2} \mathcal{J}(q) + \int_{\mathcal{B}_p([0], 1)}\mathcal{I}(\theta_0 + tcn^{-1/2})q(t)\, dt} \\
    &=\frac{1}{\frac{1}{c^2} \mathcal{J}(q) + 1/\sigma^2}.
\end{align*}
The inequality above holds for any density function $q$ over $[-1,1]$ that satisfies assumptions. Therefore, the supremum over $q$ on the right-hand side can be attained by minimizing Fisher information $\mathcal{J}(q)$. Moreover, it can be shown that the smallest Fisher information among all the densities $q$ supported on $[-1,1]$ is $\pi^2$. The corresponding density function is given by 
\[q(t) = \frac{1}{2}q_0\left(\frac{t-\theta_0}{2}\right)\, \text{ where }\, q_0(t) = \cos^2(\pi t/2)I(|t|\le1).\]
We refer the reader \cite{bercher2009minimum} for additional details. We thus conclude 
\begin{align*}
    \sup_{|t|<1} \E^n_{\theta_0 + tcn^{-1/2}}\left[n^{1/2}\left\{T(x)-\psi(\theta_0+tcn^{-1/2})\right\}\right]^2 &\ge \frac{1}{\pi^2/c^2+ 1/\sigma^2}
\end{align*}
for $a < \theta_0 < b$.

Finally, we consider the case $\theta_0 = a$. The functional $\Pi_{[a,b]}(\theta)$ is no longer continuously differentiable, and thus we will apply Theorem~\ref{thm:crvtBound} to the density function $q_{\theta_0, n,c}(\vartheta)$. Now we obtain 
\begin{align*}
   & \int_{\mathbb{R}}\E^n_{\theta}\left\{T(x)-\Pi_{[a,b]}(\theta)\right\}^2q_{\theta_0, n,c}(\theta)\, d\theta \ge  \sup_{ |h|<\delta}\frac{\left\{\int_{\mathbb{R}} \left(\Pi_{[a,b]}(\theta)-\Pi_{[a,b]}(\theta-h)\right)q_{\theta_0, n,c}(\theta)\,d\theta\right\}^2}{\chi^2(Q_{h}\|Q)+\int_{\mathbb{R}} \frac{q_{\theta_0, n,c}(\theta+h)^2}{q_{\theta_0, n,c}(\theta)}\chi^2(P^n_{\theta+h}\|P^n_\theta)\,d\theta}.
\end{align*}
\kt{TODO: show this result}
\begin{align*}
    \lim_{\varepsilon_n\to 0}\varepsilon_n^{-2}\chi^2(Q_{u\varepsilon_n}\|Q) &= \frac{n}{c^2}u^T\mathcal{J}(q)u\\
    \lim_{\varepsilon_n\to 0}\varepsilon_n^{-2}\int_{\mathbb{R}} \frac{q_{\theta_0, n,c}(\theta+u\varepsilon_n)^2}{q_{\theta_0, n,c}(\theta)}\chi^2(P^n_{\theta+u\varepsilon_n}\|P^n_\theta)\,d\theta &=n\int_{-1}^1 \mathcal{I}(\theta_0 + tcn^{-1/2})q(t)\, dt = \frac{n}{\sigma^2}
\end{align*}
The standard local asymptotic minimax theorem fails for this functional when $\theta_0=a$ since the projection $\Pi_{[a,b]}$ is not continuously differentiable on the boundary. The numerator 
\begin{align*}
&\lim_{\varepsilon_n\to 0}\int_{-1}^1\varepsilon_n^{-1}\left\{\Pi_{[a,b]}(\theta)-\Pi_{[a,b]}(\theta-u\varepsilon_n)\right\}q_{\theta_0, n,c}(\theta)\, d\theta\\
&\qquad=\lim_{\varepsilon_n\to 0}\int_{-1}^1\varepsilon_n^{-1}\left\{\Pi_{[a,b]}(a+ tcn^{-1/2})-\Pi_{[a,b]}(a+ tcn^{-1/2}-u\varepsilon_n)\right\}q(t)\, dt.
\end{align*}
For a fixed $c > 0$, we assume that $n$ is a large constant so that $|cn^{-1/2}| +|\delta| < |b-a|$.
We first observe that 
\begin{align*}
    \Pi_{[a,b]}\left(a+ctn^{-1/2}\right) &= \begin{cases}
    a+ctn^{-1/2}, & \text{for } t \ge 0 \\
    a, & \text{for } t < 0
    \end{cases}\\
    &= aI(t < 0) + \left(a + ctn^{-1/2}\right)I(t \ge 0)\\
    & = a+ ctn^{-1/2}I(t \ge 0)
\end{align*}
and similarly,
\begin{align*}
    \Pi_{[a,b]}\left(a-u\varepsilon_n+ctn^{-1/2}\right) &= \begin{cases}
    a-u\varepsilon_n + ctn^{-1/2}, & \text{for } t \ge \frac{u\varepsilon_nn^{1/2}}{c} \\
    a, & \text{for } t < \frac{u\varepsilon_nn^{1/2}}{c}
    \end{cases}\\
    &=aI\left(t < \frac{u\varepsilon_nn^{1/2}}{c}\right) + \left(a - u\varepsilon_n + ctn^{-1/2}\right)I\left(t \ge \frac{u\varepsilon_nn^{1/2}}{c}\right)\\
    &= a + \left( ctn^{-1/2}-u\varepsilon_n \right)I\left(t \ge \frac{u\varepsilon_nn^{1/2}}{c}\right).
\end{align*}

For a univariate functional, there are only two possible $u$: $u=1$ or $u=-1$. Thus the supremum over $|h| < \delta$ reduces to analyzing the limit of two cases.

First we assume $u = 1$. Then it follows $I\left(t \ge \frac{u\varepsilon_nn^{1/2}}{c}\right) \implies I(t \ge 0)$ and we have
\begin{align*}
    \Pi_{[a,b]}\left(a+ctn^{-1/2}\right) - \Pi_{[a,b]}\left(a-u\varepsilon_n+ctn^{-1/2}\right) &= ctn^{-1/2}I(t \ge 0) - \left( ctn^{-1/2}-\varepsilon_n  \right)I\left(t \ge \frac{\varepsilon_nn^{1/2}}{c}\right)\\
     &= \varepsilon_n I\left(t \ge \frac{\varepsilon_nn^{1/2}}{c}\right) +ctn^{-1/2}I\left(\frac{\varepsilon_nn^{1/2}}{c} > t \ge 0\right).
\end{align*}
and therefore
\begin{align}
    &\int^1_{-1}\varepsilon_n^{-1} \left\{\Pi_{[a,b]}\left(a+ctn^{-1/2}\right)-\Pi_{[a,b]}\left(a-\varepsilon_n+ctn^{-1/2}\right)\right\}q\left(t\right)\,dt \nonumber
    \\&\qquad =\int^1_{-1}I\left(t \ge \frac{\varepsilon_nn^{1/2}}{c}\right)q(t)\, dt + \frac{c}{\varepsilon_nn^{1/2}}\int^1_{-1}t I\left(\frac{\varepsilon_nn^{1/2}}{c} > t \ge 0\right)q(t)\,dt\nonumber\\
    &\qquad =\int^1_{\frac{\varepsilon_nn^{1/2}}{c}}q(t)\, dt + \frac{c}{\varepsilon_nn^{1/2}}\int^{\frac{\varepsilon_nn^{1/2}}{c}}_{0}t q(t)\,dt\nonumber.
\end{align}
By taking $\varepsilon_n \to 0$, we conclude
\[\lim_{\varepsilon_n \to 0}\varepsilon_n^{-1}\int^1_{-1} \left\{\Pi_{[a,b]}\left(a+ctn^{-1/2}\right)-\Pi_{[a,b]}\left(a-\varepsilon_n+ctn^{-1/2}\right)\right\}q\left(t\right)\,dt = \int_0^1 q(t)\,dt.\]

Next, we consider the case when $u = -1$. In this case, $I(t \ge 0)\implies I(t\ge \frac{u\varepsilon_nn^{1/2}}{c})$ and thus we have
\begin{align*}
    \Pi_{[a,b]}\left(a+ctn^{-1/2}\right) - \Pi_{[a,b]}\left(a+\varepsilon_n+ctn^{-1/2}\right) 
    &= \varepsilon_n I\left(t \ge 0\right) -\left(\varepsilon_n+ctn^{-1/2}\right)I\left(0 > t \ge \frac{-\varepsilon_nn^{1/2}}{c}\right)\\
    &=\varepsilon_n I\left(t \ge \frac{-\varepsilon_nn^{1/2}}{c}\right) -ctn^{-1/2}I\left(0 > t \ge \frac{-\varepsilon_nn^{1/2}}{c}\right).
\end{align*}
Hence we have 
\begin{align}
    &\varepsilon_n^{-1}\int^1_{-1} \left\{\Pi_{[a,b]}\left(a+ctn^{-1/2}\right)-\Pi_{[a,b]}\left(a+\varepsilon_n+ctn^{-1/2}\right)\right\}q\left(t\right)\,dt \nonumber
    \\&\qquad =\int^1_{-1}I\left(t \ge \frac{-\varepsilon_nn^{1/2}}{c}\right)q(t)\, dt - \frac{c}{\varepsilon_nn^{1/2}}\int^1_{-1}t I\left(0 > t \ge \frac{-\varepsilon_nn^{1/2}}{c}\right)q(t)\,dt\nonumber\\
    &\qquad =\int^1_{\frac{-\varepsilon_nn^{1/2}}{c}}q(t)\, dt - \frac{c}{\varepsilon_nn^{1/2}}\int_{\frac{-\varepsilon_nn^{1/2}}{c}}^{0}t q(t)\,dt\nonumber.
\end{align}
By taking $\varepsilon_n \to 0$, we conclude
\[\lim_{\varepsilon_n \to 0}\varepsilon_n^{-1}\int^1_{-1} \left\{\Pi_{[a,b]}\left(a+ctn^{-1/2}\right)-\Pi_{[a,b]}\left(a+\varepsilon_n+ctn^{-1/2}\right)\right\}g\left(t\right)\,dt = \int_0^1 q(t)\,dt.\]

For a projection operator, the direction at which we take the limit does not change the numerator of the lower bound. Then the associated lower bound for a projection operator is given by
\begin{align*}
  & \sup_{|t|<1} \E^n_{\theta_0 + tcn^{-1/2}}\left[n^{1/2}\left\{T(x)-\Pi_{[a,b]}(a+tcn^{-1/2})\right\}\right]^2\ge \sup_{q}\frac{\left(\int_0^1 q(t)\,dt\right)^2}{\frac{1}{c^2}\mathcal{J}(q)+\int_{-1}^1\mathcal{I}(a + tcn^{-1/2})q(t)\,dt}.
\end{align*}

We can obtain the lower bound for $\theta_0 = b$ using an analogous argument. This concludes the claim.  
\end{proof}
% \begin{remark}
% As with the local asymptotic minimax theorem, if we take $\liminf{c\to+\infty}\liminf_{n\to+\infty}$ to both sides of the expression, it yields
% \begin{align*}
%   & \liminf_{c\to+\infty}\liminf_{n\to+\infty}\inf_{S_n}\sup_{|t|<1} \E_{a + tcn^{-1/2}}\left[n^{1/2}\left\{T(x)-\psi(\theta_0+tcn^{-1/2})\right\}\right]^2\ge \sup_{g}\frac{\{\int_0^1 q(t)\,dt\}^2}{\mathcal{I}(a)}
% \end{align*}
% We can further lower bound the expression by studying the case when density $g$ is given by $g(u) = 2\cos^2(\pi (u - 1/2))I(0 \le u \le1)$. This gives us
% \begin{align*}
%   & \liminf_{c\to+\infty}\liminf_{n\to+\infty}\inf_{S_n}\sup_{|t|<1} \E_{a + tcn^{-1/2}}\left[n^{1/2}\left\{T(x)-\psi(\theta_0+tcn^{-1/2})\right\}\right]^2\ge \frac{1}{\mathcal{I}(a)}.
% \end{align*}
% This is not a reasonable bound since the plug-in estimator of projection by a sample mean gives the risk of $\frac{1}{2\mathcal{I}(a)}$ at $\theta=a$. 
% \end{remark}

\clearpage
\subsection{Optimization under absolute moment constraints \kt{Done}}
% Corollary~\ref{cor:gaussian_proj} involves the following optimization over density functions:
% \[ \sup_q \frac{\left(\int_0^1q(t)\, dt\right)^2}{\mathcal{J}(q)/c^2+1/\sigma^2}.\]

\begin{corollary}\label{cor:ode}
\begin{align*}
    \sup_q \frac{\left(\int_0^1q(t)\, dt\right)^2}{\mathcal{J}(q)/c^2+1/\sigma^2} \ge \sup_{a \in [0,1]} \frac{a^2}{\{\pi(1+|\eta^{-1}(2a-1)|)\}^2/c^2+1/\sigma^2}
\end{align*}
where $\eta(t) = t -\sin(-\pi t)/\pi$.
\end{corollary}
\begin{proof}[\bfseries{Proof of Corollary~\ref{cor:ode}}]
First, we obverse that the following optimization is equivalent:
\begin{align*}
    \sup_q \frac{\left(\int_0^1q(t)\, dt\right)^2}{\mathcal{J}(q)/c^2+1/\sigma^2} = \sup_{a \in [0,1]}\sup_{\left\{q : \int_0^1 q(t)\, dt=a\right\}} \frac{a^2}{\mathcal{J}(q)/c^2+1/\sigma^2}.
\end{align*}
For each $a$, the supremum of the right-hand side is attained by minimizing Fisher information $\mathcal{J}(q)$ subject to the constraint $\int_0^1 q(t)\, dt=a$. We thus need to solve the following optimization:
\[
\inf_q\int_{-1}^1 \frac{\{q'(t)\}^2}{q(t)}dt,\mbox{ subject to }\int_0^1 q(t)\, dt = a
\]
where the infimum is over all absolutely continuous density function with its support $[\delta_-, \delta_+] \subseteq [-1,1]$. Using the Euler–Lagrange equation, Theorem 2.1 of~\cite{ernst2017minimizing} shows that the optimal $q$ for the above expression also satisfies
\[
-2\dot{\nu}(x) - \nu^2(x) = B_1I\{\delta_- \le x \le 0\} + B_2I\{0 \le x\le \delta_+\}
\]
where $\nu(t) = q'(t)/q(t)$ and $B_1, B_2$ are some constants. The general solution of this first-order non-homogeneous ODE is given by 
\begin{align*}
    \nu(x) = \begin{cases}
        \sqrt{B_1}\tan\left(\frac{\sqrt{B_1}}{2}(c_1-x)\right) & \text{where } \delta_- \le x \le 0\\
        \sqrt{B_2}\tan\left(\frac{\sqrt{B_2}}{2}(c_2-x)\right) & \text{where } 0 \le x \le \delta_+.
    \end{cases}
\end{align*}
By definition, we have $\nu(t) = q'(t)/q(t)$ and thus the general solution $q$ is given by 

% \begin{align*}
%     g'(x)/g(x) = \begin{cases}
%         \sqrt{B_1}\tan\left(\frac{\sqrt{B_1}}{2}(c_1-x)\right) & \text{where } -1 \le x \le 0\\
%         \sqrt{B_2}\tan\left(\frac{\sqrt{B_2}}{2}(c_2-x)\right) & \text{where } 0 \le x \le 1
%     \end{cases}
% \end{align*}
\begin{align*}
    q(x) = \begin{cases}
        \widetilde{C_1}\cos^2\left(\frac{\sqrt{B_1}}{2}(x-c_1)\right) & \text{where } \delta_- \le x \le 0\\
        \widetilde{C_2}\cos^2\left(\frac{\sqrt{B_2}}{2}(x-c_2)\right) & \text{where } 0 \le x \le \delta_+.
    \end{cases}
\end{align*}
It thus remains to solve the initial value problem. The solution $q$ must satisfy the following:
\begin{enumerate}
    \item Since $q(\delta_{-})=0$, we have
    \begin{align}
        \widetilde{C_1}\cos^2\left(\frac{\sqrt{B_1}}{2}(\delta_{-}-c_1)\right)=0 \implies \sqrt{B_1}(\delta_{-}-c_1)=\pm (2n_1+1)\pi\label{constraint:g(delta-)}\nonumber
    \end{align}
    where $n_1 \in \mathbb{N}$. Similarly  $q(\delta_{+})=0$ gives
    \begin{equation}
        \widetilde{C_2}\cos^2\left(\frac{\sqrt{B_2}}{2}(\delta_{+}-c_2)\right)=0 \implies \sqrt{B_2}(\delta_{+}-c_2)=\pm (2n_2+1)\pi\label{constraint:g(delta+)}\nonumber
    \end{equation}
    where $n_2 \in \mathbb{N}$.
    \item Since $q$ is absolutely continuous at zero, we have
    \begin{align}
        q(0) = \widetilde{C_1}\cos^2\left(-\frac{c_1\sqrt{B_1}}{2}\right)= \widetilde{C_2}\cos^2\left(-\frac{c_2\sqrt{B_2}}{2}\right).\nonumber
        % \label{constraint:g(0)}
    \end{align}
    Also $q'$ must be continuous at zero. This gives
    \begin{align*}
        q'(0) = \widetilde{C_1}\sqrt{B_1}\cos\left(-\frac{c_1\sqrt{B_1}}{2}\right)\sin\left(-\frac{c_1\sqrt{B_1}}{2}\right)=\widetilde{C_2}\sqrt{B_2}\cos\left(-\frac{c_2\sqrt{B_2}}{2}\right)\sin\left(-\frac{c_2\sqrt{B_2}}{2}\right).\nonumber
        % \label{constraint:g'(0)}
    \end{align*}
    \item By the constraint $\int_0^{\delta_+} q(t)\, dt =a$, we have
    \begin{align*}
     \widetilde{C_2}\int_{0}^{\delta_+}\cos^2\left(\frac{\sqrt{B_2}}{2}(x-c_2)\right) \, dt = \frac{\widetilde{C_2}\delta_{+}}{2} - \frac{\widetilde{C_2}}{2\sqrt{B_2}}\sin(-c_2\sqrt{B_2})=a.
     \nonumber
    %  \label{constraint:integral_right}
    \end{align*}
    Similarly, we have
    \begin{align}
     \widetilde{C_1}\int_{\delta_{-}}^0\cos^2\left(\frac{\sqrt{B_1}}{2}(x-c_1)\right) \, dt = -\frac{\widetilde{C_1}\delta_{-}}{2} + \frac{\widetilde{C_1}}{2\sqrt{B_1}}\sin(-c_1\sqrt{B_1})=1-a.\nonumber
    % \label{constraint:integral_left}
    \end{align}
\end{enumerate}

Moreover, we compute Fisher information $\mathcal{J}(q)$ under its general form. When $\delta_{-} \le x \le 0$, we have
\begin{align}
    \frac{\{q'(x)\}^2}{q(x)} &= \frac{B_1\widetilde{C_1}^2\cos^2\left(\frac{\sqrt{B_1}}{2}(x-c_1)\right)\sin^2\left(\frac{\sqrt{B_1}}{2}(x-c_1)\right)}{\widetilde{C_1}\cos^2\left(\frac{\sqrt{B_1}}{2}(x-c_1)\right)}\nonumber= B_1\widetilde{C_1}\sin^2\left(\frac{\sqrt{B_1}}{2}(x-c_1)\right)\nonumber.
\end{align}
On the other hand, we have for $0 \le x \le \delta_{+}$, 
\begin{align}
    \frac{\{q'(x)\}^2}{q(x)} &= \frac{B_2\widetilde{C_2}^2\cos^2\left(\frac{\sqrt{B_2}}{2}(x-c_2)\right)\sin^2\left(\frac{\sqrt{B_2}}{2}(x-c_2)\right)}{\widetilde{C_2}\cos^2\left(\frac{\sqrt{B_2}}{2}(x-c_2)\right)}\nonumber= B_2\widetilde{C_2}\sin^2\left(\frac{\sqrt{B_2}}{2}(x-c_2)\right)\nonumber.
\end{align}
Finally, we obtain that 
\begin{align}
    \mathcal{J}(q) &= B_1\widetilde{C_1}\int_{\delta_{-}}^0  \sin^2\left(\frac{\sqrt{B_1}}{2}(x-c_1)\right)\, dx + B_2\widetilde{C_2}\int_0^{\delta_{+}} \sin^2\left(\frac{\sqrt{B_2}}{2}(x-c_2)\right)\, dx \nonumber \\
    &=-\frac{B_1\widetilde{C_1}}{2}\delta_{-} - \frac{\sqrt{B_1}\widetilde{C_1}}{2}\sin(-\sqrt{B_1}c_1)+\frac{B_2\widetilde{C_2}}{2}\delta_{+} + \frac{\sqrt{B_2}\widetilde{C_2}}{2}\sin(-\sqrt{B_2}c_2)\nonumber.
\end{align}
Since there are eight variables: $B_1, B_2, \widetilde{C_1}, \widetilde{C_2}, c_1, c_2, \delta_-$ and $\delta_+$, the initial value problem is under-specified. We thus focus on a special case when $B_1=B_2$, $\widetilde{C_1}=\widetilde{C_2}$ and $c_1=c_2$. This improves constant compared to the case when $q$ is a cosine prior over $[0,1]$; however, it may not be sharpest. In addition to the following case, one can analyze the constant when $g(0)=0$ or $g'(0)=0$. Although we do not include such analysis, nether case provides a better constant than the cosine prior over $[0,1]$. 

We denote by $B=B_1=B_2$, $\widetilde{C} = \widetilde{C_1}=\widetilde{C_2}$ and $c=c_1=c_2$. The initial value problem then becomes
\begin{align}
    &\sqrt{B}(\delta_{-}-c)=\pm (2n_1+1)\pi\nonumber\\
    &\sqrt{B}(\delta_{+}-c)=\pm (2n_2+1)\pi\nonumber\\
    &\frac{\widetilde{C}\delta_{+}}{2} - \frac{\widetilde{C}}{2\sqrt{B}}\sin(-c\sqrt{B})=a     \label{constraint:integral_right}
\\
    &-\frac{\widetilde{C}\delta_{-}}{2} + \frac{\widetilde{C}}{2\sqrt{B}}\sin(-c\sqrt{B})=1-a.    \label{constraint:integral_left}
\end{align}
Thus we have
\begin{align}
    \widetilde{C}=\frac{2}{\delta_{+}-\delta_{-}},\, \sqrt{B}=\frac{2\pi}{\delta_{+}-\delta_{-}}\, \text{ and }\, c = \frac{\delta_{+}+\delta_{-}}{2}\nonumber.
\end{align}
Plugging them into \eqref{constraint:integral_right} and \eqref{constraint:integral_left}, we obtain
\begin{align}
 \frac{\delta_{+}}{\delta_{+}-\delta_{-}} - \frac{\sin(-c\sqrt{B})}{(\delta_{+}-\delta_{-})\sqrt{B}}=a \implies \frac{\delta_{+}}{\delta_{+}-\delta_{-}} - \frac{\sin\left(-\pi\frac{\delta_{+}+\delta_{-}}{\delta_{+}-\delta_{-}}\right)}{2\pi}=a\nonumber\\
  -\frac{\delta_{-}}{\delta_{+}-\delta_{-}} + \frac{\sin(-c\sqrt{B})}{(\delta_{+}-\delta_{-})\sqrt{B}}=1-a \implies -\frac{\delta_{-}}{\delta_{+}-\delta_{-}} + \frac{\sin\left(-\pi\frac{\delta_{+}+\delta_{-}}{\delta_{+}-\delta_{-}}\right)}{2\pi}=1-a\nonumber.
\end{align}
Finally, the difference of above displays implies
\begin{align}
 \frac{\delta_{+}+\delta_{-}}{\delta_{+}-\delta_{-}} - \frac{\sin\left(-\pi\frac{\delta_{+}+\delta_{-}}{\delta_{+}-\delta_{-}}\right)}{\pi}=2a-1\label{eq:last_constraint}.
\end{align}
Moreover, Fisher information $\mathcal{J}(q)$ is given by 
\begin{align}
    \mathcal{J}(q) 
    &=-\frac{B\widetilde{C}}{2}\delta_{-} - \frac{\sqrt{B}\widetilde{C}}{2}\sin(-\sqrt{B}c)+\frac{B\widetilde{C}}{2}\delta_{+} + \frac{\sqrt{B}\widetilde{C}}{2}\sin(-\sqrt{B}c)
    =\left(\frac{2\pi}{\delta_{+}-\delta_{-}}\right)^2\nonumber.
\end{align}

For each $a$, we hope to maximize $\delta_{+}-\delta_{-}$ subject to the equation \eqref{eq:last_constraint}. Letting $v = \frac{\delta_{+}+\delta_{-}}{\delta_{+}-\delta_{-}}$, the equation \eqref{eq:last_constraint} becomes 
\begin{align*}
    t -\sin(-\pi t)/\pi = 2a-1.
\end{align*}
Then solve for $\delta_{+}-\delta_{-}$ by 
\begin{align*}
    &\frac{\delta_{+}+\delta_{-}}{\delta_{+}-\delta_{-}} = t \Longleftrightarrow\frac{2\delta_{+}}{\delta_{+}-\delta_{-}} = t+1 \Longleftrightarrow 2\delta_{+} = (t+1)\delta_{+}-(t+1)\delta_{-} \Longleftrightarrow (1-t)\delta_{+} = -(t+1)\delta_{-}.
    % \\
    % &\qquad \Longleftrightarrow \frac{1-v}{v+1}\delta_{+} = -\delta_{-}
\end{align*}
Hence we have $\delta_{+}-\delta_{-}=\frac{2}{t+1}\delta_{+}$ or $\delta_{+}-\delta_{-}=-\frac{2}{1-t}\delta_-$. When $a>1/2$, we have $t > 0$ and thus $\delta_{+}+\delta_{-} > 0$. We can thus maximize $\delta_{+}-\delta_{-}$ by letting $\delta_{+}=1$ and we obtain $\mathcal{J}(q)=\left(2\pi/\frac{2}{t+1}\right)^2=\pi^2(1+t)^2$. Similarly when $a<1/2$, we have $t<0$. We can then maximize $\delta_{+}-\delta_{-}$ by letting $\delta_{-}=-1$ and we obtain $\mathcal{J}(q)=\left(2\pi/\frac{2}{1-t}\right)^2=\pi^2(1-t)^2$.

Putting together, we conclude that 
\begin{align*}
    \sup_q \frac{\left(\int_0^1q(t)\, dt\right)^2}{\mathcal{J}(q)/c^2+1/\sigma^2} \ge \sup_{a \in [0,1]} \frac{a^2}{\{\pi(1+|\eta^{-1}(2a-1)|)\}^2/c^2+1/\sigma^2}
\end{align*}
where $\eta(t) = t -\sin(-\pi t)/\pi$.
% \begin{align*}
%     \delta_+-\delta_- = \begin{cases}
%     \frac{2}{v+1}\delta_+\\
%     -\frac{2}{1-v}\delta_-
%     \end{cases}
% \end{align*}
% Then $\delta_{+}  -\delta_{-} = \delta_{+}+\frac{1-v}{v+1}\delta_{+} =\frac{2}{v+1}\delta_{+}$. This suggests we can take $\delta_+=1$. When $a < 0.5$, we take $\delta_{-}=-1$
% }
\end{proof}
\clearpage

 \subsection{The local risk of the pre-test estimator}
Consider the estimator of the form 
\begin{align*}
    S_n = \begin{cases}
    \tau &\text{ if } \overline{X}_n < r_n\\
    \overline{X}_n&\text{ otherwise } 
    \end{cases}
\end{align*}
A notable example is Hodges' estimator where $\tau=0$ and $r_n = n^{-1/4}$.
\begin{proof}
When $\mu_0 = 0$, we have 
\begin{align*}
    \sup_{|\mu - \mu_0| < cn^{-1/2}}\E_\mu \left|S_n - \psi(\mu)\right|^2 &= \max\left(\sup_{-cn^{-1/2} < \mu \le 0 }\left|S_n - \psi(\mu)\right|^2, \, \sup_{0 \le\mu < cn^{-1/2} }\left|S_n - \psi(\mu)\right|^2\right)
\end{align*}
For the first term, we observe that 
\begin{align*}
    \sup_{-cn^{-1/2} < \mu \le 0 }\E_\mu\left|S_n - \psi(\mu)\right|^2 
    &= \sup_{-cn^{-1/2} < \mu \le 0 }\left\{\E_\mu \overline{X}_n^{2\alpha} I(\overline{X}_n \ge r_n)+\E_\mu \tau^{2\alpha} I(\overline{X}_n < r_n)\right\}\\
    &= \sup_{-c/\sigma < \eta \le 0 }\frac{\sigma^{2\alpha}}{n^{\alpha}}\left\{\E_\mu (Z+\eta)^{2\alpha} I\left(Z \ge \frac{n^{1/2}}{\sigma}r_n-\eta\right)+\frac{n^\alpha\tau^{2\alpha}}{\sigma^{2\alpha}}P\left(Z < \frac{n^{1/2}}{\sigma}r_n-\eta\right)  \right\}
\end{align*}
where $Z:=\frac{n^{1/2}(\overline{X}_n-\mu)}{\sigma}$ and $\eta = \frac{n^{1/2}\mu}{\sigma}$. In particular $Z$ is standardized sample mean and follows a Gaussian distribution $N(0,1)$. Let $\phi$ be a density function for $N(0,1)$. Then for any $-c/\sigma < \eta \le 0$, it follows that 
\begin{align*}
    \E (Z+\eta)^{2\alpha} I(Z\ge -\eta) &= \int_{-\eta}^\infty (z+\eta)^{2\alpha}\phi(z)\, dz\le  \int_{-\eta}^\infty (z+\eta)^{2\alpha}\phi(z+\eta)\, dz=  \int_{0}^\infty z'^{2\alpha}\phi(z')\, dz'.
\end{align*}
The middle inequality follows since the density $\phi(z)$ is non-increasing on $0 \le z$. This implies that $\phi(z) \le \phi(z+\eta)$ since $\eta \le 0$ and $0 \le z+\eta$. The last quantity is equivalent to $\E Z^{2\alpha} I(Z\ge 0)$ and hence the risk of the estimator for any  $-c/\sigma \le \eta \le 0$ is upper bounded by the case when $\eta = 0$, or equivalently, when $\mu = 0$. This implies that 
\begin{align*}
    \sup_{-cn^{-1/2} < \mu \le 0 }\left|S_n - \psi(\mu)\right|^2 \le \left|S_n - \psi(0)\right|^2\le  \sup_{0 \le\mu < cn^{-1/2} }\left|S_n - \psi(\mu)\right|^2
\end{align*}
and the maximum is attained by some $\mu$ for $0 \le\mu < cn^{-1/2}$. For this case, we have
\begin{align*}
    \sup_{0 \le\mu < cn^{-1/2} }\left|S_n - \psi(\mu)\right|^2 
    &= \sup_{0 \le\mu < cn^{-1/2} }\left\{\E \left(\overline{X}_n^{\alpha}-\mu^{\alpha}\right)^2 I(\overline{X}_n \ge 0) + \E_\mu \mu^{2\alpha} I(\overline{X}_n < 0)\right\} \\
    & = \sup_{0 \le\eta < c/\sigma }\frac{\sigma^{2\alpha}}{n^\alpha}\left\{\E\left((Z+\eta)^{\alpha}-\eta^{\alpha}\right)^2 I(Z \ge -\eta) + \E \eta^{2\alpha} I(Z < -\eta)\right\}
\end{align*}

\end{proof}
