# Supplementary material for: Generalized van Trees inequality: Local minimax bounds for non-smooth functionals and irregular statistical models
Source: arXiv:2405.06437 source file (2024-10-19)
Supplement: Supplementary file 8 [file unif.tex]

\clearpage
\section{The minimax lower bounds for estimating the parameter of uniform distribution}
Given $n$ IID observations, the squared Hellinger distance has the following property: 
\begin{align*}
    H^2(P^n_{\theta_0}, P^n_{\theta_0+h}) &=2-2\left(1-\frac{H^2(P_{\theta_0}, P_{\theta_0+h})}{2}\right)^n.
\end{align*}
We consider $H^2(P_{\theta_0}, P_{\theta_0+h})$ where $P_\theta$ corresponds to the uniform distribution with support over $[0, \theta]$. We now consider two cases. When $h>0$, we have
\begin{align*}
    H^2(P_{\theta_0}, P_{\theta_0+h}) &= \int_0^{\theta_0}\left(\theta_0^{-1/2}-(\theta_0+h)^{-1/2}\right)^2\,dx + \int_{\theta_0}^{\theta_0 +h}(\theta_0+h)^{-1}\,dx \\
    &= 1-2\theta_0/\sqrt{\theta_0(\theta_0+h)}+\theta_0/(\theta_0+h)+h/(\theta_0+h) \\
    &= 2-\frac{2}{\sqrt{1+h/\theta_0}}\\
    &= 2\left(1-(1+h/\theta_0)^{-1/2}\right).
\end{align*}
Similarly when $h<0$, we have
\begin{align*}
    H^2(P_{\theta_0}, P_{\theta_0+h}) &= \int_0^{\theta_0+h}\left(\theta_0^{-1/2}-(\theta_0+h)^{-1/2}\right)^2\,dx + \int_{\theta_0+h}^{\theta_0}\theta_0^{-1}\,dx \\
    &= (\theta_0+h)/\theta_0 - 2(\theta_0+h)/\sqrt{\theta_0(\theta_0+h)}+1+1-(\theta_0+h)/\theta_0 \\
    &= 2-\frac{2(1+h/\theta_0)}{\sqrt{1+h/\theta_0}}\\
    &= 2\left(1-(1+h/\theta_0)^{1/2}\right).
\end{align*}
Then we have 
\begin{align*}
     H^2(P^n_{\theta_0}, P^n_{\theta_0+h}) &= 2-2(1+h/\theta_0)^{-n/2}
\end{align*}
when $h > 0$ and 
\begin{align*}
     H^2(P^n_{\theta_0}, P^n_{\theta_0+h}) &= 2-2(1+h/\theta_0)^{n/2}
\end{align*}
when $h < 0$. 

Consider a random variable $\vartheta \in [\theta_0 - \delta, \theta_0+\delta]$. Let $q_{\theta_0, \delta}$ be the density for $\vartheta$. Then our lower bound implies
\begin{align*}
    &\max\left( \int_{\Theta^{(-\delta)}}\E_\theta\left(T(x)-\psi(\theta)\right)^2q_{\theta_0, \delta}(\theta) \, d\theta,\, \int_{\Theta^{(-\delta)}}\E_\theta\left(T(x)-\psi(\theta)\right)^2q_{\theta_0, \delta}(\theta+h) \, d\theta\right)\\
    &\qquad \ge \frac{h^2}{4\left\{H^2(Q_h, Q) +\int_{\Theta} q_{\theta_0, \delta}^{1/2}(\theta+h)q_{\theta_0, \delta}^{1/2}(\theta)H^2(P_{\theta+h}, P_{\theta})\,d\theta\right\}}\\
    &\qquad \ge\frac{h^2}{4\left\{H^2(Q_h, Q) +\int_{\Theta} q_{\theta_0, \delta}^{1/2}(\theta+h)q_{\theta_0, \delta}^{1/2}(\theta)\{2-2(1+h/\theta)^{-n/2}\}\,d\theta\right\}}
\end{align*}
We first let $h \to 0$ while $\delta$ fixed. First, the left-hand side can be bounded by 
\[\lim_{h\to0}\max\left( \int_{\Theta^{(-\delta)}}\E_\theta\left(T(x)-\theta\right)^2q_{\theta_0, \delta}(\theta) \, d\theta,\, \int_{\Theta^{(-\delta)}}\E_\theta\left(T(x)-\theta\right)^2q_{\theta_0, \delta}(\theta+h) \, d\theta\right) \le \sup_{\theta: |\theta-\theta_0| < \delta} \E_\theta\left(T(x)-\theta\right)^2.\]
This corresponds to the left-hand side of \cite{korostelev2011mathematical}. 
\begin{align*}
    \lim_{h\to 0}\int_{\Theta} q_{\theta_0, \delta}^{1/2}(\theta+h)q_{\theta_0, \delta}^{1/2}(\theta)\{2-2(1+h/\theta)^{-n/2}\}\,d\theta &= \lim_{h\to 0}2\int_{\Theta} q_{\theta_0, \delta}(\theta)\{1-(1+h/\theta)^{-n/2}\}\,d\theta
\end{align*}
\kt{From here we want to show that the constant is $\theta_0^2$. I tried with uniform prior since this bound does not require $q$ to be absolutely continuous, but did not work.}

Let $q_{\theta_0, \delta}(t) = 1/(2\delta)$. Then 
\[H^2(Q_h, Q) = \frac{2h}{2\delta}\]
\[2\int_{\Theta} q_{\theta_0, \delta}(\theta)\{1-(1+h/\theta)^{-n/2}\}\,d\theta = \frac{1}{\delta} \int_{\theta_0-\delta}^{\theta_0+\delta}1-(1+h/\theta)^{-n/2}\,d\theta \approx \frac{1}{2\delta} \int_{\theta_0-\delta}^{\theta_0+\delta}\frac{hn}{\theta}\,d\theta = \frac{nh}{2\delta} [\log(\theta_0+\delta)-\log(\theta_0-\delta) ]\]
(The approximation is by the first order Taylor expansion, which is still crude since I just wanted to see if this approach works). 
{\color{blue} If $h = c_0/n$, then
\[
\frac{1}{\delta}\int_{\theta_0 - \delta}^{\theta_0 + \delta} 1 - (1+h/\theta)^{n/2}d\theta \approx \frac{1}{\delta}\int_{\theta_0 - \delta}^{\theta_0 + \delta} 1-e^{c_0/(2\theta)}d\theta,
\]
this approximation is obtained by taking the limit as $n\to\infty$ inside the integral.}
Then if we let $h = c_0/n$ and $n\to\infty$, we get
\[\liminf_{n\to\infty}\sup_{\theta: |\theta-\theta_0| < \delta} \E_\theta n^2\left(T(x)-\theta\right)^2 \ge \liminf_{n\to\infty}\frac{c_0^2}{4\frac{c_0}{n\delta} + 4c_0\frac{\log(\theta_0+\delta)-\log(\theta_0-\delta)}{2\delta}} = \frac{c_0}{4\frac{\log(\theta_0+\delta)-\log(\theta_0-\delta)}{2\delta}}\]
Finally, if we let $\delta \to 0$, we get $\frac{c_0\theta_0}{4}$. 
\kt{I think I made a mistake again somewhere I take the order of limit.} {\color{blue}If you think you did something wrong because you are not getting $\theta_0^2$, this is because $c_0$ has an additional $\theta_0$. But it seems there is something wrong going on because the approximation you are using for exponential to linear function does not work because $hn/(2\theta)$ is, in fact, an $O(1)$ quantity, not $o(1)$. See my approximation above which is valid as $n\to\infty$.}

\kt{Using fundamental theorem of calculus,
\begin{align*}
    \lim_{\delta\to0}\liminf_{n\to\infty}\sup_{\theta: |\theta-\theta_0| < \delta} \E_\theta n^2\left(T(x)-\theta\right)^2 &\ge \lim_{\delta\to0}\liminf_{n\to\infty} \frac{c_0^2}{4\frac{c_0}{n\delta} + 4\frac{1}{2\delta}\int_{\theta_0 - \delta}^{\theta_0 + \delta} 2(1-e^{-c_0/(2\theta)})d\theta} \\
    &=\lim_{\delta\to0}\frac{c_0^2}{4\frac{1}{2\delta}\int_{\theta_0 - \delta}^{\theta_0 + \delta} 2(1-e^{-c_0/(2\theta)})d\theta} \\
    &= \frac{c_0^2}{8(1-e^{-c_0/(2\theta_0)})}
\end{align*}
}
At this point, $c_0$ is not a free parameter. Note that $h$ and $\delta$ are related. You should not take the limit as $\delta \to 0$ before figuring out this relation.

\newpage
\kt{New attempt. Let $\delta_n = a/n$ and $h_n = b/n$. Assume $a$ and $b$ satisfy $(a+b)/n < \delta$ and take the limit $n \to \infty$}
The left-hand side can be bounded by 
\[\max\left( \int_{\Theta^{(-\delta_n)}}\E_\theta\left(T(x)-\theta\right)^2q_{\theta_0, \delta_n}(\theta) \, d\theta,\, \int_{\Theta^{(-\delta_n)}}\E_\theta\left(T(x)-\theta\right)^2q_{\theta_0, \delta_n}(\theta+h_n) \, d\theta\right) \le \sup_{\theta: |\theta-\theta_0| < \delta_n+h_n} \E_\theta\left(T(x)-\theta\right)^2.\]
Similarly, consider the uniform prior, $q_{\theta_0, \delta}(t) = 1/(2\delta)$ \kt{Maybe there is a better prior?}. Then 
\[H^2(Q_{h_n}, Q) = \frac{2h_n}{2\delta_n} = b/a.\]
For the second term we have 
\begin{align*}
    \int_{\Theta} q_{\theta_0, \delta_n}^{1/2}(\theta+h_n)q_{\theta_0, \delta_n}^{1/2}(\theta)\{2-2(1+h/\theta)^{-n/2}\}\,d\theta = \frac{1}{2\delta_n}\int_{\theta_0-\delta_n}^{\theta_0+\delta_n-h_n} \{2-2(1+h_n/\theta)^{-n/2}\}\,d\theta 
\end{align*}
assuming $h_n > 0$.
\begin{align*}
    \frac{n}{2a}\int_{\theta_0-a/n}^{\theta_0+a/n-b/n} \{2-2(1+\tfrac{b}{n\theta})^{-n/2}\}\,d\theta 
\end{align*}

Plugging in everything, we get
\begin{align*}
    &\sup_{\theta: |\theta-\theta_0| < \delta_n+h_n} \E_\theta\left(T(x)-\theta\right)^2 \ge \frac{b^2}{n^2\left\{\tfrac{4b}{a} + \frac{4n}{2a}\int_{\theta_0-a/n}^{\theta_0+a/n-b/n} \{2-2(1+\tfrac{b}{n\theta})^{-n/2}\}\,d\theta \right\}}\\
    &\qquad \implies \sup_{\theta: |\theta-\theta_0| < \delta_n+h_n} n^2 \E_\theta\left(T(x)-\theta\right)^2 \ge \frac{b^2}{\tfrac{4b}{a} + \frac{4n}{2a}\int_{\theta_0-a/n}^{\theta_0+a/n-b/n} \{2-2(1+\tfrac{b}{n\theta})^{-n/2}\}\,d\theta } 
\end{align*}
The right-hand-side can further be lower bounded by \kt{possibly losing something here...}
\begin{align*}
    \frac{b^2}{\tfrac{4b}{a} + \frac{4n}{2a}\int_{\theta_0-a/n}^{\theta_0+a/n-b/n} \{2-2(1+\tfrac{b}{n\theta})^{-n/2}\}\,d\theta } & \ge 
    \frac{b^2}{\tfrac{4b}{a} + \frac{4n}{2a}\int_{\theta_0-a/n}^{\theta_0+a/n} \{2-2(1+\tfrac{b}{n\theta})^{-n/2}\}\,d\theta }
\end{align*}
since $b > 0$. Now taking the limit as $n \to \infty$, we get
\begin{align*}
    \lim_{n\to \infty} \frac{b^2}{\tfrac{4b}{a} + \frac{4n}{2a}\int_{\theta_0-a/n}^{\theta_0+a/n} \{2-2(1+\tfrac{b}{n\theta})^{-n/2}\}\,d\theta} &= \frac{b^2}{\tfrac{4b}{a} + 4\left(2-2\exp(-b/2\theta_0)\right)}
\end{align*}
\kt{From here, I solve the optimization on wolframalpha with contraint $a+b \le 1; b \ge 0$. I did not get the right constant.}

\clearpage
\kt{Another attempt}
Following \ref{as:IPBorder}, let $\Theta = [\theta_0 - \gamma, \theta_0 + \gamma]$ for fixed $\gamma > 0$ and apply our bound. Suppose $q$ has the support over $\Theta = [\theta_0 - \gamma + 2\delta, \theta_0 + \gamma- 2\delta]$ and $h < \delta$, {\color{red}and $\delta < \gamma/2$} we get
\[\sup_{\theta: |\theta_0 -\theta| < \gamma} E_\theta \{T(x) - \theta\}^2 \ge \frac{h^2}{4\left\{H^2(Q_h, Q) +\int_{\Theta} q^{1/2}(\theta+h)q^{1/2}(\theta)H^2(P^n_{\theta+h}, P^n_{\theta})\,d\theta\right\}}\]
Let $h = c/n$ and $n$ large enough such that 
\[2h < 2\delta < \gamma \implies c < \gamma n/2\]
Let $q$ be some location-scaling family of $q^*$ such that 
\[q(t) = \frac{1}{\gamma - 2\delta}q^*\left(\frac{t-\theta_0}{\gamma-2\delta}\right)\]
and $\supp(q^*) = [-1,1]$. We have $\mathcal{J}(Q) = \frac{1}{(\gamma-2\delta)^2}\mathcal{J}(Q^*)$

\begin{align*}
    &\frac{h^2}{4\left\{H^2(Q_h, Q) +\int_{\Theta} q^{1/2}(\theta+h)q^{1/2}(\theta)H^2(P^n_{\theta+h}, P^n_{\theta})\,d\theta\right\}} \\
    &\qquad = \frac{c^2}{4n^2\left\{H^2(Q_{c/n}, Q) +\int_{\theta_0 - \gamma - 2\delta}^{\theta_0 + \gamma - 2\delta} q^{1/2}(\theta+c/n)q^{1/2}(\theta)(1+\frac{c}{n\theta})^{-n/2}\,d\theta\right\}}\\
    &\qquad \ge \frac{c^2}{4n^2\left\{H^2(Q_{c/n}, Q) +\left(1+\frac{c}{n(\theta_0-\gamma)}\right)^{-n/2}\int_{\theta_0 - \gamma - 2\delta}^{\theta_0 + \gamma - 2\delta} q^{1/2}(\theta+c/n)q^{1/2}(\theta)\,d\theta\right\}} &&(\kt{Can be improved?})\\
    &\qquad = \frac{c^2}{4n^2\left[H^2(Q_{c/n}, Q) +\left(1+\frac{c}{n(\theta_0-\gamma)}\right)^{-n/2}\left\{1-\frac{1}{2}H^2(Q_{c/n}, Q)\right\}\right]}\\
    &\qquad = \frac{c^2}{4n^2\left[\left\{1-\frac{1}{2}\left(1+\frac{c}{n(\theta_0-\gamma)}\right)^{-n/2}\right\}H^2(Q_{c/n}, Q) +\left(1+\frac{c}{n(\theta_0-\gamma)}\right)^{-n/2}\right]} 
\end{align*}
If we move $n^2$ and use $(1+x/n)^{n} \approx \exp(x)$ as $n \to \infty$ and the limit of $H^2(Q_{c/n}, Q)$, 
\begin{align*}
    \liminf_{n\to \infty}\sup_{\theta: |\theta_0 -\theta| < \gamma} n^2E_\theta \{T(x) - \theta\}^2 &\ge \liminf_{n\to \infty}\frac{c^2}{4\left[\left\{1-\frac{1}{2}\exp\left(-\frac{c}{2(\theta_0-\gamma)}\right)\right\}\frac{c^2}{4n^2}\frac{1}{(\gamma-2\delta)^2}\mathcal{J}(Q^*) +\exp\left(-\frac{c}{2(\theta_0-\gamma)}\right)\right]}\\
    &=\frac{c^2}{4\exp\left(-\frac{c}{2(\theta_0-\gamma)}\right)}
\end{align*}
\kt{Why does $c$ appear in the numerator?}
\clearpage
\kt{Update from our discussion on the February 1st}. 
\begin{align}
    h^2 & \le \left\{\E_{\mathcal{X}, \Theta} \left(\sqrt{\frac{\gamma_h(x,t)}{\gamma_0(x,t)}}+1\right)^2 \left(T(x)-t\right)^2 \right\}\E_{\mathcal{X}, \Theta} \left(\sqrt{\frac{\gamma_h(x,t)}{\gamma_0(x,t)}}-1\right)^2\nonumber \\
    &\le \left\{\E_{\mathcal{X}, \Theta} \left(\sqrt{\frac{\gamma_h(x,t)}{\gamma_0(x,t)}}+1\right)^2 \left(T(x)-t\right)^2 \right\}H^2\left(\Gamma_h,\Gamma_0\right)\nonumber \\
    &\le 2\left\{\int_\Theta \E_{t} \left(T(x)-t\right)^2 q(t)\, dt + \int_\Theta \E_{t+h} \left(T(x)-t\right)^2 q(t+h)\, dt\right\}H^2\left(\Gamma_h,\Gamma_0\right)\nonumber 
\end{align}
\kt{I think the term in the bracket gives\[
2\max\left\{\sup_{t \in \Theta}\E_t (T(x)-t)^2, \sup_{\{u: u-h\in \Theta\}}\E_u (T(x)-u+h)^2\right\}
\]}
Similar to \cite{korostelev2011mathematical}, we consider uniform prior over $[\theta_0, \theta_0 + b/n]$. Then we have the following items:
\begin{enumerate}
    \item $q(t) := I(\theta_0 \le t \le \theta_0+b/n) \frac{n}{b}$
    \item $q(t+h) := I(\theta_0 \le t+h \le \theta_0+b/n) \frac{n}{b}$
    \item $p^n(x; t) := I(0 \le \min x, \max x \le t) \frac{1}{t^n}$
    \item $p^n(x; t+h) := I(0 \le \min x, \max x \le t+h) \frac{1}{(t+h)^n}$
\end{enumerate}
Now we evaluate $H^2(\Gamma_h,\Gamma_0)$. 
\begin{align*}
    &H^2(\Gamma_h,\Gamma_0) \\
    &\qquad = 2-2\iint_{\mathcal{X}, \Theta}I(\theta_0 \le t \le \theta_0+b/n)I(\theta_0 \le t+h \le \theta_0+b/n)\frac{n}{b}\\
    &\qquad\qquad I(0 \le \min x, \max x \le t)I(0 \le \min x, \max x \le t+h)\frac{1}{t^{n/2}}\frac{1}{(t+h)^{n/2}}\, dx^n \, dt\\
    &\qquad = 2-2\int_{\theta_0}^{\theta_0+b/n-h}\int_0^t \frac{n}{b}\frac{1}{t^{n/2}}\frac{1}{(t+h)^{n/2}}\, dx^n \, dt \\
    &\qquad = 2-2\frac{n}{b}\int_{\theta_0}^{\theta_0+b/n-h} \frac{t^n}{t^{n/2}(t+h)^{n/2}} \, dt\\
    &\qquad = 2-2\frac{n}{b}\int_{\theta_0}^{\theta_0+b/n-h} (1+h/t)^{-n/2} \, dt \\
    & \qquad \le 2-2 (1+h/\theta_0)^{-n/2} \left(1-\frac{nh}{b}\right)
\end{align*}

From here, we may let $h = c/n$ where $ 0 < c < b$. Then we have 
\begin{align*}
    H^2(\Gamma_{c/n},\Gamma_0) &\le 2-2 (1+c/n\theta_0)^{-n/2} \left(1-\frac{c}{b}\right)
\end{align*}

Taking the log of the second component, we get
\begin{align*}
    \log\left\{-2 (1+c/n\theta_0)^{-n/2} \left(1-\frac{c}{b}\right)\right\} &= \log(-2)-\frac{n}{2}\log(1+c/n\theta_0)+\log\left(1-\frac{c}{b}\right) = \eta(c)
\end{align*}
\begin{align*}
    \frac{d}{dc}\eta(c) = -\frac{n}{2}\frac{1/n\theta_0}{1+c/n\theta_0} + \frac{-1/b}{1-c/b} = -\frac{n}{2n\theta_0 + 2c}-\frac{1}{b-c}
\end{align*}
\begin{align*}
    \frac{d^2}{dc^2}\eta(c) = \frac{2n}{(2n\theta_0 + 2c)^2}-\frac{1}{(b-c)^2}
\end{align*}
\begin{align*}
    \frac{d}{dc}\eta(c) \bigg|_{c=c^*}= 0 &\implies 
    -\frac{n}{2n\theta_0 + 2c^*}=\frac{1}{b-c^*}\\
    &\implies n(b-c^*) = -2n\theta_0 - 2c^*\\
    &\implies 2c^*-nc^* = -nb-2n\theta_0 \\
    &\implies c^* = (b+2\theta_0)/(1-2/n)
\end{align*}
Since we restrict $c < b$ and the last term is greater than $b$ as $n \to \infty$, the optimal is attained as $c \to b$. 

\begin{align*}
    \log\left(\frac{c^2/n^2}{-2(1+c/n\theta_0)^{-n/2} \left(1-\frac{c}{b}\right)}\right) = 2\log(c/n)-\log(-2)+\frac{n}{2}\log(1+c/n\theta_0)-\log\left(1-\frac{c}{b}\right)
\end{align*}

Taking derivative wrt $c$, 
\begin{align*}
    \frac{2}{c}+\frac{n}{2n\theta_0 + 2c}+\frac{1}{b-c}
\end{align*}

The second derivative is 
\begin{align*}
    -\frac{2}{c^2}-\frac{2n}{(2n\theta_0 + 2c)^2}+\frac{1}{(b-c)^2}
\end{align*}

\begin{align*}
    \frac{2}{c}+\frac{n}{2n\theta_0 + 2c}+\frac{1}{b-c} = \frac{n}{2n\theta_0 + 2c}+\frac{2(b-c)+c}{c(b-c)}= \frac{n}{2n\theta_0 + 2c}+\frac{2b-c}{c(b-c)}
\end{align*}

\clearpage
\kt{New development}
First, we start with \cite{ibragimov1981statistical, lin2019optimal} and others where minimax risk is lower bounded by the sum of risk at two points. When $0 < h < \delta$, we have
\begin{align*}
    H^2(P^n_{\theta_0}, P^n_{\theta_0+h}) &= 2\left(1-(1+h/\theta_0)^{-n/2}\right).
\end{align*}
Take $h = b/n$ such that $b < \delta n$. Then as $n \to \infty$, 
\begin{align*}
    H^2(P^n_{\theta_0}, P^n_{\theta_0+h}) &\approx 2\left(1-(1+h/\theta_0)^{-n/2}\right) = 2-2\exp\left(-\frac{b}{2\theta_0}\right).
\end{align*}

Consier the modulus of continuity i.e., $\{h : H^2(P^n_{\theta_0}, P^n_{\theta_0+h}) \le \rho\}$ for $\rho < 1$. Then 
\begin{align*}
    2-2\exp\left(-\frac{b}{2\theta_0}\right) \le \rho &\implies 1-\rho/2 \le \exp\left(-\frac{b}{2\theta_0}\right)\\
    &\implies \log\left(1-\rho/2\right) \le -\frac{b}{2\theta_0} 
    \\
    &\implies b  \le -2\theta_0 \log\left(1-\rho/2\right)
\end{align*}

\begin{align*}
    \frac{1}{2}\left\{E_{\theta + h}|T - \psi(\theta + h)|^2 + E_{\theta}|T - \psi(\theta)|^2 \right\} &\ge  \sup_{\{h : H^2(P^n_{\theta_0}, P^n_{\theta_0+h}) \le \rho\}}\left(\frac{1 -\rho}{4}\right)_+h^2 \\
    &= \left(\frac{1 -\rho}{4}\right)_+\frac{4\theta_0^2 \log^2\left(1-\rho/2\right)}{n^2}
\end{align*}
We then optimize $(1 -\rho)\log^2\left(1-\rho/2\right)$ for $\rho$ over $0 \le \rho \le 1$. The minimax lower bound is $c\theta_0^2/n^2$ where $c$ is approximately $0.05$ according to wolfram alpha. This is better than the constant by \cite{lin2019optimal}, which is $1/576$ but both of them is far smaller than the sharp constant $1$. 

The benefit of van-trees is in the extension of above results to the distribution over local alternatives instead of two points. We thus need to compute the Hellinger distance such that it takes advantage of this.
\begin{align*}
    H^2(\Gamma^n_{\theta_0}, \Gamma^n_{\theta_0+h}) &= 2\int_{\theta_0}^{\theta_0+\delta-h}\left(1-(1+h/t)^{-n/2}\right)\, q^{1/2}(t)q^{1/2}(t+h)\, dt.
\end{align*}

\kt{New attempt}
\begin{align*}
    H^2(\Gamma^n_{\theta_0}, \Gamma^n_{\theta_0+h}) &= 2-2\int_{\theta_0-\gamma+2h}^{\theta_0+\gamma-3h}\frac{t^n}{t^{n/2}(t+h)^{n/2}}\, q^{1/2}(t)q^{1/2}(t+h)\, dt.
\end{align*}
where the minimax risk is over $|\theta_0 \pm \gamma|$ and the support of $q$ must be contained in $[\theta_0 - \gamma + 2h, \theta_0 + \gamma - 2h]$. We let $h=b/n$ and $\gamma  = c/n$. Then it immediately follows that $0 < \gamma < \theta_0 \implies 0< c < \theta_0 n$ and $0 < 2h < \gamma \implies 0 < b < c/2$.

Now take $q(t) \propto 1/t^n$. Since the support at least $[\theta_0 - \gamma + 2h, \theta_0 + \gamma - 2h]$, the normalizing constant is 
\begin{align*}
    C=\int_{\theta_0 - \gamma + 2h}^{\theta_0 + \gamma - 2h}  1/t^n \, dt = \frac{1}{n-1}\left((\theta_0-\gamma+2h)^{-(n+1)}-(\theta_0+\gamma-2h)^{-(n+1)}\right)
\end{align*}
We then obtain 
\begin{align*}
    H^2(\Gamma^n_{\theta_0}, \Gamma^n_{\theta_0+h}) &= 2-2/C\int_{\theta_0-\gamma+2h}^{\theta_0+\gamma-3h}\frac{t^n}{t^{n}(t+h)^{n}}\, dt \\ 
    &= 2-2/C\int_{\theta_0-(c-2b)/n}^{\theta_0+(c-3b)/n}(t+b/n)^{-n}\, dt \\
    &= 2-2/C \frac{1}{n-1}\left((\theta_0-c/n+3b/n)^{-(n+1)}-(\theta_0+c/n-2b/n)^{-(n+1)}\right)\\
    &= 2-2\frac{(\theta_0-c/n+3b/n)^{-(n+1)}-(\theta_0+c/n-2b/n)^{-(n+1)}}{(\theta_0-c/n+2b/n)^{-(n+1)}-(\theta_0+c/n-2b/n)^{-(n+1)}}\\
    &= 2-2\frac{(1-(c-3b)/(\theta_0n))^{-(n+1)}-(1+(c-2b)/(n\theta_0))^{-(n+1)}}{(\theta_0-c/n+2b/n)^{-(n+1)}-(\theta_0+c/n-2b/n)^{-(n+1)}}
\end{align*}
\kt{I thought I could make a Gamma function but realized we have $\exp(-1/x)$, not $\exp(-x)$}
