# Supplementary material for: Generalized van Trees inequality: Local minimax bounds for non-smooth functionals and irregular statistical models
Source: arXiv:2405.06437 source file (2024-10-19)
Supplement: Supplementary file 9 [file fisher-defect.tex]

\section{On Hellinger differentiability and the Fisher defect}
